# Supplementary material for: Optical Emission Line Nebulae in Galaxy Cluster Cores 1: The Morphological, Kinematic and Spectral Properties of the Sample
Source: arXiv:1603.03047 source file (2016-03-09)
Supplement: Supplementary file 1 [file appendix_r2.tex]

\begin{appendix}

%Appendix A--------------------------------------------------------------------------------
\clearpage
\onecolumn
%\thispagestyle{headings}
%\mbox{}
\section{Table 1. continued}
\label{app:tab1}

\begin{table}
\begin{center}
\scriptsize
\centerline{\sc Table 1.}
\centerline{\sc The observational parameters listed for each object in the VIMOS sample}
\smallskip
\begin{tabular}{c c c c c c c c c c c}
\hline
\noalign{\smallskip} 
Cluster & Redshift & Grating & Exposure & Mean & Lines  & RA & Dec & L$_x$ & T$_x$ & Classification \\ 
 & & & (s) & Seeing('') & Detected & & & (10$^{43}$\,erg\,s$^{-1}$) & (keV) & \\[0.5ex]
\hline
Abell 1060 & 0.01263 & HR-orange & 3$\times$600 & 0.79 &  &  10:36:42.78 &  -27:31:39.66 & 3.34 & 3.2 & Cluster \\
\noalign{\smallskip} 
Abell 1084 & 0.13301 & HR-red    & 3$\times$600 & 0.68 & [OI] &  10:44:32.69 &  -07:04:05.21  & 48.99 & 7.3 & Cluster \\
\noalign{\smallskip} 
Abell 11   & 0.14910 & HR-red    & 3$\times$600 & 0.77 & [OI], [SII] & 00:12:33.58 &  -16:28:05.17  & 18.2 & --- & Cluster \\
\noalign{\smallskip} 
Abell 1111 & 0.16518 & HR-red    & 3$\times$600 & 0.85 & [OI], [SII] & 10:50:36.26 &  -02:36:13.37  & 27.30 & --- & Cluster  \\
\noalign{\smallskip} 
Abell 1204 & 0.17057 & HR-red    & 3$\times$600 & 0.81 & [OI] &  11:13:20.08 &  17:35:37.88  & 72.6 & 3.78 & Cluster \\
\noalign{\smallskip} 
Abell 133  & 0.05665 & HR-orange & 3$\times$600 & 0.93 & [OI], [SII] &  01:02:41.49 &  -21:52:48.62 & 16.17 & 3.71 & Cluster \\
\noalign{\smallskip} 
Abell 1348 & 0.11985 & HR-orange & 3$\times$600 & 0.87 & H$\beta$, [OIII], &  11:41:24.12 &  -12:16:35.90  & 21.09 & 5.5 & Cluster   \\
 & & & & & [NI], [OI] & & & & & \\
\noalign{\smallskip} 
Abell 1663 & 0.08433 & HR-orange & 3$\times$600 & 2.46 & [OI], [SII] &  13:02:52.36 &  -02:30:55.93 & 8.04 & --- & Cluster \\
\noalign{\smallskip} 
Abell 1668 & 0.06355 & HR-orange & 3$\times$600 & 1.21 & [OIII], [SII] &  13:03:42.29 &  19:16:14.70  & 16.1 & 3.7 & Cluster  \\
\noalign{\smallskip} 
Abell 194  & 0.01820 & HR-orange & 3$\times$600 & 1.17 & [SII] &  01:25:44.08 &  -01:22:43.19 & 0.74 & 1.4 & Group$^1$ \\
\noalign{\smallskip} 
Abell 1991 & 0.05901 & HR-orange & 3$\times$600 & 0.68 & [OI], [SII] &  15:43:31.36 &  18:38:29.52 & 13.50 & 5.4 & Cluster \\
\noalign{\smallskip} 		
Abell 2052 & 0.03435 & HR-orange & 3$\times$600 & 1.89 & [OI], [SII] &  15:16:44.45 &  07:01:14.65  & 25.2 & 2.98 & Cluster  \\
\noalign{\smallskip} 
Abell 2390 & 0.23041 & HR-red    & 3$\times$600 & 1.41 & [NI], [OI], &  21:53:36.62 &  17:41:40.04  & 214.44 & 11.6 & Cluster  \\
 & & & & & [SII] & & & & & \\
\noalign{\smallskip} 
Abell 2415 & 0.05759 & HR-orange & 3$\times$600 & 1.51 & [OI], [SII] &  22:05:40.33 &  -05:35:32.36  & 12.07 & 3.8 & Cluster \\
\noalign{\smallskip} 
Abell 2495 & 0.07932 & HR-orange & 3$\times$600 & 0.92 & [SII] &  22:50:19.66 &  10:54:10.63 & 29.80 & 5.0 & Cluster \\	
\noalign{\smallskip} 	
Abell 2566 & 0.08301 & HR-orange & 3$\times$600 & 0.99 & H$\beta$, [OIII], &  23:16:07.26 &  -20:27:18.44  & 13.32 & 4.0 & Cluster \\
 & & & & & [OI], [SII] & & & & & \\
\noalign{\smallskip} 
Abell 2580 & 0.08811 & HR-orange & 2$\times$600 & 1.85 & [SII] &  23:21:26.24 &  -23:12:26.78 & 6.9 & --- & Cluster \\
\noalign{\smallskip} 
Abell 2734 & 0.06204 & HR-orange & 3$\times$600 & 1.81 & [OI], [SII] &  00:11:21.62 &  -28:51:12.82  & 11.97 & 4.5 & Cluster \\
\noalign{\smallskip} 
Abell 291  & 0.19603 & HR-red    & 3$\times$600 & 1.05 & [SII] &  02:01:42.90 &  -02:11:46.85 & 48.83 & --- & Cluster \\
\noalign{\smallskip} 
Abell 3017 & 0.21927 & HR-red    & 3$\times$600 & 1.39 & [OI],[SII] &  02:25:52.97 &  -41:54:51.94  & 124.2 & 9.1 & Cluster \\
\noalign{\smallskip} 
Abell 3112 & 0.07602 & HR-orange & 3$\times$600 & 2.25 & [OI], [SII] &  03:17:57.49 &  -44:14:15.70 & 42.43 & 4.28 & Cluster  \\	
\noalign{\smallskip} 	
Abell 3378 & 0.14132 & HR-red    & 3$\times$600 & 1.32 & [SII] &  06:05:53.70 &  -35:18:06.90 & 46.65 & 7.0 & Cluster \\	
\noalign{\smallskip} 	
Abell 3444 & 0.25550 & HR-red    & 3$\times$600 & 0.51 & [OI] &  10:23:49.94 &  -27:15:21.56 & 137.60 & 12.0 & Cluster \\	
\noalign{\smallskip} 	
Abell 3574 & 0.01409 & HR-orange & 3$\times$400 & 0.92 & [OI], [SII] &  13:47:24.31 &  -30:24:22.78 & 0.14 & --- & Group$^{1}$ \\
\noalign{\smallskip} 
Abell 3581 & 0.02160 & HR-orange & 3$\times$600 & 2.03 & [OI], [SII] &  14:07:27.88 &  -27:00:50.93 & 3.81 & 2.4 & Cluster \\
\noalign{\smallskip} 
Abell 3605 & 0.06430 & HR-orange & 3$\times$600 & 0.69 & [OI], [SII] &  14:35:06.73 &  -28:20:28.22 & 4.96 & --- & Cluster \\
\noalign{\smallskip} 
Abell 3638 & 0.07687 & HR-orange & 3$\times$600 & 1.04 & [OIII], [NI], &  19:25:29.39 &  -42:57:08.38 & 10.20 & 4.0 & Cluster \\
 & & & & & [OI], [SII] & & & & & \\
\noalign{\smallskip} 
Abell 3639 & 0.15051 & HR-red    & 3$\times$600 & 0.72 & [OI], [SII] &  19:28:12.66 &  -50:56:22.42 & 22.99 & --- & Cluster  \\	
\noalign{\smallskip} 	
Abell 3806 & 0.07460 & HR-orange & 3$\times$600 & 0.56 & [SII] &  21:46:22.30 &  -57:17:08.14 & 9.94 & 3.6 & Cluster\\
\noalign{\smallskip} 
Abell 383  & 0.18869 & HR-red    & 3$\times$600 & 1.28 & [OI], [SII] &  02:48:03.07 &  -03:31:42.72 & 45.59 & 3.93 & Cluster  \\
\noalign{\smallskip} 
Abell 3880 & 0.05835 & HR-orange & 3$\times$600 & 2.57 & [OIII],[NI], &  22:27:54.51 &  -30:34:37.23 & 9.39 & 4.0 & Cluster \\
 & & & & & [OI], [SII] & & & & & \\
\noalign{\smallskip} 
Abell 3998 & 0.09019 & HR-orange & 3$\times$600 & 2.01 & [SII] &  23:21:33.25 &  -41:53:52.28 & 17.87 & 5.0 & Cluster \\
\noalign{\smallskip} 
Abell 4059 & 0.04900 & HR-orange & 3$\times$600 & 1.71 & [OI], [SII] &  23:57:00.51 &  -34:45:30.50 & 17.87 & 4.69 & Cluster  \\

\hline
\end{tabular}  
\caption[The  observational parameters of the VIMOS sample]{The observational parameters listed for each object in the VIMOS sample.  The first column states the cluster designation as used throughout this paper.  The redshift is the median redshift acquired from the fits to the H$\alpha$-[NII] complex, the median is calculated from the fits after dropping the top and bottom 2.5\% of the redshifts. The grating is the VIMOS grating used for the observations and the exposure lists the total integration time on target.  The seeing is calculated as the mean of the DIMM seeing across all exposures for each object.  The final column lists all lines apart from the H$\alpha$ and [NII] lines that were detected by visual inspection, the H$\alpha$--abs line is included for systems which show some evidence of stellar H$\alpha$ absorption.The right ascension and declination are measured at the centre of the field of view for each observation. X-ray luminosities were taken from the surveys of \citet{boh04,ebe98,ebe00} and temperatures are taken from \citet{ebe96,ebe98,ebe00,cav09}. The classifications are based on the x-ray properties following \citet{bah99}.}
\end{center}
%\label{tab:sam}
\end{table}

$^1$Defined as Groups based on their x-ray properties. While both Abell 194 and Abell 3574 are defined as clusters in the origonal abell cataloge \citep{abl58} they have a richness class of 0 putting them at the lowest end of the richness scale which may explain why their x-ray properties are consistent with those of groups.

\begin{table}
\ContinuedFloat
\begin{center}
\scriptsize

\smallskip
\begin{tabular}{c c c c c c c c c c c}
\hline
\noalign{\smallskip} 
Cluster & Redshift & Grating & Exposure & Mean & Lines & RA & Dec & L$_x$ & T$_x$ & Classification \\ 
 & & & (s) & Seeing('') & Detected & & & (10$^{43}$\,erg\,s$^{-1}$) & (keV) & \\[0.5ex]
\hline 
Abell 478       & 0.08556 & HR-orange & 3$\times$600 & 1.95 & H$\beta$, [OI], &  04:13:25.11 &  10:27:54.50 & 131.90 & 6.8 & Cluster  \\
 & & & & & [SII] & & & & & \\
\noalign{\smallskip} 
Abell 496       & 0.03294 & HR-orange & 3$\times$600 & 1.88 & [OI],  &  04:33:37.99 &  -13:15:50.56 & 20.54 & 3.89 & Cluster \\
\noalign{\smallskip} 
Abell 795       & 0.13487 & HR-red    & 3$\times$600 & 1.17 & [OI], [SII] &  09:24:05.12 &  14:10:19.34 & 56.60 & 6.6 & Cluster \\	
\noalign{\smallskip} 
Abell 85        & 0.05533 & HR-orange & 3$\times$600 & 1.00 & [OI], [SII] &  00:41:50.32 &  -09:18:07.01 & 56.31 & 6.9 & Cluster \\
\noalign{\smallskip} 
HCG62           & 0.01423 & HR-orange & 3$\times$600 & 0.63 & H$\alpha$--abs, [SII] & 12:53:05.48 &  -09:12:12.60 & 0.37 & 1.1 & Group  \\
\noalign{\smallskip} 
Hydra-A         & 0.05315 & HR-orange & 3$\times$600 & 1.38 & [OIII], [NI], & 09:18:05.52 &  -12:05:41.54 & 30.22 & 4.3 & Cluster  \\
 & & & & & [OI], [SII] & & & & & \\
\noalign{\smallskip} 
NGC4325         & 0.02547 & HR-orange & 3$\times$600 & 2.39 & [OI], [SII] &  12:23:06.36 &  10:37:14.48 & 2.0 & --- & Cluster \\
\noalign{\smallskip} 
NGC5044         & 0.00894 & HR-orange & 3$\times$600 & 2.23 & [OI], [SII] &  13:15:23.72 &  -16:23:03.84 & 1.10 & 1.22 & Group \\
\noalign{\smallskip} 
NGC533          & 0.01877 & HR-orange & 3$\times$400 & 0.92 & [SII] & 01:25:30.02 &  01:45:40.65 & 0.36 & --- & Group  \\
\noalign{\smallskip}
NGC5813         & 0.00677 & HR-orange & 3$\times$400 & 2.03 & [SII] &  15:01:11.00 &  01:42:01.99 & 0.14 & 0.76 & Group\\
\noalign{\smallskip} 
NGC5846         & 0.00611 & HR-orange & 3$\times$400 & 1.26 & [SII] &  15:06:28.90 &  01:36:15.78 & 0.11 & 0.64 & Group \\
\noalign{\smallskip} 		
RXCJ0120.9-1351 & 0.05060 & HR-orange & 3$\times$600 & 0.92 & [OI], [SII] & 01:20:58.40 &  -13:50:57.60 & 8.20 & --- & Cluster\\
\noalign{\smallskip} 
RXCJ0132.6-0804 & 0.14830 & HR-red    & 3$\times$600 & 0.75 & [OI],[SII] &  01:32:40.92 &  -08:04:02.06 & 21.73 & --- & Cluster \\
\noalign{\smallskip} 
RXCJ0331.1-2100 & 0.19276 & HR-red    & 3$\times$600 & 1.63 & [OI], [SII] &  03:31:05.72 &  -21:00:30.28 & 43.60 & 4.61 & Cluster \\
\noalign{\smallskip} 
RXCJ0543.4-4430 & 0.16377 & HR-red    & 3$\times$600 & 1.32 & [OI] &  05:43:24.77 &  -44:30:23.48 & 28.73 & --- & Cluster\\
\noalign{\smallskip} 
RXCJ0944.6-2633 & 0.14256 & HR-red    & 3$\times$600 & 0.43 & [OI], [SII] &  09:44:36.77 &  -26:44:52.17 & 35.10 & --- & Cluster  \\
\noalign{\smallskip} 
RXCJ1257.1-1339 & 0.01470 & HR-orange & 3$\times$400 & 1.63 & [OI], [SII] &  12:57:09.89 &  -13:39:17.14 & 0.16 & --- & Group \\
\noalign{\smallskip} 
RXCJ1304.2-3030 & 0.01093 & HR-orange & 3$\times$400 & 1.97 & [OI], [SII] &  13:04:16.90 &  -30:31:31.82 & 0.28 & --- & Group \\
\noalign{\smallskip} 
RXCJ1436.8-0900 & 0.08093 & HR-orange & 3$\times$600 & N/A & H$\beta$, [OIII], &  14:36:52.50 &  -09:00:19.97 & 7.98 & --- & Cluster \\
 & & & & & [NI], [OI], & & & & & \\
 & & & & & [SII] & & & & & \\
\noalign{\smallskip} 
RXCJ1511.5+0145 & 0.03983 & HR-orange & 3$\times$400 & 1.68 & [SII] &  15:11:33.28 &  01:45:47.40 & 0.85 & --- & Group\\
\noalign{\smallskip} 
RXCJ1524.2-3154 & 0.10190 & HR-orange & 3$\times$600 & 1.27 & H$\beta$, [OIII], &  15:24:12.57 &  -31:54:09.99  & 31.42 & --- & Cluster \\
 & & & & & [NI], [OI], & & & & & \\
 & & & & & [SII] & & & & & \\
\noalign{\smallskip} 
RXCJ1539.5-8335 & 0.07554 & HR-orange & 3$\times$600 & 0.47 & [OI](6300), &  15:39:33.51 &  -83:35:32.35 & 25.02 & --- & Cluster \\  
 & & & & & [SII], & & & & & \\
\noalign{\smallskip} 
RXCJ1558.3-1410 & 0.09680 & HR-orange & 3$\times$600 & 1.17 & H$\beta$, [OIII], &  15:58:21.70 &  -14:09:55.25 & 35.74 & --- & Cluster  \\ 
 & & & & & [NI], [OI], & & & & & \\
 & & & & & [SII], & & & & & \\
\noalign{\smallskip} 
RXCJ2014.8-2430 & 0.15515 & HR-red    & 2$\times$600 & 2.00 & [OI], [SII] &  20:14:51.70 &  -24:30:19.83 & 110.33 & --- & Cluster \\
\noalign{\smallskip} 
RXCJ2101.8-2802 & 0.03332 & HR-orange & 4$\times$600 & 0.90 & [OI], [SII] &  21:01:59.47 &  -28:03:29.96 & 3.03 & --- & Cluster \\
\noalign{\smallskip} 
RXCJ2129.6+0005 & 0.23394 & HR-red    & 3$\times$600 & 1.80 & [SII] &  21:29:40.16 &  00:05:30.58 & 185.90 & --- & Cluster \\
\noalign{\smallskip} 
RXCJ2213.0-2753 & 0.06128 & HR-orange & 3$\times$600 & 1.27 & [OI], [SII] &  22:13:06.04 &  -27:54:17.79 & 3.16 & --- & Cluster\\
\noalign{\smallskip} 
RXJ0000.1+0816  & 0.03927 & HR-orange & 3$\times$600 & 1.48 & [OI], [SII] &  00:00:06.92 &  08:16:45.27 & 3.80 & 2.3 & Cluster \\
\noalign{\smallskip} 
RXJ0338+09      & 0.03445 & HR-orange & 3$\times$600 & 1.27 & [NI], [OI], &  03:38:40.27 &  09:58:09.62 & 42.10 & 3.0 & Cluster  \\
 & & & & & [SII], & & & & & \\
\noalign{\smallskip} 
RXJ0352.9+1941  & 0.10833 & HR-orange & 3$\times$600 & 1.67 & H$\beta$, [OIII], &  03:52:58.83 &  19:40:57.01 & 39.80 & 5.7 & Cluster  \\
 & & & & & [NI], [OI], & & & & & \\
 & & & & & [SII], & & & & & \\
\noalign{\smallskip} 
RXJ0439.0+0520  & 0.20760 & HR-red    & 3$\times$600 & 1.27 & [SII] &  04:39:02.18 &  05:20:38.58 & 86.20 & 7.9 & Cluster  \\
\noalign{\smallskip} 
RXJ0747-19      & 0.10266 & HR-orange & 3$\times$600 & 1.5 & H$\beta$, [OIII], &  07:47:31.16 &  -19:17:38.23 & 280.00 & 8.5 & Cluster  \\
 & & & & & [NI], [OI], & & & & & \\
 & & & & & [SII], & & & & & \\
\noalign{\smallskip} 
RXJ0821+07      & 0.11088 & HR-orange & 3$\times$600 & 1.25 & H$\beta$, [OIII], &  08:21:02.36 &  07:51:44.13 & 20.90 & 4.4 & Cluster \\
 & & & & & [OI], [SII], & & & & & \\
\noalign{\smallskip} 
RXJ1651.1+0459  & 0.15467 & HR-red    & 3$\times$600 & 1.00 & [OI], [SII] &  16:51:07.96 &  04:59:27.89  & 56.20 & 6.6 & Cluster\\
\noalign{\smallskip} 	
S555            & 0.04484 & HR-orange & 3$\times$600 & 1.75 & [OI], [SII] &  05:57:12.39 &  -37:28:35.30 & 3.35 & --- & Cluster \\
\noalign{\smallskip} 
S780            & 0.23412 & HR-red    & 3$\times$600 & 1.50 & [OI], [SII] &  14:59:28.56 &  -18:10:42.50 & 155.31 & --- & Cluster \\
\noalign{\smallskip} 
S805            & 0.01518 & HR-orange & 3$\times$600 & 1.25 & [SII] &  18:47:19.88 &  -63:20:10.23 & 0.34 & --- & Group \\
\noalign{\smallskip} 
S851            & 0.00941 & HR-orange & 3$\times$600 & 1.25 & [OI], [SII] &  20:09:53.57 &  -48:22:44.85 & 0.10 & --- & Group  \\
\noalign{\smallskip} 
Z3179           & 0.14229 & HR-red    & 3$\times$600 & 1.00 & [OI], [SII] &  10:25:57.77 &  12:41:05.50 & 47.80 & 6.2 & Cluster  \\
\noalign{\smallskip} 
Z348            & 0.25286 & HR-red    & 3$\times$600 & 1.75 & [NI], [OI], &  01:06:49.14 &  01:03:19.93 & 98.00 & 8.4 & Cluster \\
 & & & & & [SII], & & & & & \\

\hline
\end{tabular}  
\caption[]{continued.}
\end{center}
%\label{tab:sam}
\end{table}

%Appendix B-----------------------------------------------------------------------------------

\clearpage
\onecolumn
%\thispagestyle{headings}
%\mbox{}
\section{Channel Maps}
\label{app:chan}

\bgroup
%  1 is the default, change whatever you need
\begin{tabular}[t]{c}
\epsfig{figure=/media/stephen/HYDRA/Backup/Obs/lvjm32/Vimos-ifu/Channelmaps/Maps3/A1060_chan.ps,width=12.7cm} \\
\epsfig{figure=/media/stephen/HYDRA/Backup/Obs/lvjm32/Vimos-ifu/Channelmaps/Maps3/A1084_chan.ps,width=12.7cm} \\
\end{tabular}
\clearpage
\begin{tabular}[t]{c}
\epsfig{figure=/media/stephen/HYDRA/Backup/Obs/lvjm32/Vimos-ifu/Channelmaps/Maps3/A1111_chan.ps,width=12.7cm} \\
\epsfig{figure=/media/stephen/HYDRA/Backup/Obs/lvjm32/Vimos-ifu/Channelmaps/Maps3/A11_chan.ps,width=12.7cm} \\
\end{tabular}
\clearpage
\begin{tabular}[t]{c}
\epsfig{figure=/media/stephen/HYDRA/Backup/Obs/lvjm32/Vimos-ifu/Channelmaps/Maps3/A1204_chan.ps,width=12.7cm} \\
\epsfig{figure=/media/stephen/HYDRA/Backup/Obs/lvjm32/Vimos-ifu/Channelmaps/Maps3/A133_chan.ps,width=12.7cm} \\
\end{tabular}
\clearpage
\begin{tabular}[t]{c}
\epsfig{figure=/media/stephen/HYDRA/Backup/Obs/lvjm32/Vimos-ifu/Channelmaps/Maps3/A1348_chan.ps,width=12.7cm} \\
\epsfig{figure=/media/stephen/HYDRA/Backup/Obs/lvjm32/Vimos-ifu/Channelmaps/Maps3/A1663_chan.ps,width=12.7cm} \\
\end{tabular}
\clearpage
\vspace{-1cm}
\begin{tabular}[t]{c}
\epsfig{figure=/media/stephen/HYDRA/Backup/Obs/lvjm32/Vimos-ifu/Channelmaps/Maps3/A1668_chan.ps,width=12.7cm} \\
\vspace{-1cm}
\epsfig{figure=/media/stephen/HYDRA/Backup/Obs/lvjm32/Vimos-ifu/Channelmaps/Maps3/A194_chan.ps,width=12.7cm} \\
\end{tabular}
\clearpage
\begin{tabular}[t]{c}
\epsfig{figure=/media/stephen/HYDRA/Backup/Obs/lvjm32/Vimos-ifu/Channelmaps/Maps3/A1991-added_chan.ps,width=12.7cm} \\
\epsfig{figure=/media/stephen/HYDRA/Backup/Obs/lvjm32/Vimos-ifu/Channelmaps/Maps3/A2052_chan.ps,width=12.7cm} \\
\end{tabular}
\clearpage
\begin{tabular}[t]{c}
\epsfig{figure=/media/stephen/HYDRA/Backup/Obs/lvjm32/Vimos-ifu/Channelmaps/Maps3/A2390_chan.ps,width=12.7cm} \\
\epsfig{figure=/media/stephen/HYDRA/Backup/Obs/lvjm32/Vimos-ifu/Channelmaps/Maps3/A2415_chan.ps,width=12.7cm} \\
\end{tabular}
\clearpage
\begin{tabular}[t]{c}
\epsfig{figure=/media/stephen/HYDRA/Backup/Obs/lvjm32/Vimos-ifu/Channelmaps/Maps3/A2495_chan.ps,width=12.7cm} \\
\epsfig{figure=/media/stephen/HYDRA/Backup/Obs/lvjm32/Vimos-ifu/Channelmaps/Maps3/A2566_chan.ps,width=12.7cm} \\
\end{tabular}
\clearpage
\begin{tabular}[t]{c}
\epsfig{figure=/media/stephen/HYDRA/Backup/Obs/lvjm32/Vimos-ifu/Channelmaps/Maps3/A2580_chan.ps,width=12.7cm} \\
\epsfig{figure=/media/stephen/HYDRA/Backup/Obs/lvjm32/Vimos-ifu/Channelmaps/Maps3/A2734_chan.ps,width=12.7cm} \\
\end{tabular}
\clearpage
\begin{tabular}[t]{c}
\epsfig{figure=/media/stephen/HYDRA/Backup/Obs/lvjm32/Vimos-ifu/Channelmaps/Maps3/A291_chan.ps,width=12.7cm} \\
\epsfig{figure=/media/stephen/HYDRA/Backup/Obs/lvjm32/Vimos-ifu/Channelmaps/Maps3/A3017_chan.ps,width=12.7cm} \\
\end{tabular}
\clearpage
\begin{tabular}[t]{c}
\epsfig{figure=/media/stephen/HYDRA/Backup/Obs/lvjm32/Vimos-ifu/Channelmaps/Maps3/A3112_chan.ps,width=12.7cm} \\
\epsfig{figure=/media/stephen/HYDRA/Backup/Obs/lvjm32/Vimos-ifu/Channelmaps/Maps3/A3378_chan.ps,width=12.7cm} \\
\end{tabular}
\clearpage
\begin{tabular}[t]{c}
\epsfig{figure=/media/stephen/HYDRA/Backup/Obs/lvjm32/Vimos-ifu/Channelmaps/Maps3/A3444_chan.ps,width=12.7cm} \\
\epsfig{figure=/media/stephen/HYDRA/Backup/Obs/lvjm32/Vimos-ifu/Channelmaps/Maps3/A3574_chan.ps,width=12.7cm} \\
\end{tabular}
\clearpage
\begin{tabular}[t]{c}
\epsfig{figure=/media/stephen/HYDRA/Backup/Obs/lvjm32/Vimos-ifu/Channelmaps/Maps3/A3581_chan.ps,width=12.7cm} \\
\epsfig{figure=/media/stephen/HYDRA/Backup/Obs/lvjm32/Vimos-ifu/Channelmaps/Maps3/A3605_chan.ps,width=12.7cm} \\
\end{tabular}
\clearpage
\begin{tabular}[t]{c}
\epsfig{figure=/media/stephen/HYDRA/Backup/Obs/lvjm32/Vimos-ifu/Channelmaps/Maps3/A3638_chan.ps,width=12.7cm} \\
\epsfig{figure=/media/stephen/HYDRA/Backup/Obs/lvjm32/Vimos-ifu/Channelmaps/Maps3/A3639_chan.ps,width=12.7cm} \\
\end{tabular}
\clearpage
\begin{tabular}[t]{c}
\epsfig{figure=/media/stephen/HYDRA/Backup/Obs/lvjm32/Vimos-ifu/Channelmaps/Maps3/A3806_chan.ps,width=12.7cm} \\
\epsfig{figure=/media/stephen/HYDRA/Backup/Obs/lvjm32/Vimos-ifu/Channelmaps/Maps3/A383_chan.ps,width=12.7cm} \\
\end{tabular}
\clearpage
\begin{tabular}[t]{c}
\epsfig{figure=/media/stephen/HYDRA/Backup/Obs/lvjm32/Vimos-ifu/Channelmaps/Maps3/A3880_chan.ps,width=12.7cm} \\
\epsfig{figure=/media/stephen/HYDRA/Backup/Obs/lvjm32/Vimos-ifu/Channelmaps/Maps3/A3998_chan.ps,width=12.7cm} \\
\end{tabular}
\clearpage
\begin{tabular}[t]{c}
\epsfig{figure=/media/stephen/HYDRA/Backup/Obs/lvjm32/Vimos-ifu/Channelmaps/Maps3/A4059_chan.ps,width=12.7cm} \\
\epsfig{figure=/media/stephen/HYDRA/Backup/Obs/lvjm32/Vimos-ifu/Channelmaps/Maps3/A478_chan.ps,width=12.7cm} \\
\end{tabular}
\clearpage
\begin{tabular}[t]{c}
\epsfig{figure=/media/stephen/HYDRA/Backup/Obs/lvjm32/Vimos-ifu/Channelmaps/Maps3/A496_chan.ps,width=12.7cm} \\
\epsfig{figure=/media/stephen/HYDRA/Backup/Obs/lvjm32/Vimos-ifu/Channelmaps/Maps3/A795_chan.ps,width=12.7cm} \\
\end{tabular}
\clearpage
\begin{tabular}[t]{c}
\epsfig{figure=/media/stephen/HYDRA/Backup/Obs/lvjm32/Vimos-ifu/Channelmaps/Maps3/A85_chan.ps,width=12.7cm} \\
\epsfig{figure=/media/stephen/HYDRA/Backup/Obs/lvjm32/Vimos-ifu/Channelmaps/Maps3/HCG62_chan.ps,width=12.7cm} \\
\end{tabular}
\clearpage
\begin{tabular}[t]{c}
\epsfig{figure=/media/stephen/HYDRA/Backup/Obs/lvjm32/Vimos-ifu/Channelmaps/Maps3/Hydra-a_chan.ps,width=12.7cm} \\
\epsfig{figure=/media/stephen/HYDRA/Backup/Obs/lvjm32/Vimos-ifu/Channelmaps/Maps3/NGC4325_chan.ps,width=12.7cm} \\
\end{tabular}
\clearpage
\begin{tabular}[t]{c}
\epsfig{figure=/media/stephen/HYDRA/Backup/Obs/lvjm32/Vimos-ifu/Channelmaps/Maps3/NGC5044_chan.ps,width=12.7cm} \\
\epsfig{figure=/media/stephen/HYDRA/Backup/Obs/lvjm32/Vimos-ifu/Channelmaps/Maps3/NGC533_chan.ps,width=12.7cm} \\
\end{tabular}
\clearpage
\begin{tabular}[t]{c}
\epsfig{figure=/media/stephen/HYDRA/Backup/Obs/lvjm32/Vimos-ifu/Channelmaps/Maps3/NGC5813_chan.ps,width=12.7cm} \\
\epsfig{figure=/media/stephen/HYDRA/Backup/Obs/lvjm32/Vimos-ifu/Channelmaps/Maps3/NGC5846_chan.ps,width=12.7cm} \\
\end{tabular}
\clearpage
\begin{tabular}[t]{c}
\epsfig{figure=/media/stephen/HYDRA/Backup/Obs/lvjm32/Vimos-ifu/Channelmaps/Maps3/RXCJ0120.9-1351_chan.ps,width=12.7cm} \\
\epsfig{figure=/media/stephen/HYDRA/Backup/Obs/lvjm32/Vimos-ifu/Channelmaps/Maps3/RXCJ0132.6-0804_chan.ps,width=12.7cm} \\
\end{tabular}
\clearpage
\begin{tabular}[t]{c}
\epsfig{figure=/media/stephen/HYDRA/Backup/Obs/lvjm32/Vimos-ifu/Channelmaps/Maps3/RXCJ0331.1-2100_chan.ps,width=12.7cm} \\
\epsfig{figure=/media/stephen/HYDRA/Backup/Obs/lvjm32/Vimos-ifu/Channelmaps/Maps3/RXCJ0543.4-4430_chan.ps,width=12.7cm} \\
\end{tabular}
\clearpage
\begin{tabular}[t]{c}
\epsfig{figure=/media/stephen/HYDRA/Backup/Obs/lvjm32/Vimos-ifu/Channelmaps/Maps3/RXCJ0944.6-2633_chan.ps,width=12.7cm} \\
\epsfig{figure=/media/stephen/HYDRA/Backup/Obs/lvjm32/Vimos-ifu/Channelmaps/Maps3/RXCJ1257.1-1339_chan.ps,width=12.7cm} \\
\end{tabular}
\clearpage
\begin{tabular}[t]{c}
\epsfig{figure=/media/stephen/HYDRA/Backup/Obs/lvjm32/Vimos-ifu/Channelmaps/Maps3/RXCJ1304.2-3030_chan.ps,width=12.7cm} \\
\epsfig{figure=/media/stephen/HYDRA/Backup/Obs/lvjm32/Vimos-ifu/Channelmaps/Maps3/RXCJ1436.8-0900_chan.ps,width=12.7cm} \\
\end{tabular}
\clearpage
\begin{tabular}[t]{c}
\epsfig{figure=/media/stephen/HYDRA/Backup/Obs/lvjm32/Vimos-ifu/Channelmaps/Maps3/RXCJ1511.5+0145_chan.ps,width=12.7cm} \\
\epsfig{figure=/media/stephen/HYDRA/Backup/Obs/lvjm32/Vimos-ifu/Channelmaps/Maps3/RXCJ1524.2-3154_chan.ps,width=12.7cm} \\
\end{tabular}
\clearpage
\begin{tabular}[t]{c}
\epsfig{figure=/media/stephen/HYDRA/Backup/Obs/lvjm32/Vimos-ifu/Channelmaps/Maps3/RXCJ1539.5-8335_chan.ps,width=12.7cm} \\
\epsfig{figure=/media/stephen/HYDRA/Backup/Obs/lvjm32/Vimos-ifu/Channelmaps/Maps3/RXCJ1558.3-1410_chan.ps,width=12.7cm} \\
\end{tabular}
\clearpage
\begin{tabular}[t]{c}
\epsfig{figure=/media/stephen/HYDRA/Backup/Obs/lvjm32/Vimos-ifu/Channelmaps/Maps3/RXCJ2014.8-2430_chan.ps,width=12.7cm} \\
\epsfig{figure=/media/stephen/HYDRA/Backup/Obs/lvjm32/Vimos-ifu/Channelmaps/Maps3/RXCJ2101.8-2802_chan.ps,width=12.7cm} \\
\end{tabular}
\clearpage
\begin{tabular}[t]{c}
\epsfig{figure=/media/stephen/HYDRA/Backup/Obs/lvjm32/Vimos-ifu/Channelmaps/Maps3/RXCJ2129.6+0005_chan.ps,width=12.7cm} \\
\epsfig{figure=/media/stephen/HYDRA/Backup/Obs/lvjm32/Vimos-ifu/Channelmaps/Maps3/RXCJ2213.0-2753_chan.ps,width=12.7cm} \\
\end{tabular}
\clearpage
\begin{tabular}[t]{c}
\epsfig{figure=/media/stephen/HYDRA/Backup/Obs/lvjm32/Vimos-ifu/Channelmaps/Maps3/RXJ0000.1+0816_chan.ps,width=12.7cm} \\
\epsfig{figure=/media/stephen/HYDRA/Backup/Obs/lvjm32/Vimos-ifu/Channelmaps/Maps3/RXJ0338+09_chan.ps,width=12.7cm} \\
\end{tabular}
\clearpage
\begin{tabular}[t]{c}
\epsfig{figure=/media/stephen/HYDRA/Backup/Obs/lvjm32/Vimos-ifu/Channelmaps/Maps3/RXJ0352.9+1941_chan.ps,width=12.7cm} \\
\epsfig{figure=/media/stephen/HYDRA/Backup/Obs/lvjm32/Vimos-ifu/Channelmaps/Maps3/RXJ0439.0+0520_chan.ps,width=12.7cm} \\
\end{tabular}
\clearpage
\begin{tabular}[t]{c}
\epsfig{figure=/media/stephen/HYDRA/Backup/Obs/lvjm32/Vimos-ifu/Channelmaps/Maps3/RXJ0747-19_chan.ps,width=12.7cm} \\
\epsfig{figure=/media/stephen/HYDRA/Backup/Obs/lvjm32/Vimos-ifu/Channelmaps/Maps3/RXJ0821+07_chan.ps,width=12.7cm} \\
\end{tabular}
\clearpage
\begin{tabular}[t]{c}
\epsfig{figure=/media/stephen/HYDRA/Backup/Obs/lvjm32/Vimos-ifu/Channelmaps/Maps3/RXJ1651.1+0459_chan.ps,width=12.7cm} \\
\epsfig{figure=/media/stephen/HYDRA/Backup/Obs/lvjm32/Vimos-ifu/Channelmaps/Maps3/S555_chan.ps,width=12.7cm} \\
\end{tabular}
\clearpage
\begin{tabular}[t]{c}
\epsfig{figure=/media/stephen/HYDRA/Backup/Obs/lvjm32/Vimos-ifu/Channelmaps/Maps3/S780_chan.ps,width=12.7cm} \\
\epsfig{figure=/media/stephen/HYDRA/Backup/Obs/lvjm32/Vimos-ifu/Channelmaps/Maps3/S805_chan.ps,width=12.7cm} \\
\end{tabular}
\clearpage
\begin{tabular}[t]{c}
\epsfig{figure=/media/stephen/HYDRA/Backup/Obs/lvjm32/Vimos-ifu/Channelmaps/Maps3/S851_chan.ps,width=12.7cm} \\
\epsfig{figure=/media/stephen/HYDRA/Backup/Obs/lvjm32/Vimos-ifu/Channelmaps/Maps3/Z3179_chan.ps,width=12.7cm} \\
\end{tabular}
\clearpage
\begin{tabular}[t]{c}
\epsfig{figure=/media/stephen/HYDRA/Backup/Obs/lvjm32/Vimos-ifu/Channelmaps/Maps3/Z348_chan.ps,width=12.7cm} \\ 
\end{tabular}
\egroup

%Appendix C-------------------------------------------------------------------------------
\clearpage
\onecolumn
%\thispagestyle{headings}
%\mbox{}
\section{Maps of the spectral fits for the full sample}
\label{app:maps}

Maps of the spectral fits to the VIMOS data cubes for all 73 objects in the sample.  From left to right the panels are: 1) A continuum image created by collapsing the cube over a wavelength range free of emission and sky lines, 2) The H$\alpha$ flux map, 3) A map showing the ratio of [NII] to H$\alpha$ flux, 4) the line of sight velocity profile of the H$\alpha$ and [NII] emission, 4) the Full width at half maximum of the emission line deconvolved for instrumental resolution. For systems in which the H$\alpha$ line appears absorbed the flux, LOS velocity and FWHM are plotted for the [NII] line.

\includegraphics[width=17cm,bbllx=74,bblly=367,bburx=459,bbury=470]{/media/stephen/HYDRA/Backup/Obs/lvjm32/Thesis/Thesistex/Chap3/Figs/Abell1060_plots.ps}

\includegraphics[width=17cm,bbllx=74,bblly=367,bburx=459,bbury=470]{/media/stephen/HYDRA/Backup/Obs/lvjm32/Thesis/Thesistex/Chap3/Figs/Abell1084_plots.ps}

\includegraphics[width=17cm,bbllx=74,bblly=367,bburx=459,bbury=470]{/media/stephen/HYDRA/Backup/Obs/lvjm32/Thesis/Thesistex/Chap3/Figs/Abell11_plots.ps}

\includegraphics[width=17cm,bbllx=74,bblly=367,bburx=459,bbury=470]{/media/stephen/HYDRA/Backup/Obs/lvjm32/Thesis/Thesistex/Chap3/Figs/Abell1111_plots.ps}
\clearpage
\includegraphics[width=17cm,bbllx=74,bblly=367,bburx=459,bbury=470]{/media/stephen/HYDRA/Backup/Obs/lvjm32/Thesis/Thesistex/Chap3/Figs/Abell1204_plots.ps}

\includegraphics[width=17cm,bbllx=74,bblly=367,bburx=459,bbury=470]{/media/stephen/HYDRA/Backup/Obs/lvjm32/Thesis/Thesistex/Chap3/Figs/Abell133_plots.ps}

\includegraphics[width=17cm,bbllx=74,bblly=367,bburx=459,bbury=470]{/media/stephen/HYDRA/Backup/Obs/lvjm32/Thesis/Thesistex/Chap3/Figs/Abell1348_plots.ps}

\includegraphics[width=17cm,bbllx=74,bblly=367,bburx=459,bbury=470]{/media/stephen/HYDRA/Backup/Obs/lvjm32/Thesis/Thesistex/Chap3/Figs/Abell1663_plots.ps}

\includegraphics[width=17cm,bbllx=74,bblly=367,bburx=459,bbury=470]{/media/stephen/HYDRA/Backup/Obs/lvjm32/Thesis/Thesistex/Chap3/Figs/Abell1668_plots.ps}
\clearpage
\includegraphics[width=17cm,bbllx=74,bblly=367,bburx=459,bbury=470]{/media/stephen/HYDRA/Backup/Obs/lvjm32/Thesis/Thesistex/Chap3/Figs/Abell194_plots.ps}

\includegraphics[width=17cm,bbllx=74,bblly=367,bburx=459,bbury=470]{/media/stephen/HYDRA/Backup/Obs/lvjm32/Thesis/Thesistex/Chap3/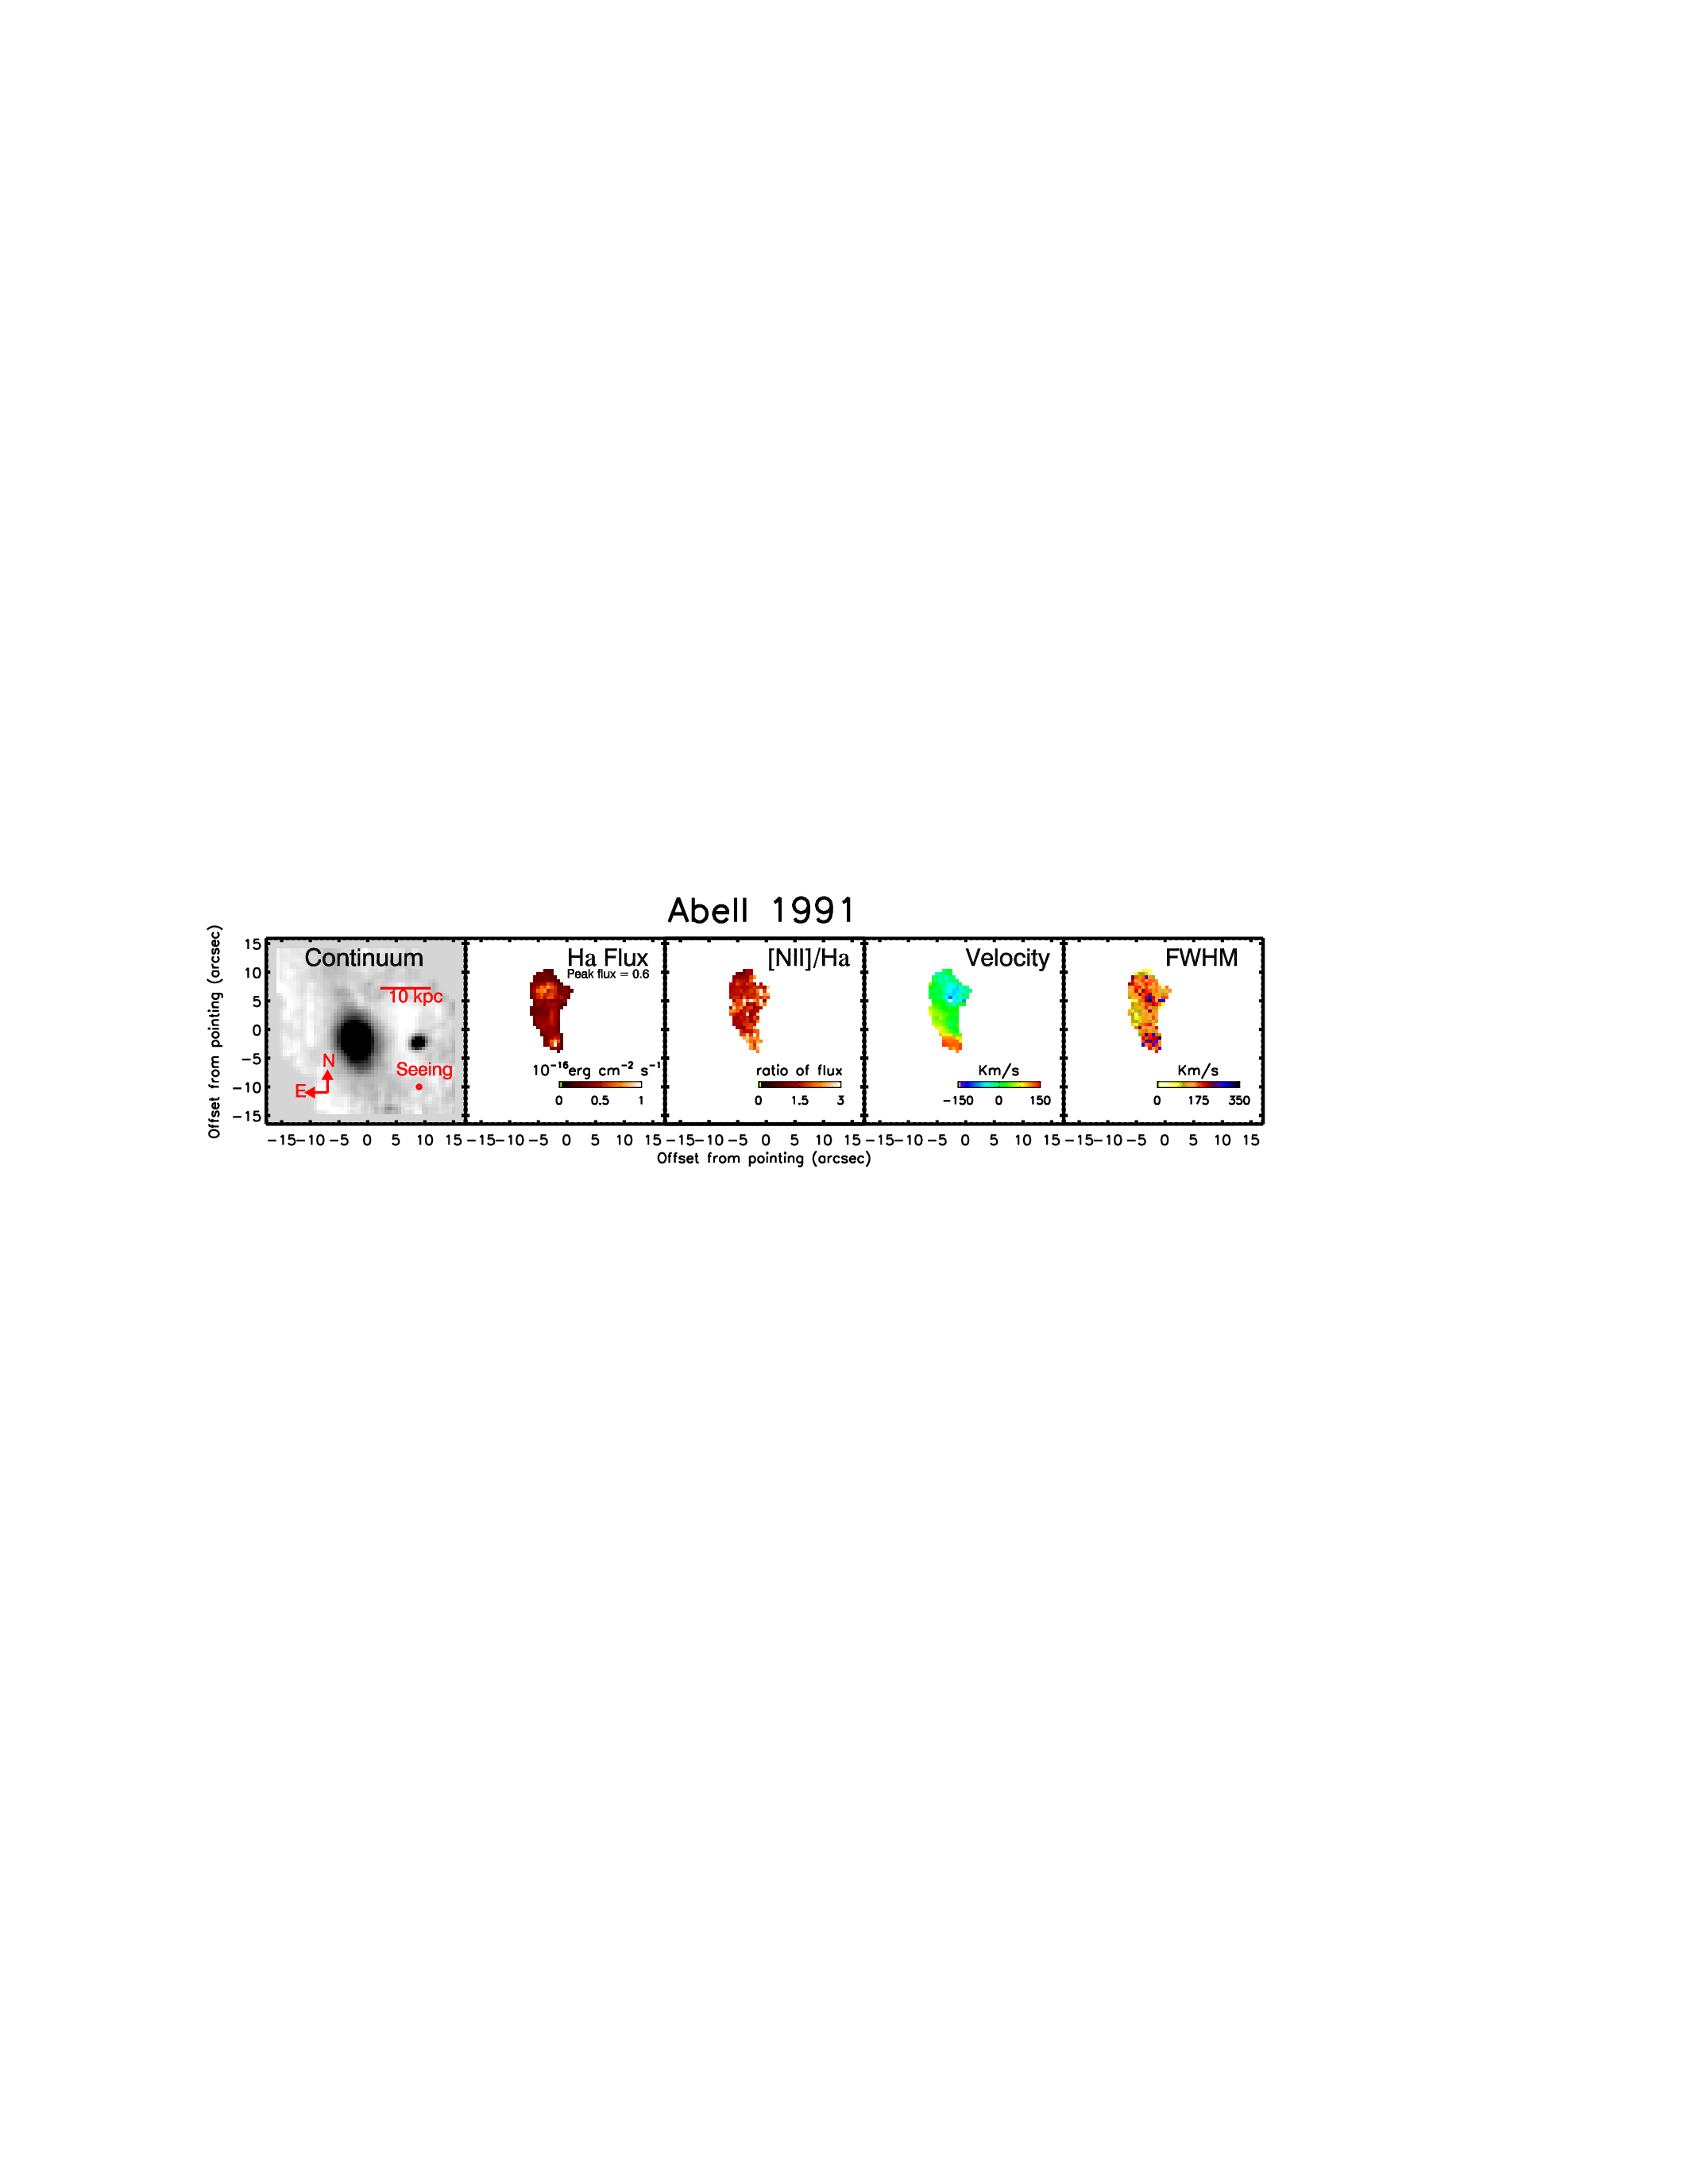}

\includegraphics[width=17cm,bbllx=74,bblly=367,bburx=459,bbury=470]{/media/stephen/HYDRA/Backup/Obs/lvjm32/Thesis/Thesistex/Chap3/Figs/Abell2052_plots.ps}

\includegraphics[width=17cm,bbllx=74,bblly=367,bburx=459,bbury=470]{/media/stephen/HYDRA/Backup/Obs/lvjm32/Thesis/Thesistex/Chap3/Figs/Abell2390_plots.ps}

\includegraphics[width=17cm,bbllx=74,bblly=367,bburx=459,bbury=470]{/media/stephen/HYDRA/Backup/Obs/lvjm32/Thesis/Thesistex/Chap3/Figs/Abell2415_plots.ps}
\clearpage
\includegraphics[width=17cm,bbllx=74,bblly=367,bburx=459,bbury=470]{/media/stephen/HYDRA/Backup/Obs/lvjm32/Thesis/Thesistex/Chap3/Figs/Abell2495_plots.ps}

\includegraphics[width=17cm,bbllx=74,bblly=367,bburx=459,bbury=470]{/media/stephen/HYDRA/Backup/Obs/lvjm32/Thesis/Thesistex/Chap3/Figs/Abell2566_plots.ps}

\includegraphics[width=17cm,bbllx=74,bblly=367,bburx=459,bbury=470]{/media/stephen/HYDRA/Backup/Obs/lvjm32/Thesis/Thesistex/Chap3/Figs/Abell2580_plots.ps}

\includegraphics[width=17cm,bbllx=74,bblly=367,bburx=459,bbury=470]{/media/stephen/HYDRA/Backup/Obs/lvjm32/Thesis/Thesistex/Chap3/Figs/Abell2734_plots.ps}

\includegraphics[width=17cm,bbllx=74,bblly=367,bburx=459,bbury=470]{/media/stephen/HYDRA/Backup/Obs/lvjm32/Thesis/Thesistex/Chap3/Figs/Abell291_plots.ps}
\clearpage
\includegraphics[width=17cm,bbllx=74,bblly=367,bburx=459,bbury=470]{/media/stephen/HYDRA/Backup/Obs/lvjm32/Thesis/Thesistex/Chap3/Figs/Abell3017_plots.ps}

\includegraphics[width=17cm,bbllx=74,bblly=367,bburx=459,bbury=470]{/media/stephen/HYDRA/Backup/Obs/lvjm32/Thesis/Thesistex/Chap3/Figs/Abell3112_plots.ps}

\includegraphics[width=17cm,bbllx=74,bblly=367,bburx=459,bbury=470]{/media/stephen/HYDRA/Backup/Obs/lvjm32/Thesis/Thesistex/Chap3/Figs/Abell3378_plots.ps}

\includegraphics[width=17cm,bbllx=74,bblly=367,bburx=459,bbury=470]{/media/stephen/HYDRA/Backup/Obs/lvjm32/Thesis/Thesistex/Chap3/Figs/Abell3444_plots.ps}

\includegraphics[width=17cm,bbllx=74,bblly=367,bburx=459,bbury=470]{/media/stephen/HYDRA/Backup/Obs/lvjm32/Thesis/Thesistex/Chap3/Figs/Abell3574_plots.ps}
\clearpage
\includegraphics[width=17cm,bbllx=74,bblly=367,bburx=459,bbury=470]{/media/stephen/HYDRA/Backup/Obs/lvjm32/Thesis/Thesistex/Chap3/Figs/Abell3581_plots.ps}

\includegraphics[width=17cm,bbllx=74,bblly=367,bburx=459,bbury=470]{/media/stephen/HYDRA/Backup/Obs/lvjm32/Thesis/Thesistex/Chap3/Figs/Abell3605_plots.ps}

\includegraphics[width=17cm,bbllx=74,bblly=367,bburx=459,bbury=470]{/media/stephen/HYDRA/Backup/Obs/lvjm32/Thesis/Thesistex/Chap3/Figs/Abell3638_plots.ps}

\includegraphics[width=17cm,bbllx=74,bblly=367,bburx=459,bbury=470]{/media/stephen/HYDRA/Backup/Obs/lvjm32/Thesis/Thesistex/Chap3/Figs/Abell3639_plots.ps}

\includegraphics[width=17cm,bbllx=74,bblly=367,bburx=459,bbury=470]{/media/stephen/HYDRA/Backup/Obs/lvjm32/Thesis/Thesistex/Chap3/Figs/Abell3806_plots.ps}
\clearpage
\includegraphics[width=17cm,bbllx=74,bblly=367,bburx=459,bbury=470]{/media/stephen/HYDRA/Backup/Obs/lvjm32/Thesis/Thesistex/Chap3/Figs/Abell383_plots.ps}

\includegraphics[width=17cm,bbllx=74,bblly=367,bburx=459,bbury=470]{/media/stephen/HYDRA/Backup/Obs/lvjm32/Thesis/Thesistex/Chap3/Figs/Abell3880_plots.ps}

\includegraphics[width=17cm,bbllx=74,bblly=367,bburx=459,bbury=470]{/media/stephen/HYDRA/Backup/Obs/lvjm32/Thesis/Thesistex/Chap3/Figs/Abell3998_plots.ps}

\includegraphics[width=17cm,bbllx=74,bblly=367,bburx=459,bbury=470]{/media/stephen/HYDRA/Backup/Obs/lvjm32/Thesis/Thesistex/Chap3/Figs/Abell4059_plots.ps}

\includegraphics[width=17cm,bbllx=74,bblly=367,bburx=459,bbury=470]{/media/stephen/HYDRA/Backup/Obs/lvjm32/Thesis/Thesistex/Chap3/Figs/Abell478_plots.ps}
\clearpage
\includegraphics[width=17cm,bbllx=74,bblly=367,bburx=459,bbury=470]{/media/stephen/HYDRA/Backup/Obs/lvjm32/Thesis/Thesistex/Chap3/Figs/Abell496_plots.ps}

\includegraphics[width=17cm,bbllx=74,bblly=367,bburx=459,bbury=470]{/media/stephen/HYDRA/Backup/Obs/lvjm32/Thesis/Thesistex/Chap3/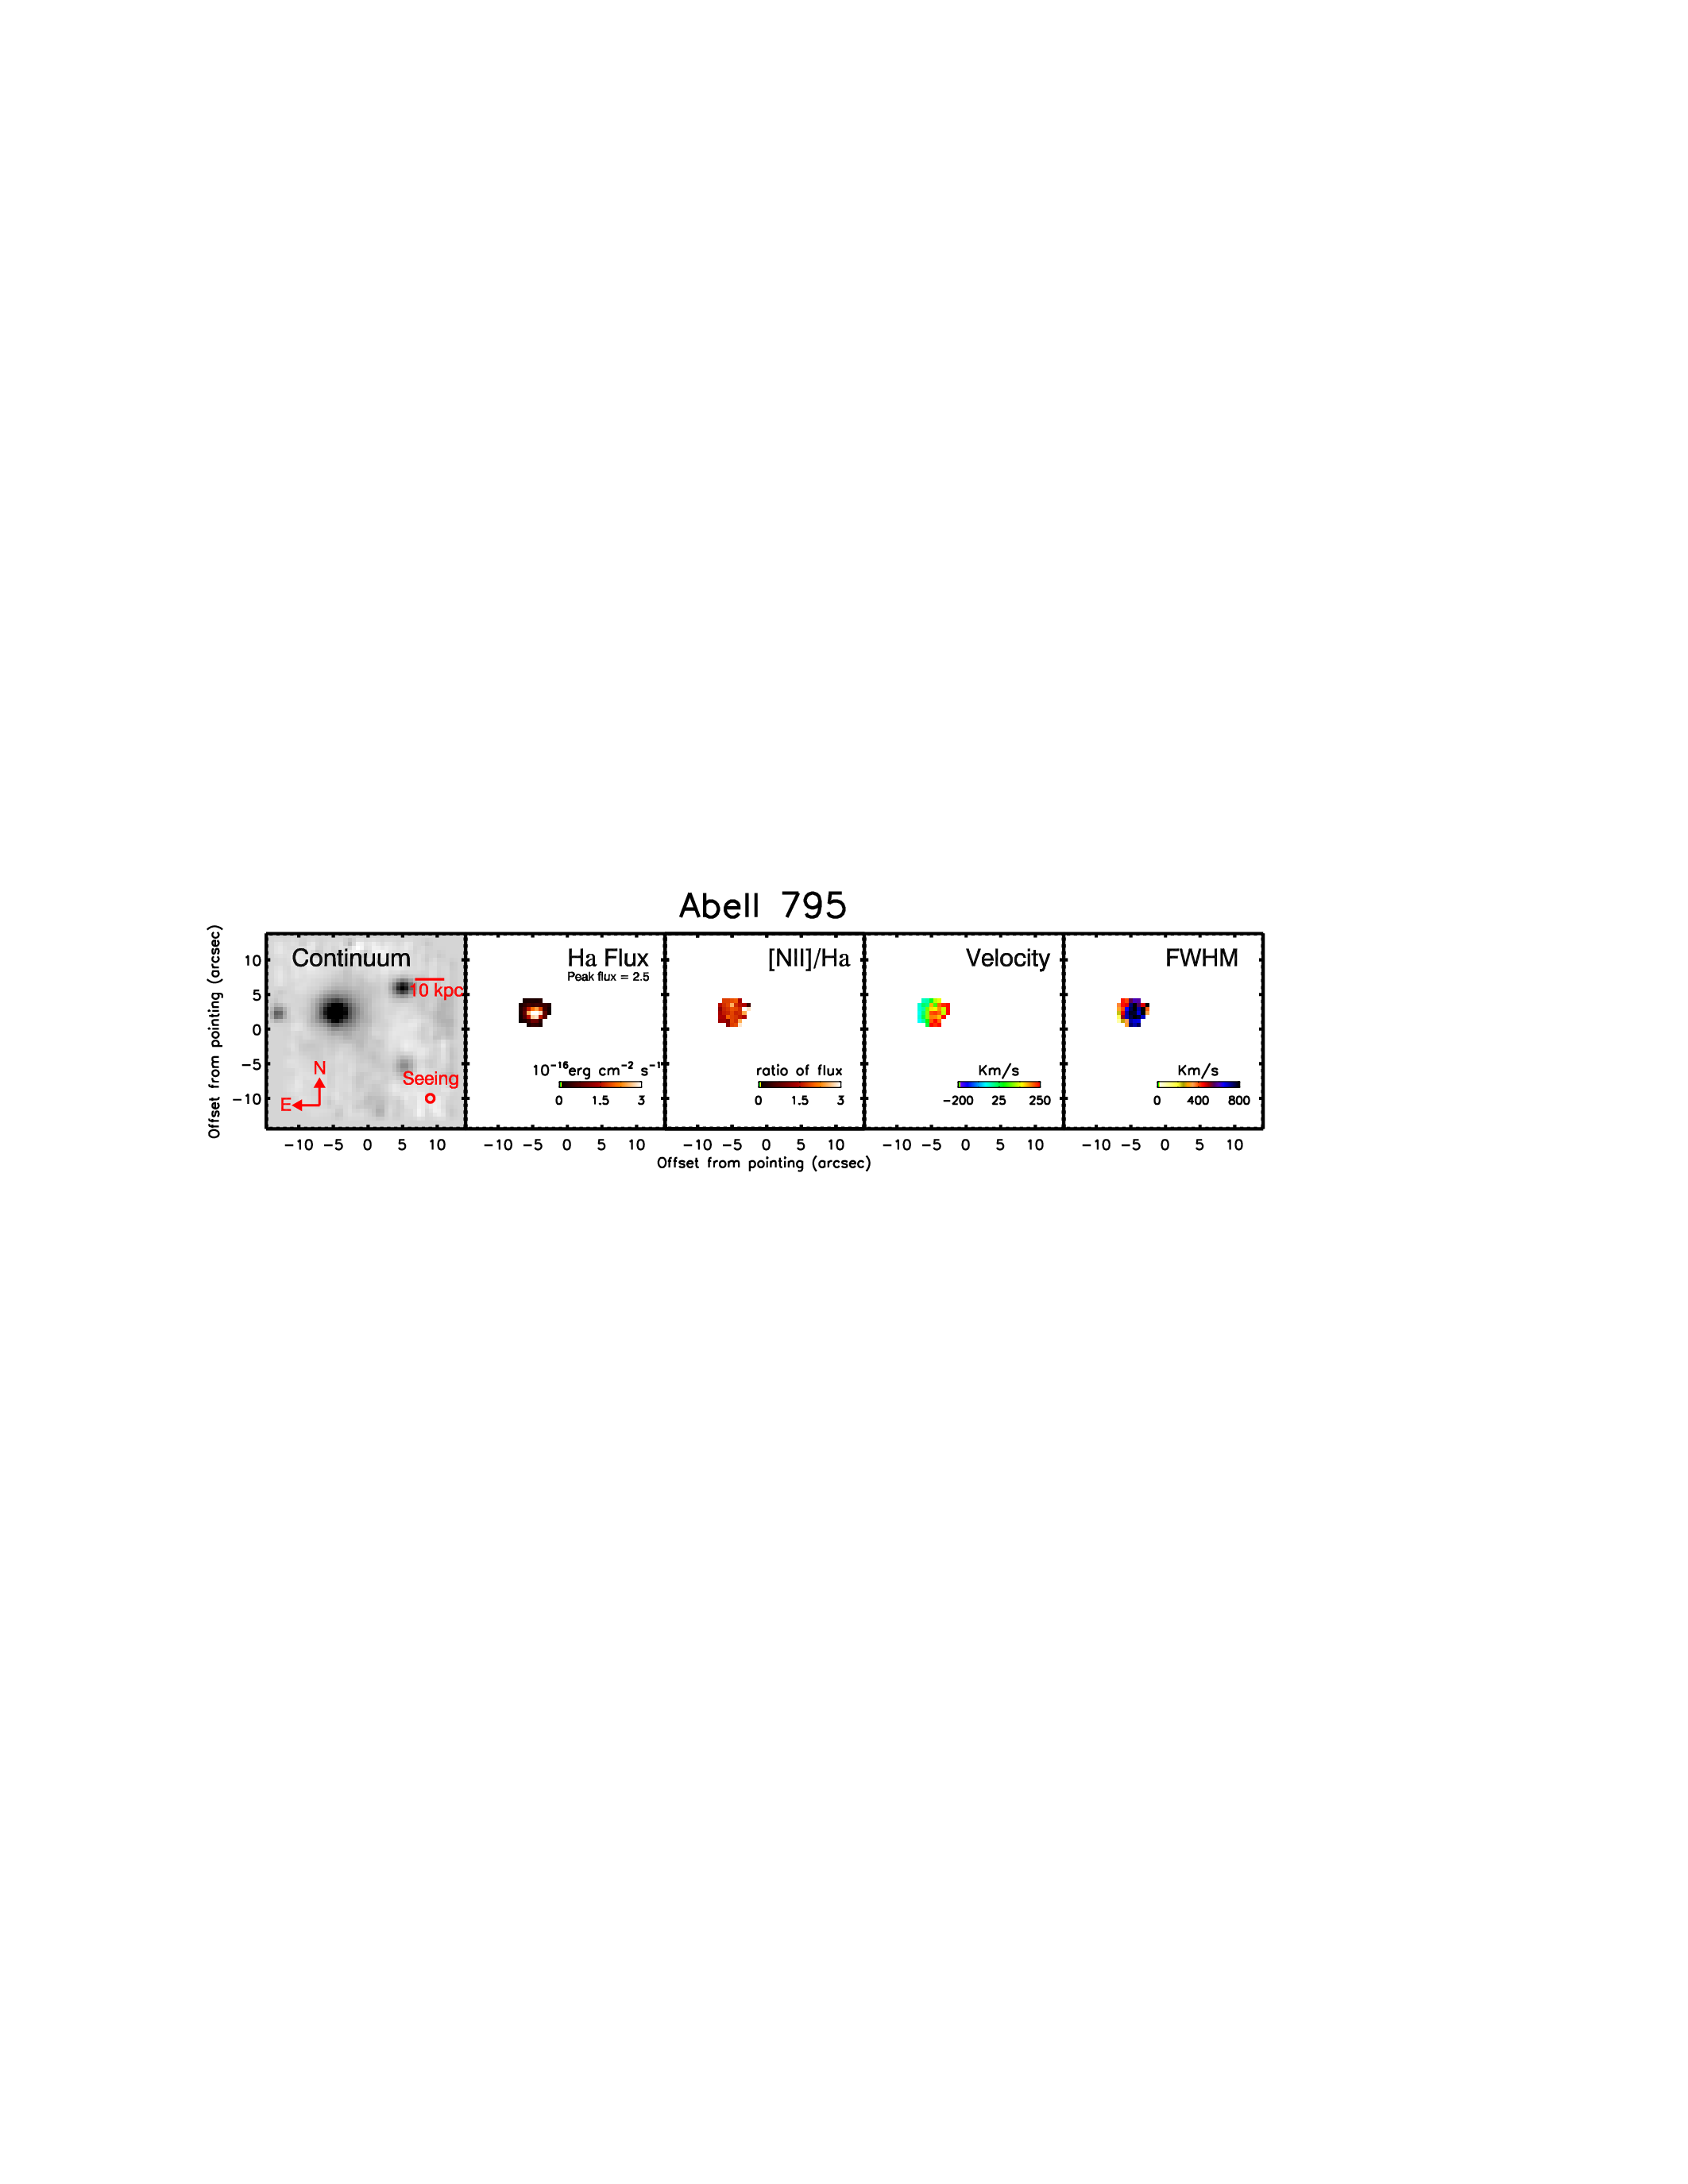}

\includegraphics[width=17cm,bbllx=74,bblly=367,bburx=459,bbury=470]{/media/stephen/HYDRA/Backup/Obs/lvjm32/Thesis/Thesistex/Chap3/Figs/Abell85_plots.ps}

\includegraphics[width=17cm,bbllx=74,bblly=367,bburx=459,bbury=470]{/media/stephen/HYDRA/Backup/Obs/lvjm32/Thesis/Thesistex/Chap3/Figs/HCG62_plots.ps}

\includegraphics[width=17cm,bbllx=74,bblly=367,bburx=459,bbury=470]{/media/stephen/HYDRA/Backup/Obs/lvjm32/Thesis/Thesistex/Chap3/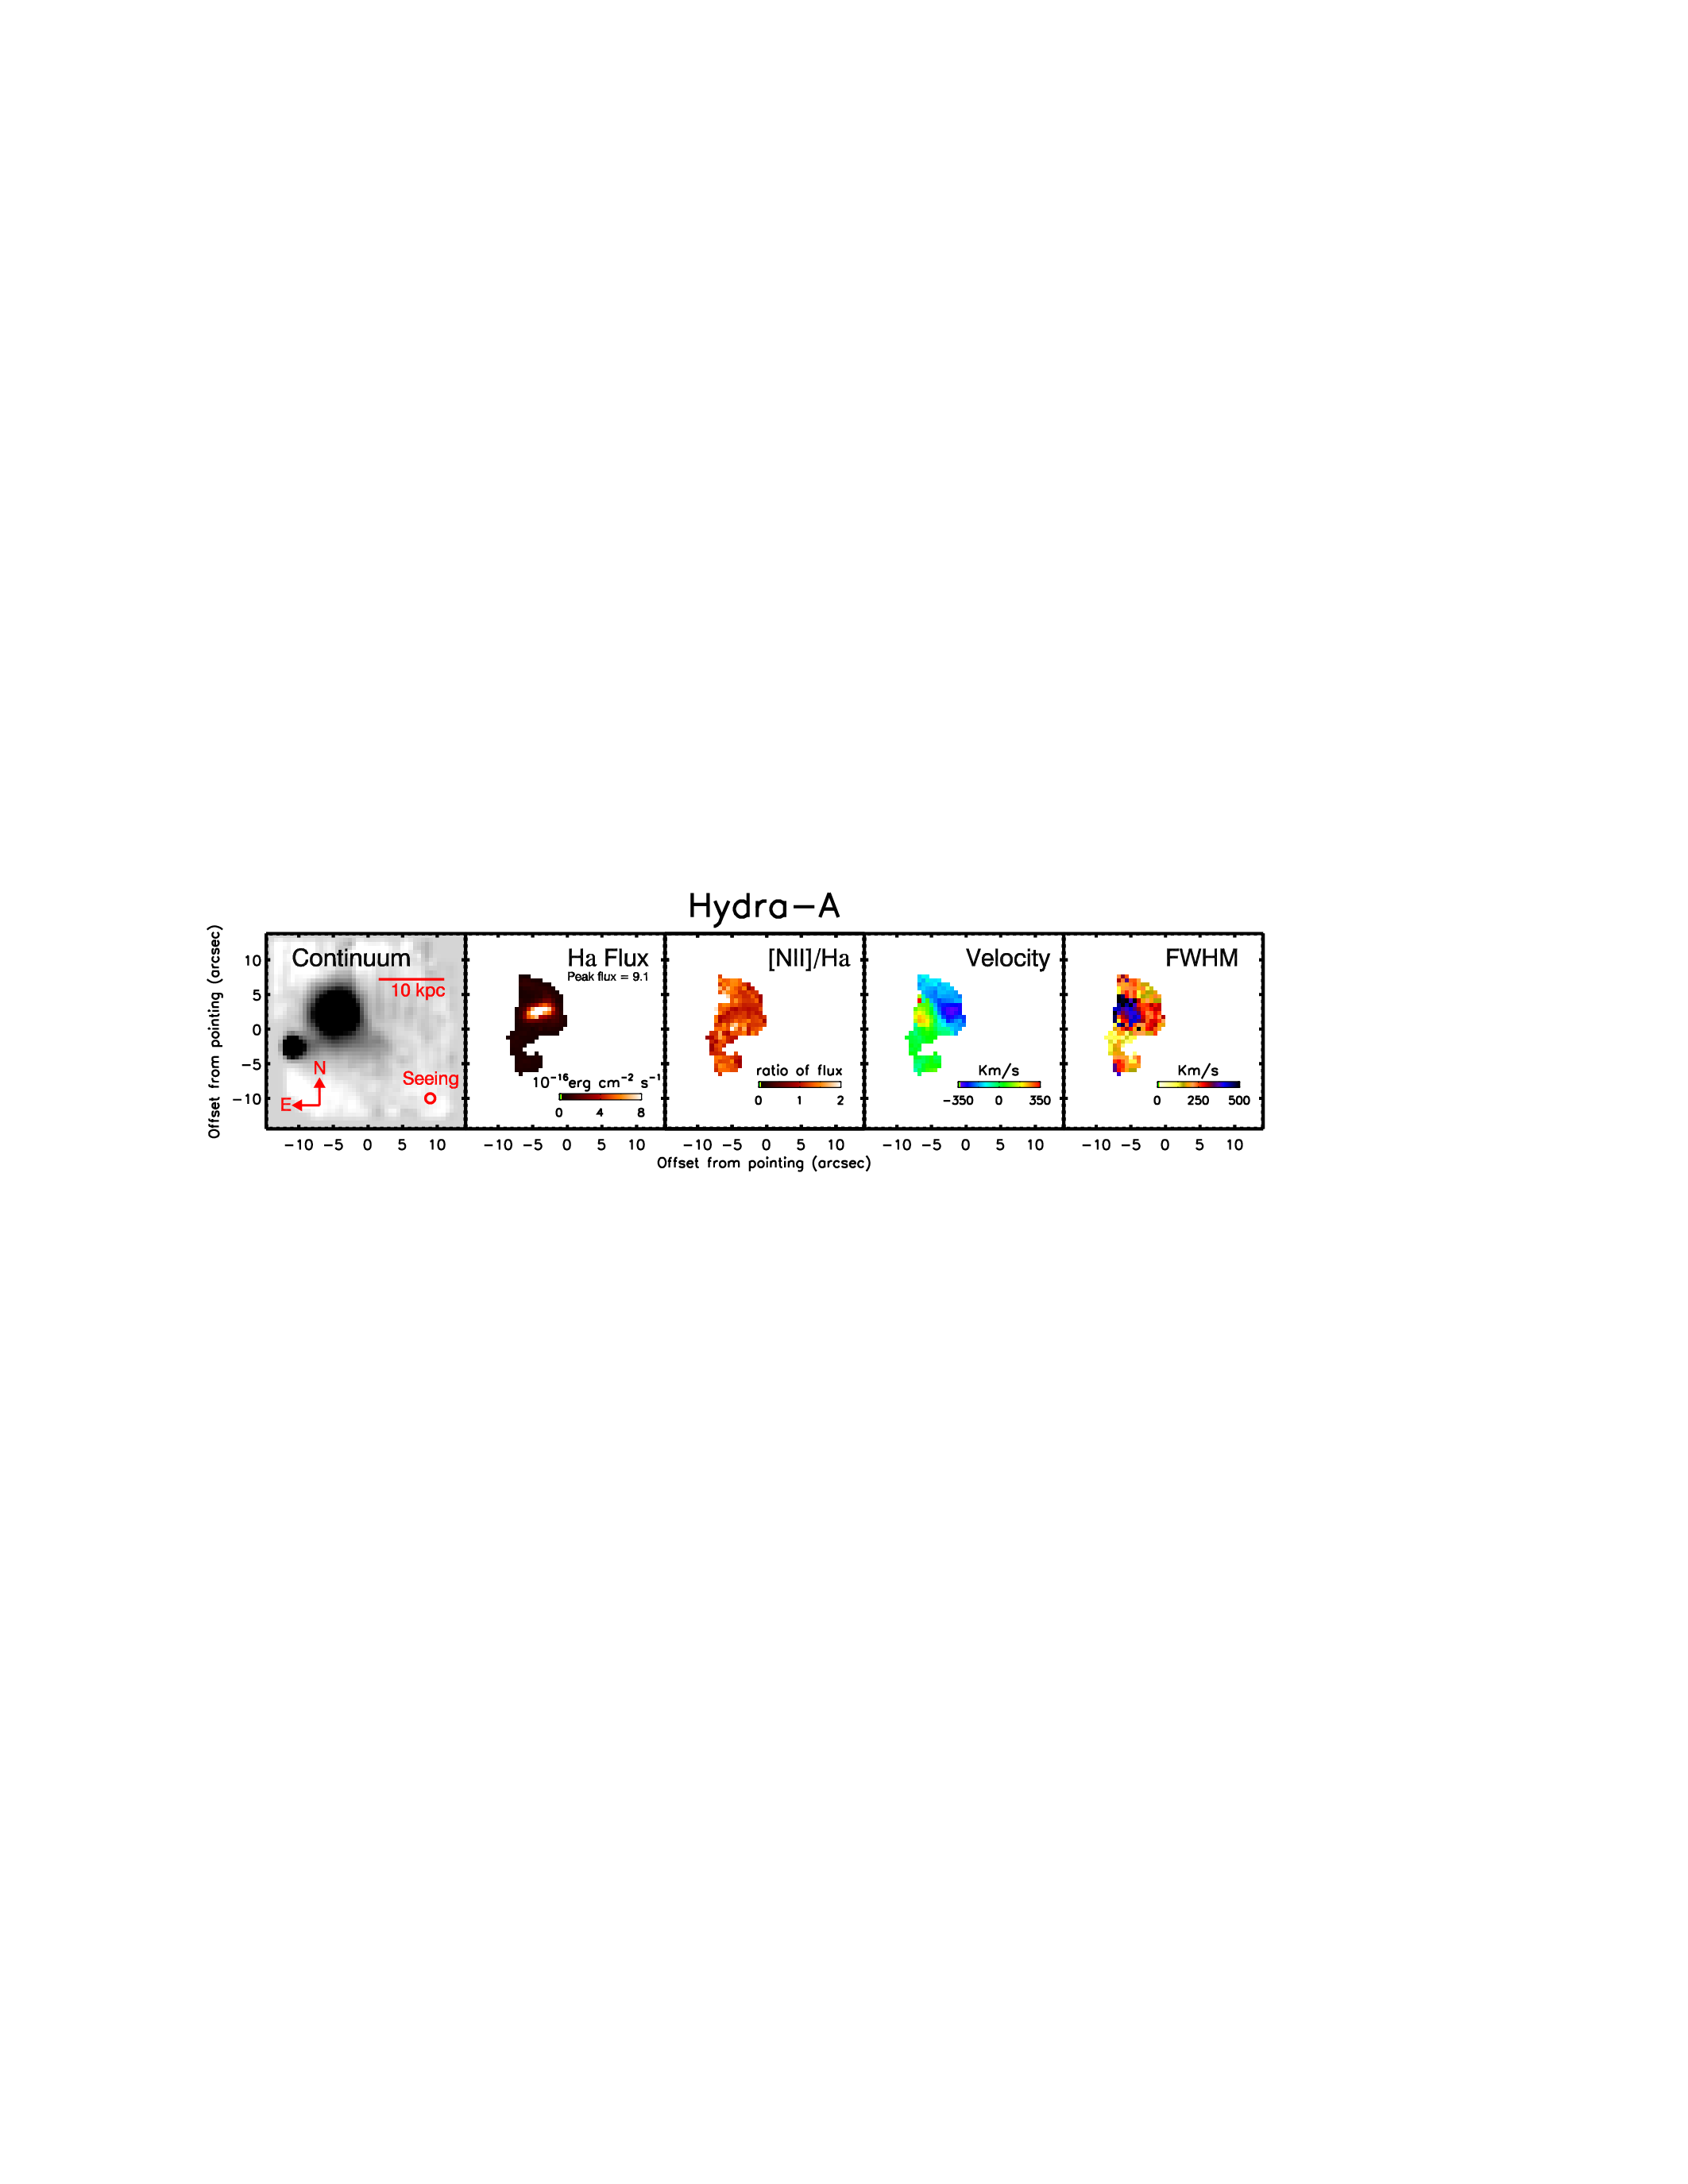}
\clearpage
\includegraphics[width=17cm,bbllx=74,bblly=367,bburx=459,bbury=470]{/media/stephen/HYDRA/Backup/Obs/lvjm32/Thesis/Thesistex/Chap3/Figs/NGC4325_plots.ps}

\includegraphics[width=17cm,bbllx=74,bblly=367,bburx=459,bbury=470]{/media/stephen/HYDRA/Backup/Obs/lvjm32/Thesis/Thesistex/Chap3/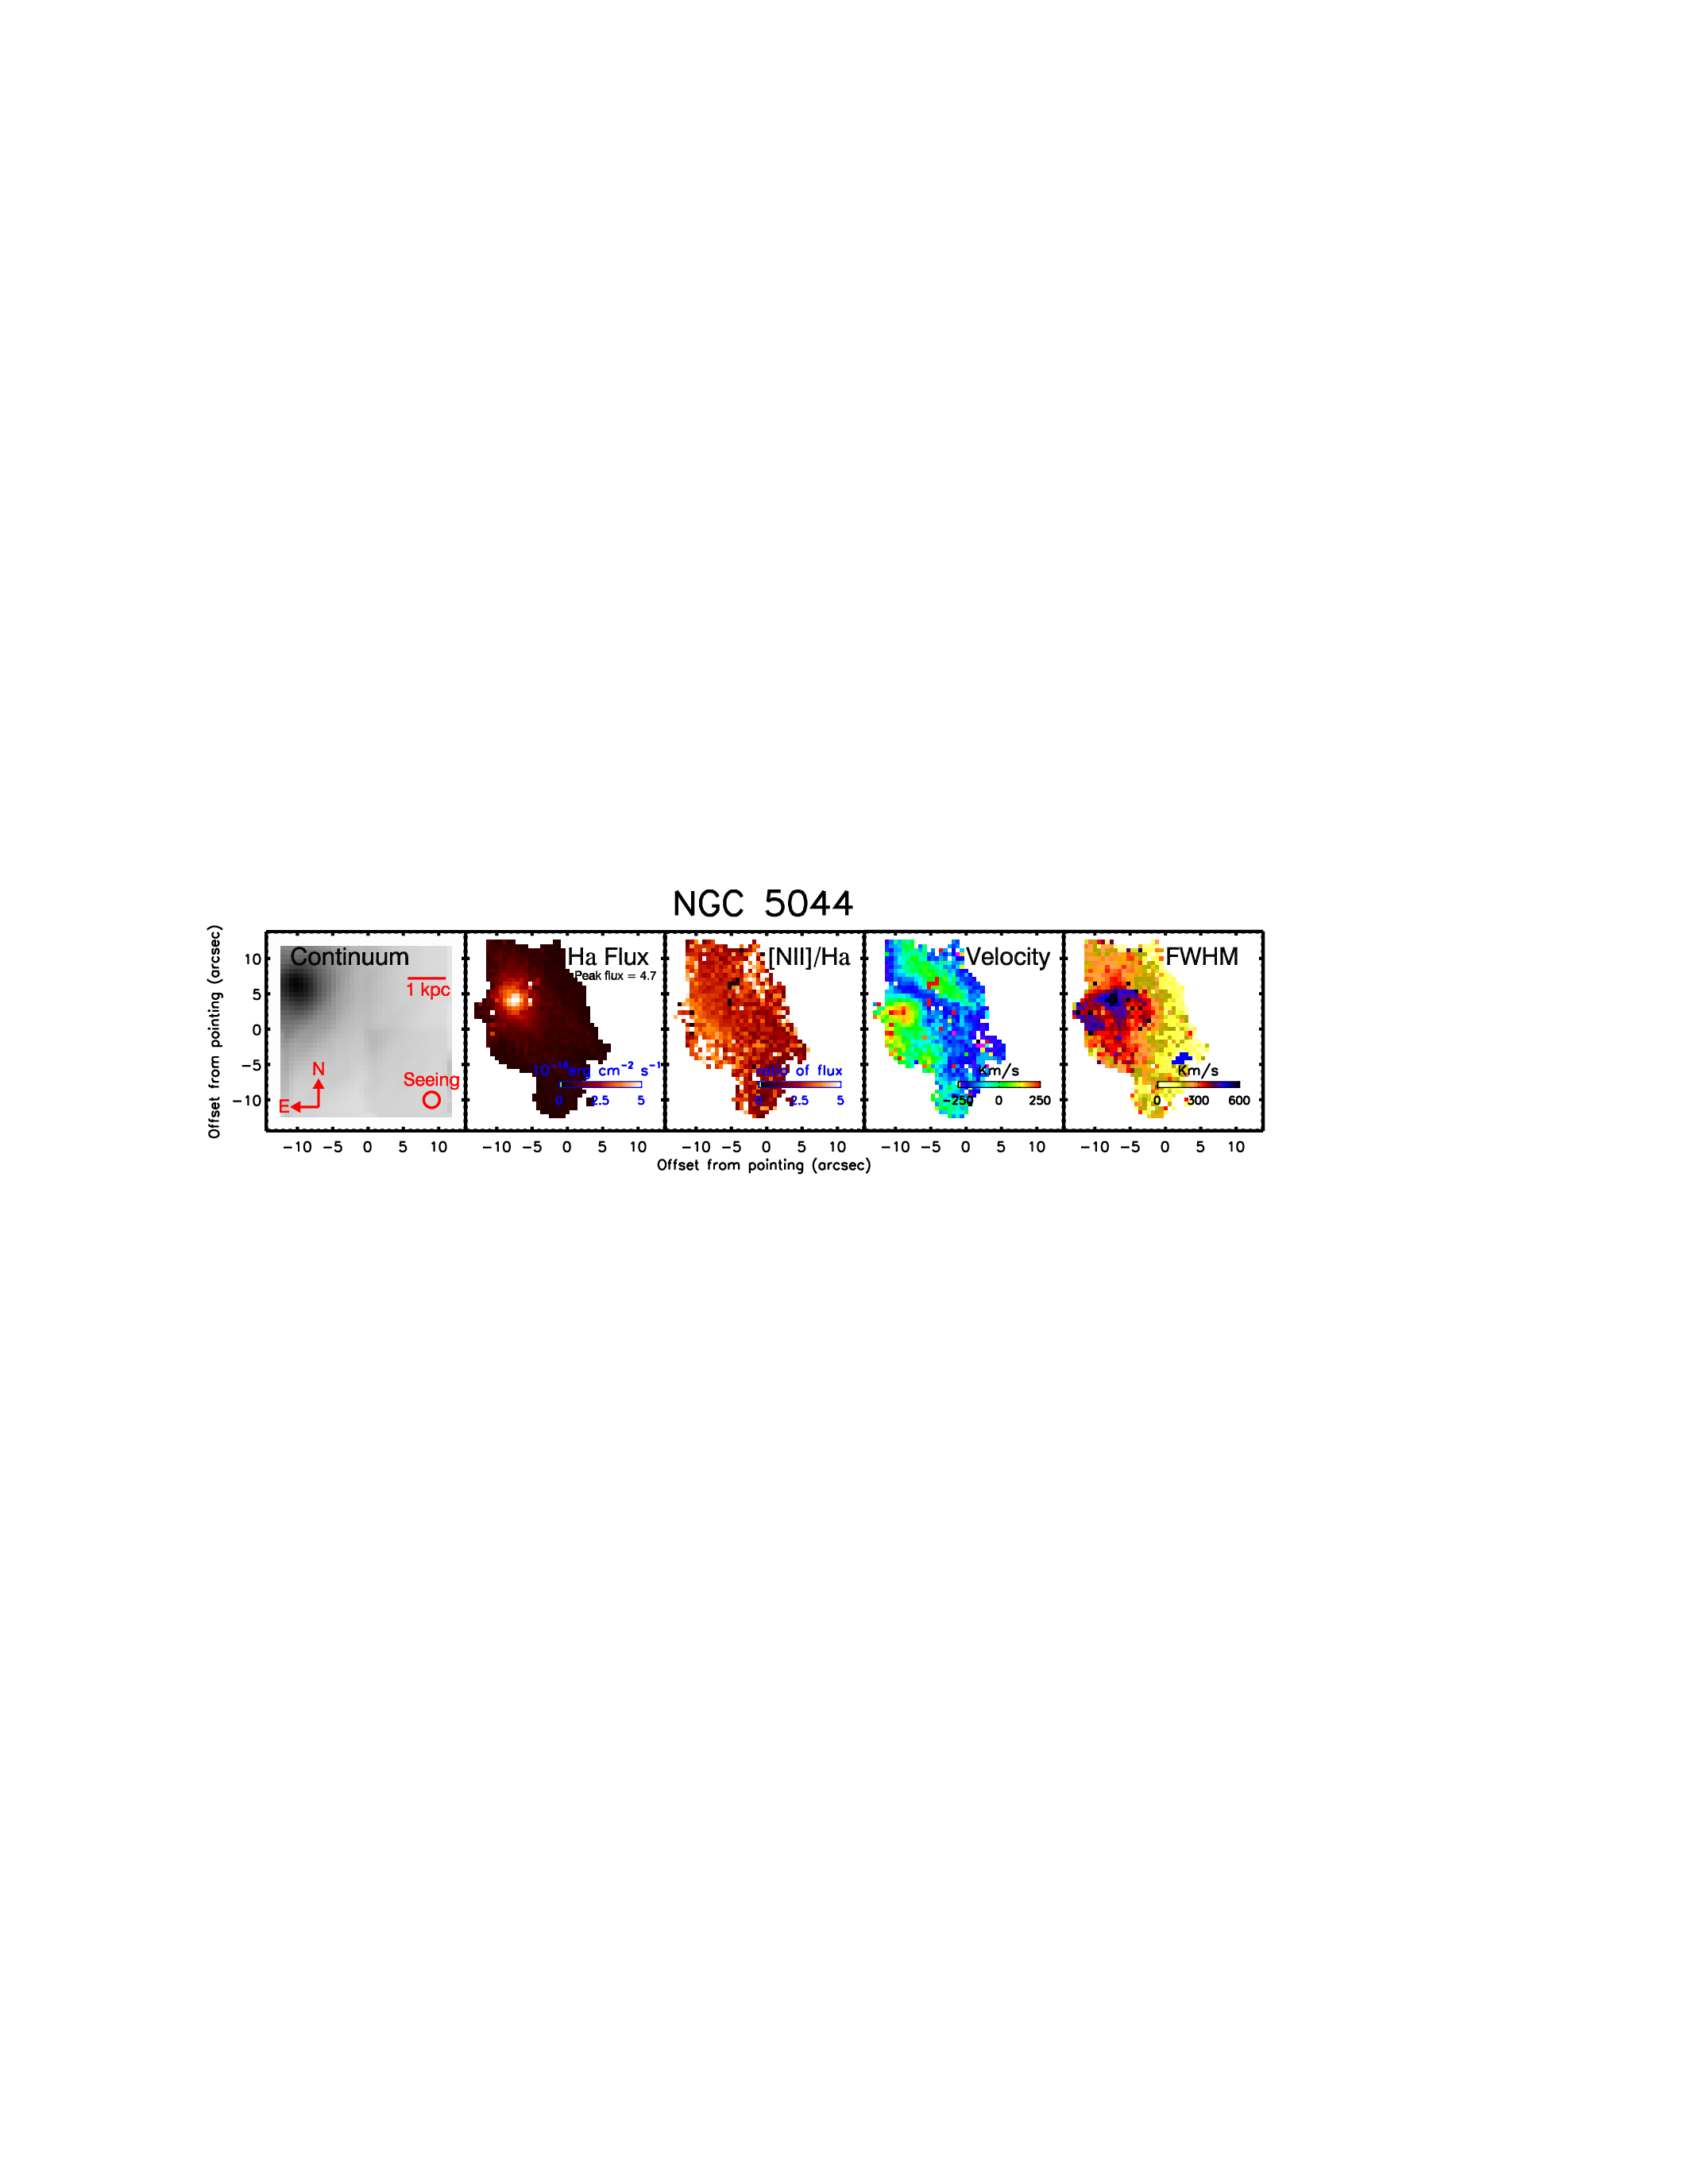}

\includegraphics[width=17cm,bbllx=74,bblly=367,bburx=459,bbury=470]{/media/stephen/HYDRA/Backup/Obs/lvjm32/Thesis/Thesistex/Chap3/Figs/NGC533_plots.ps}

\includegraphics[width=17cm,bbllx=74,bblly=367,bburx=459,bbury=470]{/media/stephen/HYDRA/Backup/Obs/lvjm32/Thesis/Thesistex/Chap3/Figs/NGC5813_plots.ps}

\includegraphics[width=17cm,bbllx=74,bblly=367,bburx=459,bbury=470]{/media/stephen/HYDRA/Backup/Obs/lvjm32/Thesis/Thesistex/Chap3/Figs/NGC5846_plots.ps}
\clearpage
\includegraphics[width=17cm,bbllx=74,bblly=367,bburx=459,bbury=470]{/media/stephen/HYDRA/Backup/Obs/lvjm32/Thesis/Thesistex/Chap3/Figs/RXCJ0120.9-1351_plots.ps}

\includegraphics[width=17cm,bbllx=74,bblly=367,bburx=459,bbury=470]{/media/stephen/HYDRA/Backup/Obs/lvjm32/Thesis/Thesistex/Chap3/Figs/RXCJ0132.6-0804_plots.ps}

\includegraphics[width=17cm,bbllx=74,bblly=367,bburx=459,bbury=470]{/media/stephen/HYDRA/Backup/Obs/lvjm32/Thesis/Thesistex/Chap3/Figs/RXCJ0331.1-2100_plots.ps}

\includegraphics[width=17cm,bbllx=74,bblly=367,bburx=459,bbury=470]{/media/stephen/HYDRA/Backup/Obs/lvjm32/Thesis/Thesistex/Chap3/Figs/RXCJ0543.4-4430_plots.ps}

\includegraphics[width=17cm,bbllx=74,bblly=367,bburx=459,bbury=470]{/media/stephen/HYDRA/Backup/Obs/lvjm32/Thesis/Thesistex/Chap3/Figs/RXCJ0944.6-2633_plots.ps}
\clearpage
\includegraphics[width=17cm,bbllx=74,bblly=367,bburx=459,bbury=470]{/media/stephen/HYDRA/Backup/Obs/lvjm32/Thesis/Thesistex/Chap3/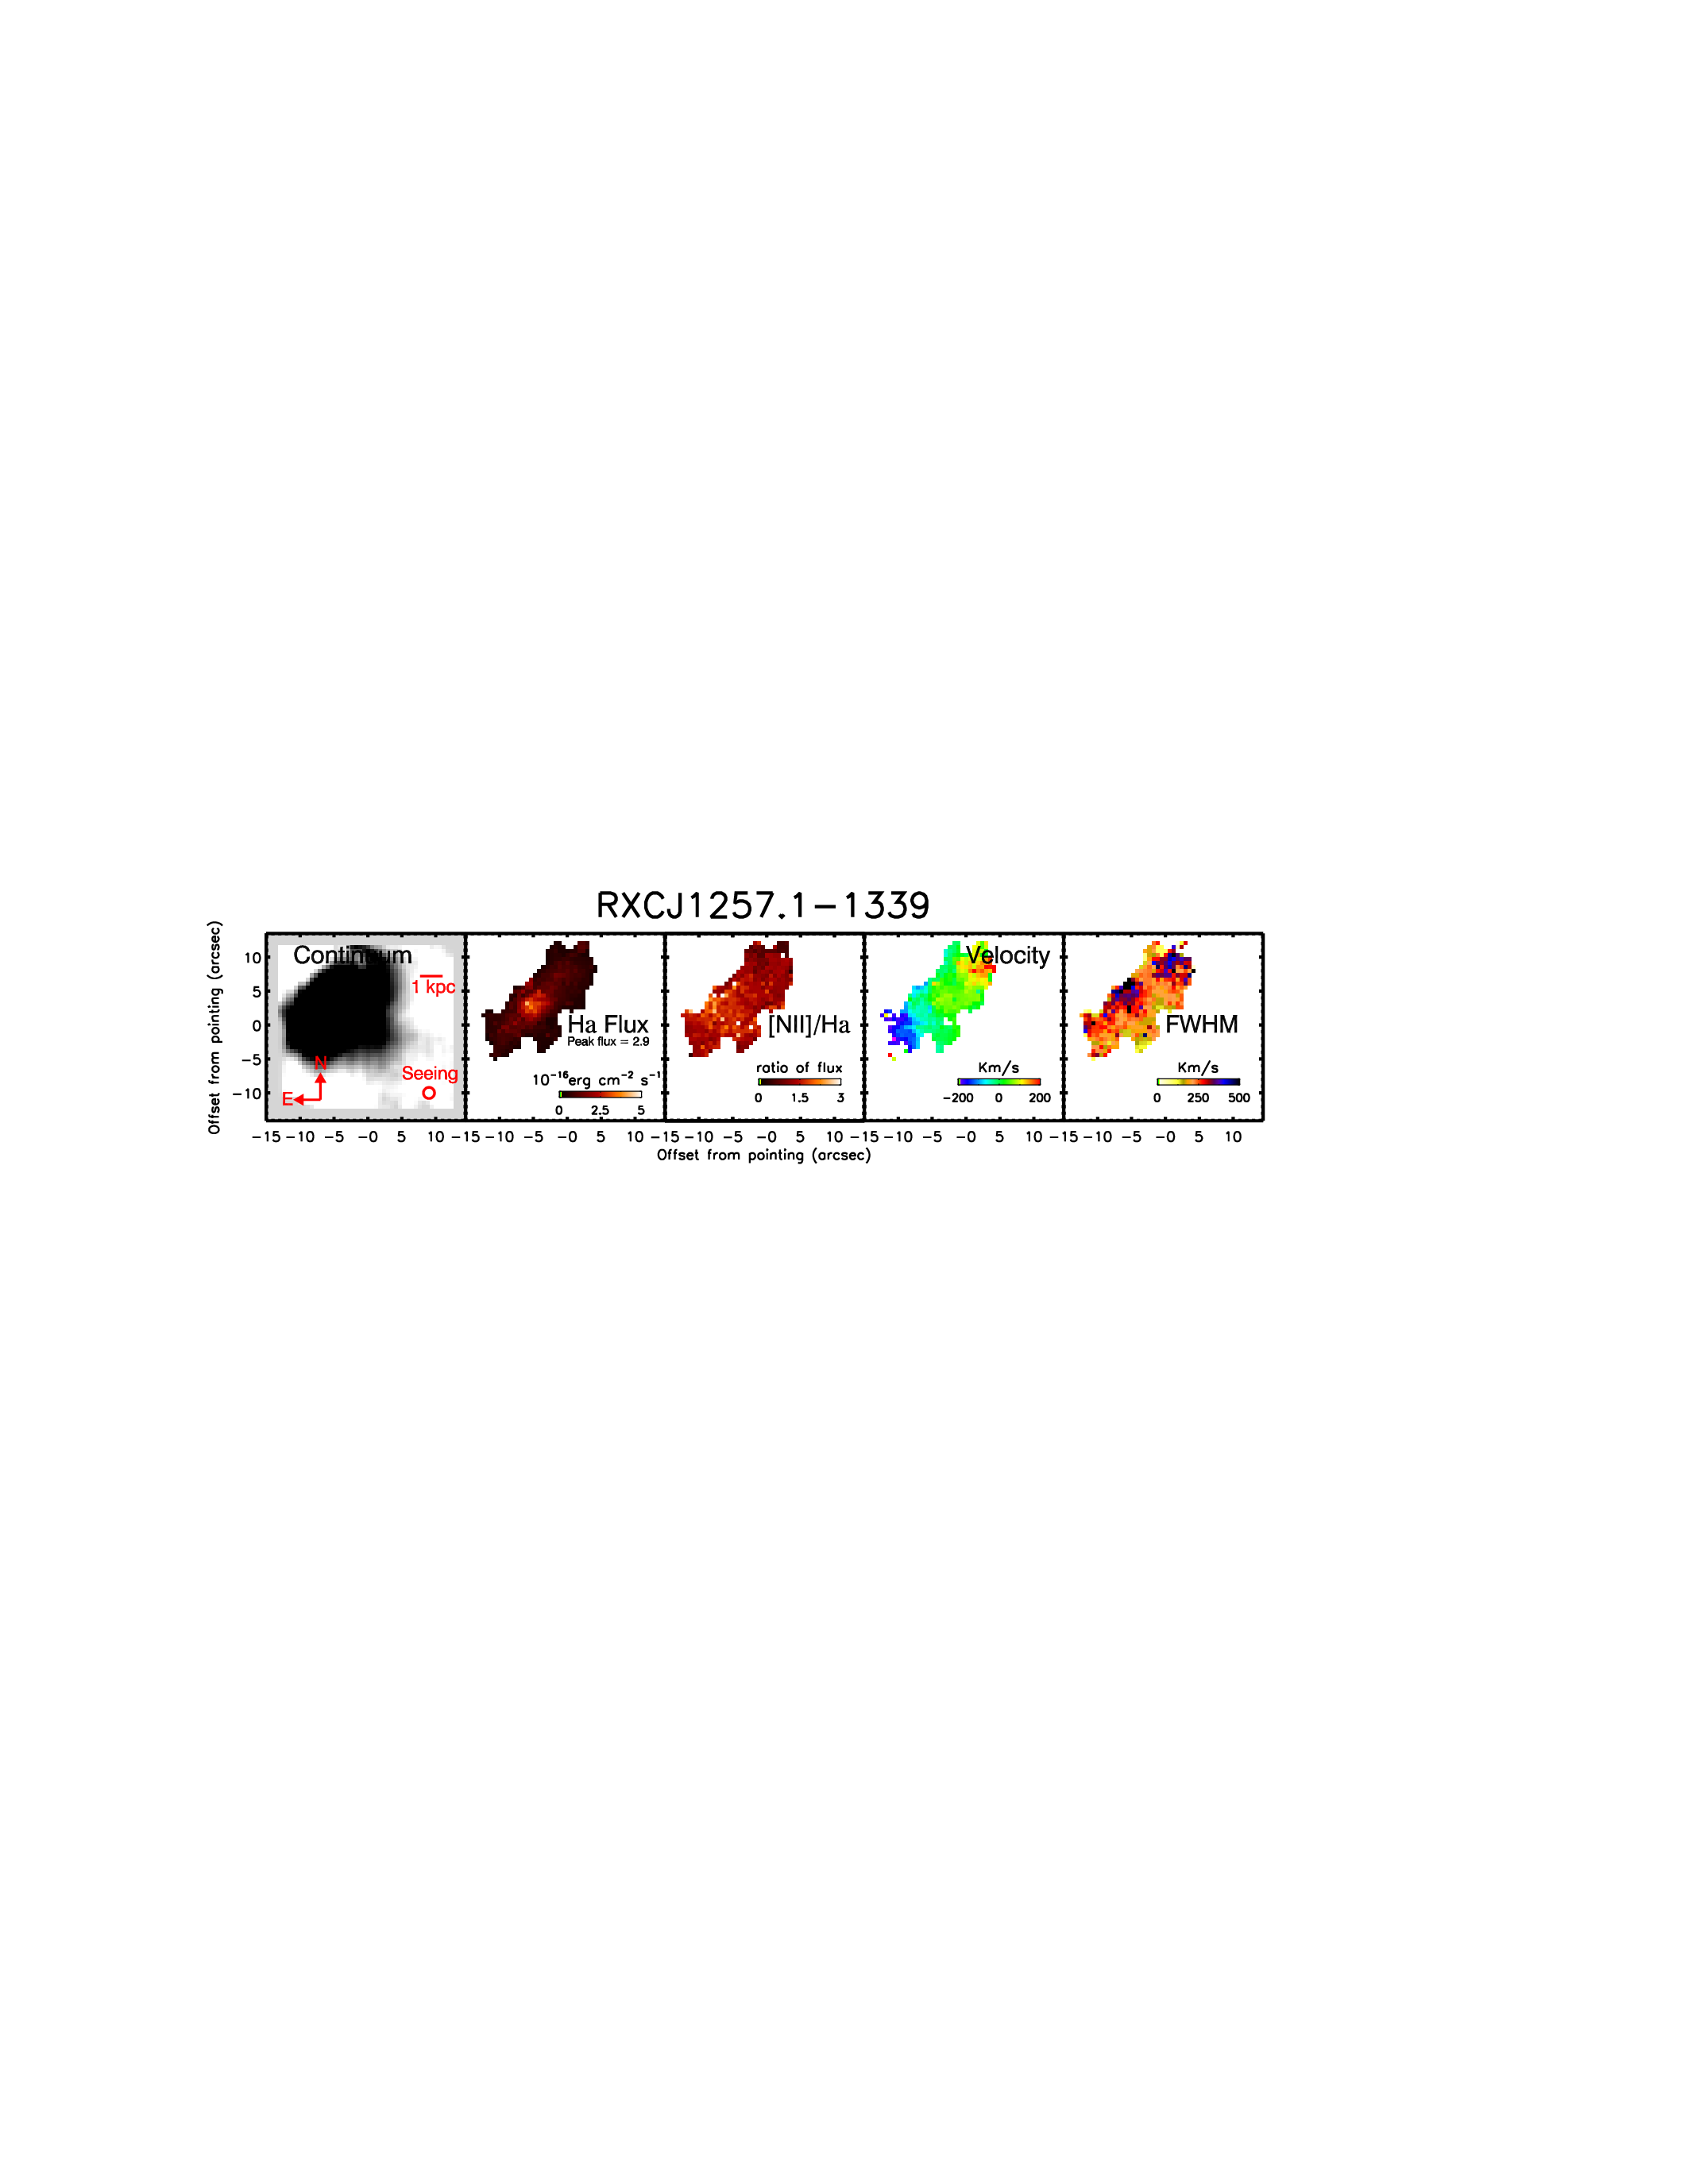}

\includegraphics[width=17cm,bbllx=74,bblly=367,bburx=459,bbury=470]{/media/stephen/HYDRA/Backup/Obs/lvjm32/Thesis/Thesistex/Chap3/Figs/RXCJ1304.2-3030_plots.ps}

\includegraphics[width=17cm,bbllx=74,bblly=367,bburx=459,bbury=470]{/media/stephen/HYDRA/Backup/Obs/lvjm32/Thesis/Thesistex/Chap3/Figs/RXCJ1436.8-0900_plots.ps}

\includegraphics[width=17cm,bbllx=74,bblly=367,bburx=459,bbury=470]{/media/stephen/HYDRA/Backup/Obs/lvjm32/Thesis/Thesistex/Chap3/Figs/RXCJ1511.5+0145_plots.ps}

\includegraphics[width=17cm,bbllx=74,bblly=367,bburx=459,bbury=470]{/media/stephen/HYDRA/Backup/Obs/lvjm32/Thesis/Thesistex/Chap3/Figs/RXCJ1524.2-3154_plots.ps}
\clearpage
\includegraphics[width=17cm,bbllx=74,bblly=367,bburx=459,bbury=470]{/media/stephen/HYDRA/Backup/Obs/lvjm32/Thesis/Thesistex/Chap3/Figs/RXCJ1539.5-8335_plots.ps}

\includegraphics[width=17cm,bbllx=74,bblly=367,bburx=459,bbury=470]{/media/stephen/HYDRA/Backup/Obs/lvjm32/Thesis/Thesistex/Chap3/Figs/RXCJ1558.3-1410_plots.ps}

\includegraphics[width=17cm,bbllx=74,bblly=367,bburx=459,bbury=470]{/media/stephen/HYDRA/Backup/Obs/lvjm32/Thesis/Thesistex/Chap3/Figs/RXCJ2014.8-2430_plots.ps}

\includegraphics[width=17cm,bbllx=74,bblly=367,bburx=459,bbury=470]{/media/stephen/HYDRA/Backup/Obs/lvjm32/Thesis/Thesistex/Chap3/Figs/RXCJ2101.8-2802_plots.ps}

\includegraphics[width=17cm,bbllx=74,bblly=367,bburx=459,bbury=470]{/media/stephen/HYDRA/Backup/Obs/lvjm32/Thesis/Thesistex/Chap3/Figs/RXCJ2129.6+0005_plots.ps}
\clearpage
\includegraphics[width=17cm,bbllx=74,bblly=367,bburx=459,bbury=470]{/media/stephen/HYDRA/Backup/Obs/lvjm32/Thesis/Thesistex/Chap3/Figs/RXCJ2213.0-2753_plots.ps}

\includegraphics[width=17cm,bbllx=74,bblly=367,bburx=459,bbury=470]{/media/stephen/HYDRA/Backup/Obs/lvjm32/Thesis/Thesistex/Chap3/Figs/RXJ0000.1+0816_plots.ps}

\includegraphics[width=17cm,bbllx=74,bblly=367,bburx=459,bbury=470]{/media/stephen/HYDRA/Backup/Obs/lvjm32/Thesis/Thesistex/Chap3/Figs/RXJ0338+09_plots.ps}

\includegraphics[width=17cm,bbllx=74,bblly=367,bburx=459,bbury=470]{/media/stephen/HYDRA/Backup/Obs/lvjm32/Thesis/Thesistex/Chap3/Figs/RXJ0352.9+1941_plots.ps}

\includegraphics[width=17cm,bbllx=74,bblly=367,bburx=459,bbury=470]{/media/stephen/HYDRA/Backup/Obs/lvjm32/Thesis/Thesistex/Chap3/Figs/RXJ0439.0+0520_plots.ps}
\clearpage
\includegraphics[width=17cm,bbllx=74,bblly=367,bburx=459,bbury=470]{/media/stephen/HYDRA/Backup/Obs/lvjm32/Thesis/Thesistex/Chap3/Figs/RXJ0747-19_plots.ps}

\includegraphics[width=17cm,bbllx=74,bblly=367,bburx=459,bbury=470]{/media/stephen/HYDRA/Backup/Obs/lvjm32/Thesis/Thesistex/Chap3/Figs/RXJ0821+07_plots.ps}

\includegraphics[width=17cm,bbllx=74,bblly=367,bburx=459,bbury=470]{/media/stephen/HYDRA/Backup/Obs/lvjm32/Thesis/Thesistex/Chap3/Figs/RXJ1651.1+0459_plots.ps}

\includegraphics[width=17cm,bbllx=74,bblly=367,bburx=459,bbury=470]{/media/stephen/HYDRA/Backup/Obs/lvjm32/Thesis/Thesistex/Chap3/Figs/S555_plots.ps}

\includegraphics[width=17cm,bbllx=74,bblly=367,bburx=459,bbury=470]{/media/stephen/HYDRA/Backup/Obs/lvjm32/Thesis/Thesistex/Chap3/Figs/S780_plots.ps}
\clearpage
\includegraphics[width=17cm,bbllx=74,bblly=367,bburx=459,bbury=470]{/media/stephen/HYDRA/Backup/Obs/lvjm32/Thesis/Thesistex/Chap3/Figs/S805_plots.ps}

\includegraphics[width=17cm,bbllx=74,bblly=367,bburx=459,bbury=470]{/media/stephen/HYDRA/Backup/Obs/lvjm32/Thesis/Thesistex/Chap3/Figs/S851_plots.ps}

\includegraphics[width=17cm,bbllx=74,bblly=367,bburx=459,bbury=470]{/media/stephen/HYDRA/Backup/Obs/lvjm32/Thesis/Thesistex/Chap3/Figs/Z3179_plots.ps}

\includegraphics[width=17cm,bbllx=74,bblly=367,bburx=459,bbury=470]{/media/stephen/HYDRA/Backup/Obs/lvjm32/Thesis/Thesistex/Chap3/Figs/Z348_plots.ps}

%Appendix D-------------------------------------------------------------------------------
\clearpage
\onecolumn
%\thispagestyle{headings}
%\mbox{}
\section{Maps comparing the stellar absorption to the H$\alpha$ emission}
\label{app:NaD}

\begin{figure}
\psfig{figure=/media/stephen/HYDRA/Backup/Obs/lvjm32/Vimos-ifu/Lowz/A1348/Abell1348_abs_plots2.ps,width=15cm,bbllx=50,bblly=350,bburx=470,bbury=640}
\psfig{figure=/media/stephen/HYDRA/Backup/Obs/lvjm32/Vimos-ifu/Lowz/A194/Abell194_abs_plots2.ps,width=15cm,bbllx=50,bblly=350,bburx=470,bbury=640}
\caption[Stellar absorption and kinematics extracting from objects in which the continuum was bright enough to fit the sodium D feature]{Here we show the stellar absorption and kinematics of each object from the sample in which the continuum was bright enough to allow the sodium D absorption feature to be fitted accurately.  Fits to the H$\alpha$ emission are included for comparison and the contrast in the mean velocity fields is very apparent clearly suggesting that the motion of the gas is decoupled from that of the stars.} 
\label{fig:absmaps}
\end{figure}

%\pagebreak
\vspace{3cm}
\begin{figure}
\ContinuedFloat
\psfig{figure=/media/stephen/HYDRA/Backup/Obs/lvjm32/Vimos-ifu/Lowz/A1991-added/Abell1991_abs_plots2.ps,width=15cm,bbllx=50,bblly=350,bburx=470,bbury=690}
\psfig{figure=/media/stephen/HYDRA/Backup/Obs/lvjm32/Vimos-ifu/Lowz/HCG62/HCG62_abs_plots2.ps,width=15cm,bbllx=50,bblly=350,bburx=470,bbury=640}
\caption[]{continued.} 
%\label{fig:lumkpcvel}
\end{figure}

\begin{figure}
\ContinuedFloat
\psfig{figure=/media/stephen/HYDRA/Backup/Obs/lvjm32/Vimos-ifu/Lowz/Hydra-a/Hydra-A_abs_plots2.ps,width=15cm,bbllx=50,bblly=350,bburx=470,bbury=640}
\psfig{figure=/media/stephen/HYDRA/Backup/Obs/lvjm32/Vimos-ifu/Lowz/NGC4325/NGC4325_abs_plots2.ps,width=15cm,bbllx=50,bblly=350,bburx=470,bbury=640}
\caption[]{continued.} 
%\label{fig:lumkpcvel}
\end{figure}

\begin{figure}
\ContinuedFloat
\psfig{figure=/media/stephen/HYDRA/Backup/Obs/lvjm32/Vimos-ifu/Lowz/NGC533/NGC533_abs_plots2.ps,width=15cm,bbllx=50,bblly=350,bburx=470,bbury=640}
\psfig{figure=/media/stephen/HYDRA/Backup/Obs/lvjm32/Vimos-ifu/Lowz/RXCJ0120.9-1351/RXCJ0120.9-1351_abs_plots2.ps,width=15cm,bbllx=50,bblly=350,bburx=470,bbury=640}
\caption[]{continued.} 
%\label{fig:lumkpcvel}
\end{figure}

\begin{figure}
\ContinuedFloat
\psfig{figure=/media/stephen/HYDRA/Backup/Obs/lvjm32/Vimos-ifu/Lowz/RXCJ1257.1-1339/RXCJ1257.1-1339_abs_plots2.ps,width=15cm,bbllx=50,bblly=350,bburx=470,bbury=640}
\psfig{figure=/media/stephen/HYDRA/Backup/Obs/lvjm32/Vimos-ifu/Lowz/RXCJ1304.2-3030/RXCJ1304.2-3030_abs_plots2.ps,width=15cm,bbllx=50,bblly=350,bburx=470,bbury=640}
\caption[]{continued.} 
%\label{fig:lumkpcvel}
\end{figure}

\begin{figure}
\ContinuedFloat
\psfig{figure=/media/stephen/HYDRA/Backup/Obs/lvjm32/Vimos-ifu/Lowz/RXJ0338+09/RXJ0338+09_abs_plots2.ps,width=15cm,bbllx=50,bblly=350,bburx=470,bbury=640}
\psfig{figure=/media/stephen/HYDRA/Backup/Obs/lvjm32/Vimos-ifu/Lowz/S851/S851_abs_plots2.ps,width=15cm,bbllx=50,bblly=350,bburx=470,bbury=640}
\caption[]{continued.} 
%\label{fig:lumkpcvel}
\end{figure}

%Appendix E-----------------------------------------------------------------------------

\clearpage
\onecolumn
%\thispagestyle{headings}
%\mbox{}
\section{Extracted spectra}
\label{app:specs}

\begin{figure}
\psfig{figure=/media/stephen/HYDRA/Backup/Obs/lvjm32/Vimos-ifu/Totspecs/Specs2/A1060_fullspec.ps,width=8cm,bbllx=74,bblly=367,bburx=450,bbury=549} 
\psfig{figure=/media/stephen/HYDRA/Backup/Obs/lvjm32/Vimos-ifu/Totspecs/Specs2/A1084_fullspec.ps,width=8cm,bbllx=74,bblly=367,bburx=450,bbury=549} 
\psfig{figure=/media/stephen/HYDRA/Backup/Obs/lvjm32/Vimos-ifu/Totspecs/Specs2/A11_fullspec.ps,width=8cm,bbllx=74,bblly=367,bburx=450,bbury=549} 
\psfig{figure=/media/stephen/HYDRA/Backup/Obs/lvjm32/Vimos-ifu/Totspecs/Specs2/A1111_fullspec.ps,width=8cm,bbllx=74,bblly=367,bburx=450,bbury=549} 
\psfig{figure=/media/stephen/HYDRA/Backup/Obs/lvjm32/Vimos-ifu/Totspecs/Specs2/A1204_fullspec.ps,width=8cm,bbllx=74,bblly=367,bburx=450,bbury=549} 
\psfig{figure=/media/stephen/HYDRA/Backup/Obs/lvjm32/Vimos-ifu/Totspecs/Specs2/A133_fullspec.ps,width=8cm,bbllx=74,bblly=367,bburx=450,bbury=549} 
\psfig{figure=/media/stephen/HYDRA/Backup/Obs/lvjm32/Vimos-ifu/Totspecs/Specs2/A1348_fullspec.ps,width=8cm,bbllx=74,bblly=367,bburx=450,bbury=549} 
\psfig{figure=/media/stephen/HYDRA/Backup/Obs/lvjm32/Vimos-ifu/Totspecs/Specs2/A1663_fullspec.ps,width=8cm,bbllx=74,bblly=367,bburx=450,bbury=549}  
\psfig{figure=/media/stephen/HYDRA/Backup/Obs/lvjm32/Vimos-ifu/Totspecs/Specs2/A1668_fullspec.ps,width=8cm,bbllx=74,bblly=367,bburx=450,bbury=549}  
\hspace{1.5cm}           
\psfig{figure=/media/stephen/HYDRA/Backup/Obs/lvjm32/Vimos-ifu/Totspecs/Specs2/A194_fullspec.ps,width=8cm,bbllx=74,bblly=367,bburx=450,bbury=549} 
\caption{Here we display the spectra of each object in the sample.  Each object is displayed in a separate panel and has two spectra; {\em Top - }The total spectrum of the line emitting region;  {\em Bottom - }Spectrum of the 2 $\times$ 2 arcsec$^2$ region centred on the brightest point of the BCG in its continuum light.   Each spectrum has had the sky removed, cosmic ray events eliminated, and has been continuum subtracted.  The spectra are presented at the rest wavelength of the line emission as given in table \ref{tab:sam1} between 6200 and 6800 \AA.}
\label{fig:spec}
\end{figure}

\clearpage

\begin{figure}
\ContinuedFloat
\psfig{figure=/media/stephen/HYDRA/Backup/Obs/lvjm32/Vimos-ifu/Totspecs/Specs2/A1991-added_fullspec.ps,width=8cm,bbllx=74,bblly=367,bburx=450,bbury=549} 
\psfig{figure=/media/stephen/HYDRA/Backup/Obs/lvjm32/Vimos-ifu/Totspecs/Specs2/A2052_fullspec.ps,width=8cm,bbllx=74,bblly=367,bburx=450,bbury=549} 
\psfig{figure=/media/stephen/HYDRA/Backup/Obs/lvjm32/Vimos-ifu/Totspecs/Specs2/A2390_fullspec.ps,width=8cm,bbllx=74,bblly=367,bburx=450,bbury=549} 
\psfig{figure=/media/stephen/HYDRA/Backup/Obs/lvjm32/Vimos-ifu/Totspecs/Specs2/A2415_fullspec.ps,width=8cm,bbllx=74,bblly=367,bburx=450,bbury=549} 
\psfig{figure=/media/stephen/HYDRA/Backup/Obs/lvjm32/Vimos-ifu/Totspecs/Specs2/A2495_fullspec.ps,width=8cm,bbllx=74,bblly=367,bburx=450,bbury=549} 
\psfig{figure=/media/stephen/HYDRA/Backup/Obs/lvjm32/Vimos-ifu/Totspecs/Specs2/A2566_fullspec.ps,width=8cm,bbllx=74,bblly=367,bburx=450,bbury=549} 
\psfig{figure=/media/stephen/HYDRA/Backup/Obs/lvjm32/Vimos-ifu/Totspecs/Specs2/A2580_fullspec.ps,width=8cm,bbllx=74,bblly=367,bburx=450,bbury=549} 
\psfig{figure=/media/stephen/HYDRA/Backup/Obs/lvjm32/Vimos-ifu/Totspecs/Specs2/A2734_fullspec.ps,width=8cm,bbllx=74,bblly=367,bburx=450,bbury=549}  
\psfig{figure=/media/stephen/HYDRA/Backup/Obs/lvjm32/Vimos-ifu/Totspecs/Specs2/A291_fullspec.ps,width=8cm,bbllx=74,bblly=367,bburx=450,bbury=549}  
\psfig{figure=/media/stephen/HYDRA/Backup/Obs/lvjm32/Vimos-ifu/Totspecs/Specs2/A3017_fullspec.ps,width=8cm,bbllx=74,bblly=367,bburx=450,bbury=549}  
\psfig{figure=/media/stephen/HYDRA/Backup/Obs/lvjm32/Vimos-ifu/Totspecs/Specs2/A3112_fullspec.ps,width=8cm,bbllx=74,bblly=367,bburx=450,bbury=549}   
\hspace{1.5cm}           
\psfig{figure=/media/stephen/HYDRA/Backup/Obs/lvjm32/Vimos-ifu/Totspecs/Specs2/A3378_fullspec.ps,width=8cm,bbllx=74,bblly=367,bburx=450,bbury=549} 
\caption{continued.}
%\label{fig:spec}
\end{figure}

\FloatBarrier

\begin{figure}
\ContinuedFloat
\psfig{figure=/media/stephen/HYDRA/Backup/Obs/lvjm32/Vimos-ifu/Totspecs/Specs2/A3444_fullspec.ps,width=8cm,bbllx=74,bblly=367,bburx=450,bbury=549} 
\psfig{figure=/media/stephen/HYDRA/Backup/Obs/lvjm32/Vimos-ifu/Totspecs/Specs2/A3574_fullspec.ps,width=8cm,bbllx=74,bblly=367,bburx=450,bbury=549} 
\psfig{figure=/media/stephen/HYDRA/Backup/Obs/lvjm32/Vimos-ifu/Totspecs/Specs2/A3581_fullspec.ps,width=8cm,bbllx=74,bblly=367,bburx=450,bbury=549} 
\psfig{figure=/media/stephen/HYDRA/Backup/Obs/lvjm32/Vimos-ifu/Totspecs/Specs2/A3605_fullspec.ps,width=8cm,bbllx=74,bblly=367,bburx=450,bbury=549} 
\psfig{figure=/media/stephen/HYDRA/Backup/Obs/lvjm32/Vimos-ifu/Totspecs/Specs2/A3638_fullspec.ps,width=8cm,bbllx=74,bblly=367,bburx=450,bbury=549} 
\psfig{figure=/media/stephen/HYDRA/Backup/Obs/lvjm32/Vimos-ifu/Totspecs/Specs2/A3639_fullspec.ps,width=8cm,bbllx=74,bblly=367,bburx=450,bbury=549} 
\psfig{figure=/media/stephen/HYDRA/Backup/Obs/lvjm32/Vimos-ifu/Totspecs/Specs2/A3806_fullspec.ps,width=8cm,bbllx=74,bblly=367,bburx=450,bbury=549} 
\psfig{figure=/media/stephen/HYDRA/Backup/Obs/lvjm32/Vimos-ifu/Totspecs/Specs2/A383_fullspec.ps,width=8cm,bbllx=74,bblly=367,bburx=450,bbury=549}  
\psfig{figure=/media/stephen/HYDRA/Backup/Obs/lvjm32/Vimos-ifu/Totspecs/Specs2/A3880_fullspec.ps,width=8cm,bbllx=74,bblly=367,bburx=450,bbury=549}  
\psfig{figure=/media/stephen/HYDRA/Backup/Obs/lvjm32/Vimos-ifu/Totspecs/Specs2/A3998_fullspec.ps,width=8cm,bbllx=74,bblly=367,bburx=450,bbury=549}  
\psfig{figure=/media/stephen/HYDRA/Backup/Obs/lvjm32/Vimos-ifu/Totspecs/Specs2/A4059_fullspec.ps,width=8cm,bbllx=74,bblly=367,bburx=450,bbury=549}   
\hspace{1.5cm}           
\psfig{figure=/media/stephen/HYDRA/Backup/Obs/lvjm32/Vimos-ifu/Totspecs/Specs2/A478_fullspec.ps,width=8cm,bbllx=74,bblly=367,bburx=450,bbury=549} 
\caption{continued.}
%\label{fig:spec}
\end{figure}

\FloatBarrier

\begin{figure}
\ContinuedFloat
\psfig{figure=/media/stephen/HYDRA/Backup/Obs/lvjm32/Vimos-ifu/Totspecs/Specs2/A496_fullspec.ps,width=8cm,bbllx=74,bblly=367,bburx=450,bbury=549} 
\psfig{figure=/media/stephen/HYDRA/Backup/Obs/lvjm32/Vimos-ifu/Totspecs/Specs2/A85_fullspec.ps,width=8cm,bbllx=74,bblly=367,bburx=450,bbury=549} 
\psfig{figure=/media/stephen/HYDRA/Backup/Obs/lvjm32/Vimos-ifu/Totspecs/Specs2/HCG62_fullspec.ps,width=8cm,bbllx=74,bblly=367,bburx=450,bbury=549} 
\psfig{figure=/media/stephen/HYDRA/Backup/Obs/lvjm32/Vimos-ifu/Totspecs/Specs2/Hydra-a_fullspec.ps,width=8cm,bbllx=74,bblly=367,bburx=450,bbury=549} 
\psfig{figure=/media/stephen/HYDRA/Backup/Obs/lvjm32/Vimos-ifu/Totspecs/Specs2/NGC4325_fullspec.ps,width=8cm,bbllx=74,bblly=367,bburx=450,bbury=549} 
\psfig{figure=/media/stephen/HYDRA/Backup/Obs/lvjm32/Vimos-ifu/Totspecs/Specs2/NGC5044_fullspec.ps,width=8cm,bbllx=74,bblly=367,bburx=450,bbury=549} 
\psfig{figure=/media/stephen/HYDRA/Backup/Obs/lvjm32/Vimos-ifu/Totspecs/Specs2/NGC533_fullspec.ps,width=8cm,bbllx=74,bblly=367,bburx=450,bbury=549} 
\psfig{figure=/media/stephen/HYDRA/Backup/Obs/lvjm32/Vimos-ifu/Totspecs/Specs2/NGC5813_fullspec.ps,width=8cm,bbllx=74,bblly=367,bburx=450,bbury=549}  
\psfig{figure=/media/stephen/HYDRA/Backup/Obs/lvjm32/Vimos-ifu/Totspecs/Specs2/NGC5846_fullspec.ps,width=8cm,bbllx=74,bblly=367,bburx=450,bbury=549}  
\psfig{figure=/media/stephen/HYDRA/Backup/Obs/lvjm32/Vimos-ifu/Totspecs/Specs2/RXCJ0120.9-1351_fullspec.ps,width=8cm,bbllx=74,bblly=367,bburx=450,bbury=549}  
\psfig{figure=/media/stephen/HYDRA/Backup/Obs/lvjm32/Vimos-ifu/Totspecs/Specs2/RXCJ0132.6-0804_fullspec.ps,width=8cm,bbllx=74,bblly=367,bburx=450,bbury=549}  
\hspace{1.5cm}            
\psfig{figure=/media/stephen/HYDRA/Backup/Obs/lvjm32/Vimos-ifu/Totspecs/Specs2/RXCJ0331.1-2100_fullspec.ps,width=8cm,bbllx=74,bblly=367,bburx=450,bbury=549} 
\caption{continued.}
%\label{fig:spec}
\end{figure}

\FloatBarrier

\begin{figure}
\ContinuedFloat
\psfig{figure=/media/stephen/HYDRA/Backup/Obs/lvjm32/Vimos-ifu/Totspecs/Specs2/RXCJ0543.4-4430_fullspec.ps,width=8cm,bbllx=74,bblly=367,bburx=450,bbury=549} 
\psfig{figure=/media/stephen/HYDRA/Backup/Obs/lvjm32/Vimos-ifu/Totspecs/Specs2/RXCJ0944.6-2633_fullspec.ps,width=8cm,bbllx=74,bblly=367,bburx=450,bbury=549} 
\psfig{figure=/media/stephen/HYDRA/Backup/Obs/lvjm32/Vimos-ifu/Totspecs/Specs2/RXCJ1257.1-1339_fullspec.ps,width=8cm,bbllx=74,bblly=367,bburx=450,bbury=549} 
\psfig{figure=/media/stephen/HYDRA/Backup/Obs/lvjm32/Vimos-ifu/Totspecs/Specs2/RXCJ1304.2-3030_fullspec.ps,width=8cm,bbllx=74,bblly=367,bburx=450,bbury=549} 
\psfig{figure=/media/stephen/HYDRA/Backup/Obs/lvjm32/Vimos-ifu/Totspecs/Specs2/RXCJ1436.8-0900_fullspec.ps,width=8cm,bbllx=74,bblly=367,bburx=450,bbury=549} 
\psfig{figure=/media/stephen/HYDRA/Backup/Obs/lvjm32/Vimos-ifu/Totspecs/Specs2/RXCJ1511.5+0145_fullspec.ps,width=8cm,bbllx=74,bblly=367,bburx=450,bbury=549} 
\psfig{figure=/media/stephen/HYDRA/Backup/Obs/lvjm32/Vimos-ifu/Totspecs/Specs2/RXCJ1524.2-3154_fullspec.ps,width=8cm,bbllx=74,bblly=367,bburx=450,bbury=549} 
\psfig{figure=/media/stephen/HYDRA/Backup/Obs/lvjm32/Vimos-ifu/Totspecs/Specs2/RXCJ1539.5-8335_fullspec.ps,width=8cm,bbllx=74,bblly=367,bburx=450,bbury=549}  
\psfig{figure=/media/stephen/HYDRA/Backup/Obs/lvjm32/Vimos-ifu/Totspecs/Specs2/RXCJ1558.3-1410_fullspec.ps,width=8cm,bbllx=74,bblly=367,bburx=450,bbury=549}  
\psfig{figure=/media/stephen/HYDRA/Backup/Obs/lvjm32/Vimos-ifu/Totspecs/Specs2/RXCJ2014.8-2430_fullspec.ps,width=8cm,bbllx=74,bblly=367,bburx=450,bbury=549}  
\psfig{figure=/media/stephen/HYDRA/Backup/Obs/lvjm32/Vimos-ifu/Totspecs/Specs2/RXCJ2101.8-2802_fullspec.ps,width=8cm,bbllx=74,bblly=367,bburx=450,bbury=549}   
\hspace{1.5cm}           
\psfig{figure=/media/stephen/HYDRA/Backup/Obs/lvjm32/Vimos-ifu/Totspecs/Specs2/RXCJ2129.6+0005_fullspec.ps,width=8cm,bbllx=74,bblly=367,bburx=450,bbury=549} 
\caption{continued.}
%\label{fig:spec}
\end{figure}

\FloatBarrier

\begin{figure}
\ContinuedFloat
\psfig{figure=/media/stephen/HYDRA/Backup/Obs/lvjm32/Vimos-ifu/Totspecs/Specs2/RXCJ2213.0-2753_fullspec.ps,width=8cm,bbllx=74,bblly=367,bburx=450,bbury=549} 
\psfig{figure=/media/stephen/HYDRA/Backup/Obs/lvjm32/Vimos-ifu/Totspecs/Specs2/RXJ0000.1+0816_fullspec.ps,width=8cm,bbllx=74,bblly=367,bburx=450,bbury=549} 
\psfig{figure=/media/stephen/HYDRA/Backup/Obs/lvjm32/Vimos-ifu/Totspecs/Specs2/RXJ0338+09_fullspec.ps,width=8cm,bbllx=74,bblly=367,bburx=450,bbury=549} 
\psfig{figure=/media/stephen/HYDRA/Backup/Obs/lvjm32/Vimos-ifu/Totspecs/Specs2/RXJ0352.9+1941_fullspec.ps,width=8cm,bbllx=74,bblly=367,bburx=450,bbury=549} 
\psfig{figure=/media/stephen/HYDRA/Backup/Obs/lvjm32/Vimos-ifu/Totspecs/Specs2/RXJ0439.0+0520_fullspec.ps,width=8cm,bbllx=74,bblly=367,bburx=450,bbury=549} 
\psfig{figure=/media/stephen/HYDRA/Backup/Obs/lvjm32/Vimos-ifu/Totspecs/Specs2/RXJ0747-19_fullspec.ps,width=8cm,bbllx=74,bblly=367,bburx=450,bbury=549} 
\psfig{figure=/media/stephen/HYDRA/Backup/Obs/lvjm32/Vimos-ifu/Totspecs/Specs2/RXJ0821+07_fullspec.ps,width=8cm,bbllx=74,bblly=367,bburx=450,bbury=549} 
\psfig{figure=/media/stephen/HYDRA/Backup/Obs/lvjm32/Vimos-ifu/Totspecs/Specs2/RXJ1651.1+0459_fullspec.ps,width=8cm,bbllx=74,bblly=367,bburx=450,bbury=549}  
\psfig{figure=/media/stephen/HYDRA/Backup/Obs/lvjm32/Vimos-ifu/Totspecs/Specs2/S555_fullspec.ps,width=8cm,bbllx=74,bblly=367,bburx=450,bbury=549}  
\psfig{figure=/media/stephen/HYDRA/Backup/Obs/lvjm32/Vimos-ifu/Totspecs/Specs2/S780_fullspec.ps,width=8cm,bbllx=74,bblly=367,bburx=450,bbury=549}  
\psfig{figure=/media/stephen/HYDRA/Backup/Obs/lvjm32/Vimos-ifu/Totspecs/Specs2/S805_fullspec.ps,width=8cm,bbllx=74,bblly=367,bburx=450,bbury=549}   
\hspace{1.5cm}           
\psfig{figure=/media/stephen/HYDRA/Backup/Obs/lvjm32/Vimos-ifu/Totspecs/Specs2/S851_fullspec.ps,width=8cm,bbllx=74,bblly=367,bburx=450,bbury=549} 
\caption{continued.}
%\label{fig:spec}
\end{figure}

\FloatBarrier 

\begin{figure}
\ContinuedFloat
\psfig{figure=/media/stephen/HYDRA/Backup/Obs/lvjm32/Vimos-ifu/Totspecs/Specs2/Z3179_fullspec.ps,width=8cm,bbllx=74,bblly=367,bburx=450,bbury=549}  
\hspace{1.8cm}           
\psfig{figure=/media/stephen/HYDRA/Backup/Obs/lvjm32/Vimos-ifu/Totspecs/Specs2/Z348_fullspec.ps,width=8cm,bbllx=74,bblly=367,bburx=450,bbury=549} 
\caption{continued.}
%\label{fig:spec}
\end{figure}

%Appendix F-----------------------------------------------------------------------------

\clearpage
\onecolumn
%\thispagestyle{headings}
%\mbox{}
\section{Principle line strengths and ratios}
\label{app:lines}

\begin{sidewaystable}[p]
\begin{center}
\tiny
\centerline{\sc Table \ref{tab:sam}.}
\centerline{\sc The spectroscopic properties for each object in the sample}
\smallskip
\begin{tabular}{l c c c c c c c c c c c}
\hline
\smallskip
Cluster & [OI]$_{\lambda 6300}$ & [OI]$_{\lambda 6366}$ & H$\alpha$ & [NII]$_{\lambda 6583}$ & [SII]$_{\lambda 6716}$ & [SII]$_{\lambda 6731}$ & $\frac{[NII]_{\lambda 6583}}{H\alpha}$ & $\frac{[SII]_{\lambda 6716 + 6731}}{H\alpha}$ & $\frac{[OI]_{\lambda 6300}}{H\alpha}$ & $\frac{[SII]_{\lambda 6716}}{[SII]_{\lambda 6731}}$ \\
  --Region & \multicolumn{6}{c}{ 10$^{-16}$ erg s$^{-1}$ cm$^{-2}$} & & & & \\
\hline
A1060 & & & & & & & & & & \\
  --Centre & 0.203$\pm$0.144 & 0.00$\pm$0.00 & 2.54$\pm$0.152 & 1.55$\pm$0.140 & 0.331$\pm$0.144 & 0.353$\pm$0.152 & 0.611$\pm$0.0661 & 0.269$\pm$0.0841 & 0.0799$\pm$0.0569 & 0.936$\pm$0.573 \\
  --Total & 0.376$\pm$0.376 & 0.00$\pm$0.00 & 17.0$\pm$1.02 & 9.95$\pm$0.895 & 1.78$\pm$0.879 & 0.881$\pm$1.02 & 0.584$\pm$0.0632 & 0.156$\pm$0.0797 & 0.0221$\pm$0.0221 & 2.02$\pm$2.54 \\
  --Extended & 0.173$\pm$0.403 & 0.00$\pm$0.00 & 14.5$\pm$1.03 & 8.40$\pm$0.906 & 1.45$\pm$0.891 & 0.527$\pm$0.888 & 0.579$\pm$0.0749 & 0.136$\pm$0.0873 & 0.0119$\pm$0.0278 & 2.74$\pm$4.92 \\
A1084 & & & & & & & & & & \\
  --Centre & 1.69$\pm$0.237 & 0.411$\pm$0.226 & 3.47$\pm$0.243 & 5.10$\pm$0.255 & 0.00$\pm$0.00 & 0.00$\pm$0.243 & 1.47$\pm$0.126 & 0.00$\pm$0.00 & 0.486$\pm$0.0761 & 0.00$\pm$0.00 \\
  --Total & 5.68$\pm$1.56 & 1.87$\pm$1.53 & 35.5$\pm$1.77 & 14.9$\pm$1.49 & 0.00$\pm$0.00 & 0.00$\pm$1.77 & 0.419$\pm$0.0468 & 0.00$\pm$0.00 & 0.160$\pm$0.0447 & 0.00$\pm$0.00 \\
  --Extended & 3.99$\pm$1.58 & 1.46$\pm$1.54 & 32.0$\pm$1.79 & 9.75$\pm$1.51 & 0.00$\pm$0.00 & 0.00$\pm$0.00 & 0.305$\pm$0.0501 & 0.00$\pm$0.00 & 0.125$\pm$0.0499 & 0.00$\pm$0.00 \\
A1111 & & & & & & & & & & \\
  --Centre & 1.90$\pm$0.286 & 0.249$\pm$0.249 & 4.28$\pm$0.300 & 5.40$\pm$0.270 & 4.32$\pm$0.302 & 2.01$\pm$0.300 & 1.26$\pm$0.108 & 1.48$\pm$0.143 & 0.445$\pm$0.0736 & 2.14$\pm$0.353 \\
  --Total & 11.8$\pm$2.06 & 3.58$\pm$1.99 & 37.6$\pm$2.25 & 36.9$\pm$2.03 & 19.8$\pm$2.08 & 14.5$\pm$2.25 & 0.983$\pm$0.0800 & 0.915$\pm$0.0984 & 0.314$\pm$0.0580 & 1.36$\pm$0.255 \\
  --Extended & 9.88$\pm$2.08 & 3.34$\pm$2.01 & 33.3$\pm$2.27 & 31.5$\pm$2.05 & 15.5$\pm$2.10 & 12.5$\pm$2.13 & 0.947$\pm$0.0893 & 0.842$\pm$0.107 & 0.297$\pm$0.0658 & 1.24$\pm$0.269 \\
A11 & & & & & & & & & & \\
  --Centre & 5.48$\pm$1.37 & 1.43$\pm$1.35 & 32.7$\pm$1.63 & 23.3$\pm$1.40 & 18.9$\pm$1.51 & 15.2$\pm$1.63 & 0.713$\pm$0.0557 & 1.04$\pm$0.0858 & 0.168$\pm$0.0428 & 1.24$\pm$0.166 \\
  --Total & 18.3$\pm$5.20 & 8.49$\pm$5.18 & 125$\pm$6.24 & 97.0$\pm$5.33 & 63.0$\pm$5.67 & 45.2$\pm$6.24 & 0.777$\pm$0.0578 & 0.868$\pm$0.0803 & 0.146$\pm$0.0423 & 1.39$\pm$0.230 \\
  --Extended & 12.8$\pm$5.38 & 7.05$\pm$5.35 & 92.1$\pm$6.45 & 73.7$\pm$5.51 & 44.2$\pm$5.87 & 30.0$\pm$5.60 & 0.800$\pm$0.0820 & 0.805$\pm$0.105 & 0.139$\pm$0.0592 & 1.47$\pm$0.337 \\
A1204 & & & & & & & & & & \\
  --Centre & 1.11$\pm$0.183 & 0.0586$\pm$0.0586 & 1.65$\pm$0.190 & 1.40$\pm$0.175 & 0.286$\pm$0.176 & 0.290$\pm$0.190 & 0.847$\pm$0.144 & 0.348$\pm$0.162 & 0.672$\pm$0.135 & 0.989$\pm$0.889 \\
  --Total & 5.06$\pm$2.61 & 0.508$\pm$0.508 & 42.7$\pm$2.99 & 33.8$\pm$2.70 & 0.286$\pm$0.00 & 5.14$\pm$2.99 & 0.791$\pm$0.0841 & 0.127$\pm$0.0706 & 0.119$\pm$0.0616 & 0.0557$\pm$0.0324 \\
  --Extended & 3.95$\pm$2.61 & 0.449$\pm$0.511 & 41.1$\pm$3.00 & 32.4$\pm$2.71 & 0.00$\pm$0.176 & 4.85$\pm$2.63 & 0.789$\pm$0.0875 & 0.118$\pm$0.0647 & 0.0963$\pm$0.0641 & 0.00$\pm$0.00 \\
A133 & & & & & & & & & & \\
  --Centre & 0.00$\pm$0.00 & 0.00$\pm$0.00 & 0.475$\pm$0.192 & 0.484$\pm$0.184 & 0.0422$\pm$0.0422 & 0.00$\pm$0.192 & 1.02$\pm$0.566 & 0.0888$\pm$0.416 & 0.00$\pm$0.00 & 0.00$\pm$0.00 \\
  --Total & 5.76$\pm$1.24 & 0.00$\pm$0.00 & 16.5$\pm$1.32 & 20.6$\pm$1.24 & 9.23$\pm$1.25 & 5.31$\pm$1.32 & 1.25$\pm$0.125 & 0.881$\pm$0.131 & 0.349$\pm$0.0800 & 1.74$\pm$0.491 \\
  --Extended & 5.76$\pm$1.24 & 0.00$\pm$0.00 & 16.0$\pm$1.33 & 20.1$\pm$1.25 & 9.19$\pm$1.25 & 5.31$\pm$1.22 & 1.25$\pm$0.130 & 0.904$\pm$0.132 & 0.359$\pm$0.0828 & 1.73$\pm$0.462 \\
A1348 & & & & & & & & & & \\
  --Centre & 6.48$\pm$1.78 & 2.42$\pm$1.76 & 25.7$\pm$1.80 & 41.4$\pm$1.86 & 0.545$\pm$0.545 & 0.545$\pm$1.80 & 1.61$\pm$0.134 & 0.0424$\pm$0.0732 & 0.252$\pm$0.0715 & 1.00$\pm$3.45 \\
  --Total & 21.1$\pm$5.06 & 9.63$\pm$5.06 & 79.6$\pm$5.57 & 125$\pm$5.00 & 1.62$\pm$1.62 & 1.62$\pm$5.57 & 1.57$\pm$0.126 & 0.0408$\pm$0.0730 & 0.265$\pm$0.0662 & 1.00$\pm$3.58 \\
  --Extended & 14.6$\pm$5.36 & 7.21$\pm$5.35 & 53.9$\pm$5.86 & 83.5$\pm$5.33 & 1.08$\pm$1.71 & 1.08$\pm$1.71 & 1.55$\pm$0.195 & 0.0400$\pm$0.0451 & 0.271$\pm$0.104 & 1.00$\pm$2.25 \\
A1663 & & & & & & & & & & \\
  --Centre & 0.749$\pm$0.311 & 0.00$\pm$0.00 & 1.60$\pm$0.313 & 6.74$\pm$0.337 & 1.41$\pm$0.318 & 0.844$\pm$0.313 & 4.20$\pm$0.846 & 1.41$\pm$0.391 & 0.467$\pm$0.214 & 1.68$\pm$0.727 \\
  --Total & 3.57$\pm$1.09 & 0.00$\pm$0.00 & 8.67$\pm$1.13 & 22.3$\pm$1.12 & 5.68$\pm$1.11 & 0.844$\pm$1.13 & 2.58$\pm$0.359 & 0.753$\pm$0.207 & 0.412$\pm$0.137 & 6.73$\pm$9.08 \\
  --Extended & 2.83$\pm$1.13 & 0.00$\pm$0.00 & 7.07$\pm$1.17 & 15.6$\pm$1.17 & 4.27$\pm$1.15 & 0.00$\pm$0.317 & 2.21$\pm$0.401 & 0.604$\pm$0.197 & 0.400$\pm$0.174 & 0.00$\pm$0.00 \\
A1668 & & & & & & & & & & \\
  --Centre & 1.72$\pm$0.688 & 0.00$\pm$0.00 & 5.73$\pm$0.688 & 18.1$\pm$0.725 & 5.56$\pm$0.723 & 4.60$\pm$0.688 & 3.16$\pm$0.400 & 1.77$\pm$0.275 & 0.300$\pm$0.125 & 1.21$\pm$0.239 \\
  --Total & 8.93$\pm$3.57 & 0.00$\pm$0.00 & 42.9$\pm$3.86 & 91.1$\pm$3.64 & 22.9$\pm$3.66 & 18.2$\pm$3.86 & 2.12$\pm$0.209 & 0.957$\pm$0.151 & 0.208$\pm$0.0852 & 1.26$\pm$0.334 \\
  --Extended & 7.21$\pm$3.64 & 0.00$\pm$0.00 & 37.2$\pm$3.93 & 73.0$\pm$3.72 & 17.3$\pm$3.73 & 13.6$\pm$3.71 & 1.96$\pm$0.230 & 0.831$\pm$0.166 & 0.194$\pm$0.0999 & 1.27$\pm$0.442 \\
A194 & & & & & & & & & & \\
  --Centre & 1.05$\pm$1.05 & 0.156$\pm$0.156 & 18.6$\pm$1.30 & 17.7$\pm$1.24 & 8.20$\pm$1.27 & 6.57$\pm$1.30 & 0.954$\pm$0.0944 & 0.796$\pm$0.113 & 0.0564$\pm$0.0566 & 1.25$\pm$0.314 \\
  --Total & 2.79$\pm$2.79 & 2.34$\pm$2.34 & 57.0$\pm$3.70 & 31.5$\pm$3.47 & 12.5$\pm$3.51 & 9.62$\pm$3.70 & 0.554$\pm$0.0707 & 0.389$\pm$0.0930 & 0.0490$\pm$0.0491 & 1.30$\pm$0.621 \\
  --Extended & 1.75$\pm$2.98 & 2.18$\pm$2.34 & 38.4$\pm$3.93 & 13.9$\pm$3.68 & 4.34$\pm$3.73 & 3.05$\pm$3.74 & 0.360$\pm$0.103 & 0.192$\pm$0.139 & 0.0454$\pm$0.0777 & 1.42$\pm$2.13 \\
A1991-added & & & & & & & & & & \\
  --Centre & 0.00$\pm$0.00 & 0.0781$\pm$0.0473 & 0.00$\pm$0.00 & 0.0381$\pm$0.0381 & 0.00$\pm$0.00 & 0.122$\pm$0.00 & 0.00$\pm$0.00 & 0.00$\pm$0.00 & 0.00$\pm$0.00 & 0.00$\pm$0.00 \\
  --Total & 8.88$\pm$2.89 & 1.46$\pm$1.46 & 47.6$\pm$2.86 & 55.3$\pm$2.76 & 13.8$\pm$2.90 & 14.0$\pm$2.86 & 1.16$\pm$0.0907 & 0.583$\pm$0.0924 & 0.187$\pm$0.0617 & 0.990$\pm$0.290 \\
  --Extended & 8.88$\pm$2.89 & 1.38$\pm$1.46 & 47.6$\pm$2.86 & 55.3$\pm$2.76 & 13.8$\pm$2.90 & 13.8$\pm$2.93 & 1.16$\pm$0.0907 & 0.581$\pm$0.0934 & 0.187$\pm$0.0617 & 0.999$\pm$0.298 \\
A2052 & & & & & & & & & & \\
  --Centre & 6.55$\pm$2.16 & 1.97$\pm$1.97 & 25.4$\pm$2.29 & 54.0$\pm$2.16 & 24.3$\pm$2.19 & 17.6$\pm$2.29 & 2.13$\pm$0.209 & 1.65$\pm$0.194 & 0.258$\pm$0.0883 & 1.38$\pm$0.218 \\
  --Total & 17.1$\pm$6.33 & 3.72$\pm$3.72 & 71.8$\pm$6.46 & 161$\pm$6.42 & 55.8$\pm$6.69 & 41.7$\pm$6.46 & 2.24$\pm$0.220 & 1.36$\pm$0.178 & 0.238$\pm$0.0908 & 1.34$\pm$0.262 \\
  --Extended & 10.6$\pm$6.69 & 1.75$\pm$4.20 & 46.4$\pm$6.85 & 107$\pm$6.77 & 31.5$\pm$7.04 & 24.1$\pm$7.05 & 2.30$\pm$0.369 & 1.20$\pm$0.278 & 0.228$\pm$0.148 & 1.31$\pm$0.482 \\
A2390 & & & & & & & & & & \\
  --Centre & 4.59$\pm$0.643 & 1.44$\pm$0.639 & 11.3$\pm$0.680 & 10.5$\pm$0.630 & 7.70$\pm$0.693 & 2.06$\pm$0.680 & 0.927$\pm$0.0787 & 0.861$\pm$0.100 & 0.406$\pm$0.0618 & 3.73$\pm$1.27 \\
  --Total & 21.2$\pm$2.12 & 6.40$\pm$2.11 & 48.1$\pm$2.41 & 35.2$\pm$2.11 & 21.0$\pm$2.10 & 14.1$\pm$2.41 & 0.732$\pm$0.0572 & 0.730$\pm$0.0758 & 0.440$\pm$0.0492 & 1.49$\pm$0.295 \\
  --Extended & 16.6$\pm$2.21 & 4.96$\pm$2.21 & 36.8$\pm$2.50 & 24.7$\pm$2.20 & 13.3$\pm$2.22 & 12.0$\pm$2.21 & 0.672$\pm$0.0753 & 0.690$\pm$0.0971 & 0.450$\pm$0.0674 & 1.11$\pm$0.275 \\
A2415 & & & & & & & & & & \\
  --Centre & 4.46$\pm$0.848 & 0.452$\pm$0.452 & 7.20$\pm$0.864 & 17.3$\pm$0.865 & 7.33$\pm$0.843 & 6.67$\pm$0.864 & 2.40$\pm$0.312 & 1.94$\pm$0.287 & 0.619$\pm$0.139 & 1.10$\pm$0.191 \\
  --Total & 6.47$\pm$3.69 & 0.693$\pm$0.693 & 49.1$\pm$3.93 & 80.2$\pm$4.01 & 24.7$\pm$3.83 & 18.7$\pm$3.93 & 1.63$\pm$0.154 & 0.884$\pm$0.132 & 0.132$\pm$0.0759 & 1.32$\pm$0.346 \\
  --Extended & 2.01$\pm$3.78 & 0.241$\pm$0.827 & 41.9$\pm$4.02 & 62.9$\pm$4.10 & 17.4$\pm$3.92 & 12.0$\pm$3.83 & 1.50$\pm$0.174 & 0.701$\pm$0.147 & 0.0479$\pm$0.0905 & 1.45$\pm$0.566 \\
A2495 & & & & & & & & & & \\
  --Centre & 0.266$\pm$0.146 & 0.00$\pm$0.00 & 2.07$\pm$0.155 & 2.65$\pm$0.146 & 0.649$\pm$0.149 & 0.135$\pm$0.155 & 1.28$\pm$0.119 & 0.379$\pm$0.108 & 0.128$\pm$0.0713 & 4.81$\pm$5.64 \\
  --Total & 1.76$\pm$0.807 & 0.00$\pm$0.00 & 9.03$\pm$0.812 & 20.3$\pm$0.812 & 2.82$\pm$0.819 & 2.28$\pm$0.812 & 2.25$\pm$0.221 & 0.565$\pm$0.138 & 0.194$\pm$0.0912 & 1.24$\pm$0.571 \\
  --Extended & 1.49$\pm$0.821 & 0.00$\pm$0.00 & 6.96$\pm$0.827 & 17.6$\pm$0.825 & 2.18$\pm$0.833 & 2.14$\pm$0.831 & 2.54$\pm$0.324 & 0.621$\pm$0.184 & 0.214$\pm$0.121 & 1.02$\pm$0.554 \\
A2566 & & & & & & & & & & \\
  --Centre & 0.00$\pm$0.00 & 0.00$\pm$0.00 & 0.115$\pm$0.115 & 0.00$\pm$0.00 & 0.867$\pm$0.247 & 0.00$\pm$0.115 & 0.00$\pm$0.00 & 7.56$\pm$7.92 & 0.00$\pm$0.00 & 0.00$\pm$0.00 \\
  --Total & 10.4$\pm$2.40 & 1.18$\pm$1.18 & 51.2$\pm$2.56 & 46.7$\pm$2.34 & 12.3$\pm$2.40 & 10.5$\pm$2.56 & 0.912$\pm$0.0645 & 0.445$\pm$0.0720 & 0.204$\pm$0.0480 & 1.17$\pm$0.367 \\
  --Extended & 10.4$\pm$2.40 & 1.18$\pm$1.18 & 51.1$\pm$2.56 & 46.7$\pm$2.34 & 11.4$\pm$2.41 & 10.5$\pm$2.41 & 0.914$\pm$0.0647 & 0.429$\pm$0.0701 & 0.204$\pm$0.0481 & 1.09$\pm$0.340 \\
A2580 & & & & & & & & & & \\
  --Centre & 0.944$\pm$0.250 & 0.694$\pm$0.243 & 2.34$\pm$0.258 & 4.87$\pm$0.243 & 1.83$\pm$0.247 & 1.06$\pm$0.258 & 2.08$\pm$0.251 & 1.23$\pm$0.204 & 0.403$\pm$0.116 & 1.73$\pm$0.480 \\
  --Total & 3.17$\pm$1.44 & 0.694$\pm$0.220 & 36.4$\pm$1.46 & 19.3$\pm$1.44 & 1.83$\pm$0.563 & 1.06$\pm$1.46 & 0.528$\pm$0.0449 & 0.0794$\pm$0.0430 & 0.0869$\pm$0.0397 & 1.73$\pm$2.43 \\
  --Extended & 2.22$\pm$1.46 & 0.00$\pm$0.328 & 34.1$\pm$1.48 & 14.4$\pm$1.46 & 0.00$\pm$0.615 & 0.00$\pm$0.322 & 0.422$\pm$0.0467 & 0.00$\pm$0.00 & 0.0652$\pm$0.0430 & 0.00$\pm$0.00 \\
A2734 & & & & & & & & & & \\
  --Centre & 1.69$\pm$0.541 & 0.00$\pm$0.00 & 5.49$\pm$0.549 & 13.7$\pm$0.548 & 4.97$\pm$0.547 & 3.85$\pm$0.549 & 2.49$\pm$0.269 & 1.61$\pm$0.214 & 0.308$\pm$0.103 & 1.29$\pm$0.232 \\
  --Total & 4.10$\pm$1.44 & 0.152$\pm$0.152 & 10.8$\pm$1.41 & 36.7$\pm$1.47 & 11.4$\pm$1.49 & 6.25$\pm$1.41 & 3.39$\pm$0.461 & 1.63$\pm$0.284 & 0.379$\pm$0.142 & 1.83$\pm$0.475 \\
  --Extended & 2.41$\pm$1.54 & 0.152$\pm$0.152 & 5.34$\pm$1.51 & 23.0$\pm$1.57 & 6.45$\pm$1.58 & 2.40$\pm$1.54 & 4.30$\pm$1.25 & 1.66$\pm$0.626 & 0.452$\pm$0.315 & 2.69$\pm$1.84 \\
A291 & & & & & & & & & & \\
  --Centre & 0.774$\pm$0.383 & 0.306$\pm$0.306 & 8.39$\pm$0.419 & 5.61$\pm$0.393 & 1.68$\pm$0.386 & 1.74$\pm$0.419 & 0.669$\pm$0.0575 & 0.408$\pm$0.0710 & 0.0923$\pm$0.0459 & 0.963$\pm$0.320 \\
  --Total & 11.4$\pm$6.30 & 0.306$\pm$0.00 & 170$\pm$6.82 & 27.1$\pm$6.10 & 34.1$\pm$6.49 & 1.74$\pm$6.82 & 0.159$\pm$0.0364 & 0.211$\pm$0.0559 & 0.0666$\pm$0.0371 & 19.6$\pm$76.6 \\
  --Extended & 10.6$\pm$6.32 & 0.00$\pm$0.306 & 162$\pm$6.83 & 21.5$\pm$6.11 & 32.5$\pm$6.50 & 0.00$\pm$0.384 & 0.133$\pm$0.0381 & 0.200$\pm$0.0411 & 0.0653$\pm$0.0391 & 0.00$\pm$0.00 \\
A3017 & & & & & & & & & & \\
  --Centre & 3.56$\pm$0.552 & 1.21$\pm$0.540 & 13.6$\pm$0.545 & 8.91$\pm$0.535 & 6.36$\pm$0.573 & 5.43$\pm$0.545 & 0.654$\pm$0.0472 & 0.866$\pm$0.0676 & 0.261$\pm$0.0419 & 1.17$\pm$0.158 \\
  --Total & 12.4$\pm$2.47 & 6.10$\pm$2.44 & 69.8$\pm$2.79 & 35.6$\pm$2.49 & 24.9$\pm$2.49 & 18.9$\pm$2.79 & 0.510$\pm$0.0411 & 0.627$\pm$0.0592 & 0.177$\pm$0.0361 & 1.32$\pm$0.236 \\
  --Extended & 8.80$\pm$2.53 & 4.89$\pm$2.50 & 56.2$\pm$2.85 & 26.7$\pm$2.55 & 18.5$\pm$2.56 & 13.4$\pm$2.51 & 0.475$\pm$0.0514 & 0.569$\pm$0.0700 & 0.157$\pm$0.0458 & 1.38$\pm$0.320 \\
A3112 & & & & & & & & & & \\
  --Centre & 6.00$\pm$1.26 & 1.91$\pm$1.23 & 11.4$\pm$1.25 & 30.6$\pm$1.22 & 12.4$\pm$1.24 & 10.6$\pm$1.25 & 2.68$\pm$0.314 & 2.01$\pm$0.270 & 0.527$\pm$0.125 & 1.17$\pm$0.182 \\
  --Total & 10.4$\pm$3.23 & 6.35$\pm$3.17 & 49.7$\pm$3.48 & 68.5$\pm$3.43 & 25.4$\pm$3.30 & 20.3$\pm$3.48 & 1.38$\pm$0.119 & 0.920$\pm$0.116 & 0.210$\pm$0.0666 & 1.25$\pm$0.268 \\
  --Extended & 4.41$\pm$3.47 & 4.44$\pm$3.40 & 38.3$\pm$3.70 & 37.9$\pm$3.64 & 13.0$\pm$3.52 & 9.78$\pm$3.49 & 0.991$\pm$0.135 & 0.596$\pm$0.142 & 0.115$\pm$0.0912 & 1.33$\pm$0.597 \\
\hline
\end{tabular}
\caption[]{}
%\label{tab:spec}
\label{tab:sam}
\end{center}
\end{sidewaystable}

\begin{sidewaystable}[p]
\begin{center}
\tiny
\centerline{\sc Table \ref{tab:sam}.}
\centerline{\sc The spectroscopic properties for each object in the sample}
\smallskip
\begin{tabular}{l c c c c c c c c c c c}
\hline
\smallskip
Cluster & [OI]$_{\lambda 6300}$ & [OI]$_{\lambda 6366}$ & H$\alpha$ & [NII]$_{\lambda 6583}$ & [SII]$_{\lambda 6716}$ & [SII]$_{\lambda 6731}$ & $\frac{[NII]_{\lambda 6583}}{H\alpha}$ & $\frac{[SII]_{\lambda 6716 + 6731}}{H\alpha}$ & $\frac{[OI]_{\lambda 6300}}{H\alpha}$ & $\frac{[SII]_{\lambda 6716}}{[SII]_{\lambda 6731}}$ \\
  --Region & \multicolumn{6}{c}{ 10$^{-16}$ erg s$^{-1}$ cm$^{-2}$} & & & & \\
\hline
A3378 & & & & & & & & & & \\
  --Centre & 0.00$\pm$0.00 & 0.625$\pm$0.331 & 1.66$\pm$0.340 & 3.52$\pm$0.335 & 1.51$\pm$0.333 & 1.98$\pm$0.340 & 2.12$\pm$0.480 & 2.11$\pm$0.519 & 0.00$\pm$0.00 & 0.763$\pm$0.213 \\
  --Total & 0.286$\pm$0.286 & 2.06$\pm$0.874 & 7.90$\pm$0.909 & 13.1$\pm$0.852 & 3.45$\pm$0.864 & 2.61$\pm$0.909 & 1.66$\pm$0.219 & 0.768$\pm$0.182 & 0.0362$\pm$0.0364 & 1.32$\pm$0.566 \\
  --Extended & 0.286$\pm$0.286 & 1.43$\pm$0.934 & 6.25$\pm$0.970 & 9.59$\pm$0.915 & 1.94$\pm$0.926 & 0.631$\pm$0.938 & 1.53$\pm$0.280 & 0.412$\pm$0.221 & 0.0458$\pm$0.0463 & 3.08$\pm$4.80 \\
A3444 & & & & & & & & & & \\
  --Centre & 0.338$\pm$0.138 & 0.756$\pm$0.144 & 5.22$\pm$0.183 & 2.38$\pm$0.143 & 0.00$\pm$0.00 & 1.51$\pm$0.183 & 0.456$\pm$0.0317 & 0.290$\pm$0.0364 & 0.0647$\pm$0.0266 & 0.00$\pm$0.00 \\
  --Total & 0.338$\pm$0.0746 & 4.69$\pm$1.06 & 18.7$\pm$1.12 & 13.2$\pm$1.06 & 0.00$\pm$0.00 & 2.95$\pm$1.12 & 0.707$\pm$0.0707 & 0.158$\pm$0.0607 & 0.0181$\pm$0.00414 & 0.00$\pm$0.00 \\
  --Extended & 0.00$\pm$0.157 & 3.94$\pm$1.07 & 13.5$\pm$1.13 & 10.8$\pm$1.07 & 0.00$\pm$0.00 & 1.44$\pm$1.06 & 0.804$\pm$0.104 & 0.107$\pm$0.0793 & 0.00$\pm$0.00 & 0.00$\pm$0.00 \\
A3574 & & & & & & & & & & \\
  --Centre & 8.83$\pm$2.07 & 3.88$\pm$2.05 & 15.8$\pm$2.14 & 27.2$\pm$2.04 & 20.3$\pm$2.13 & 14.7$\pm$2.14 & 1.72$\pm$0.265 & 2.21$\pm$0.353 & 0.557$\pm$0.151 & 1.38$\pm$0.249 \\
  --Total & 23.1$\pm$8.42 & 4.42$\pm$4.42 & 207$\pm$10.3 & 98.3$\pm$8.85 & 57.6$\pm$8.64 & 32.3$\pm$10.3 & 0.476$\pm$0.0490 & 0.435$\pm$0.0687 & 0.112$\pm$0.0412 & 1.78$\pm$0.630 \\
  --Extended & 14.3$\pm$8.68 & 0.549$\pm$4.88 & 191$\pm$10.5 & 71.1$\pm$9.08 & 37.3$\pm$8.90 & 17.6$\pm$8.82 & 0.373$\pm$0.0519 & 0.288$\pm$0.0676 & 0.0748$\pm$0.0457 & 2.12$\pm$1.17 \\
A3581 & & & & & & & & & & \\
  --Centre & 9.53$\pm$2.57 & 1.77$\pm$1.77 & 29.0$\pm$2.61 & 62.6$\pm$2.50 & 32.7$\pm$2.94 & 0.00$\pm$2.61 & 2.15$\pm$0.212 & 1.13$\pm$0.169 & 0.328$\pm$0.0934 & 0.00$\pm$0.00 \\
  --Total & 53.9$\pm$16.7 & 11.3$\pm$11.3 & 252$\pm$17.7 & 395$\pm$15.8 & 170$\pm$21.2 & 0.00$\pm$17.7 & 1.56$\pm$0.126 & 0.672$\pm$0.119 & 0.214$\pm$0.0679 & 0.00$\pm$0.00 \\
  --Extended & 44.4$\pm$16.9 & 9.51$\pm$11.4 & 223$\pm$17.9 & 332$\pm$16.0 & 137$\pm$21.4 & 0.00$\pm$0.00 & 1.49$\pm$0.139 & 0.613$\pm$0.108 & 0.199$\pm$0.0774 & 0.00$\pm$0.00 \\
A3605 & & & & & & & & & & \\
  --Centre & 4.85$\pm$2.04 & 2.85$\pm$2.01 & 13.5$\pm$2.09 & 49.7$\pm$2.24 & 19.3$\pm$2.03 & 12.9$\pm$2.09 & 3.68$\pm$0.595 & 2.39$\pm$0.429 & 0.359$\pm$0.161 & 1.49$\pm$0.287 \\
  --Total & 16.2$\pm$5.02 & 8.76$\pm$4.99 & 43.8$\pm$5.26 & 111$\pm$5.53 & 38.1$\pm$5.14 & 26.0$\pm$5.26 & 2.53$\pm$0.328 & 1.46$\pm$0.243 & 0.370$\pm$0.123 & 1.46$\pm$0.356 \\
  --Extended & 11.4$\pm$5.42 & 5.91$\pm$5.38 & 30.3$\pm$5.66 & 60.9$\pm$5.97 & 18.8$\pm$5.52 & 13.1$\pm$5.48 & 2.01$\pm$0.424 & 1.05$\pm$0.323 & 0.375$\pm$0.192 & 1.44$\pm$0.735 \\
A3638 & & & & & & & & & & \\
  --Centre & 1.65$\pm$0.322 & 0.559$\pm$0.321 & 4.61$\pm$0.323 & 6.73$\pm$0.336 & 3.18$\pm$0.318 & 2.37$\pm$0.323 & 1.46$\pm$0.126 & 1.21$\pm$0.130 & 0.358$\pm$0.0742 & 1.34$\pm$0.226 \\
  --Total & 8.92$\pm$2.32 & 3.18$\pm$2.31 & 37.3$\pm$2.61 & 54.6$\pm$2.18 & 20.8$\pm$2.39 & 15.0$\pm$2.61 & 1.46$\pm$0.118 & 0.961$\pm$0.116 & 0.239$\pm$0.0643 & 1.38$\pm$0.288 \\
  --Extended & 7.27$\pm$2.34 & 2.62$\pm$2.33 & 32.7$\pm$2.63 & 47.9$\pm$2.21 & 17.6$\pm$2.41 & 12.7$\pm$2.43 & 1.46$\pm$0.136 & 0.926$\pm$0.129 & 0.222$\pm$0.0738 & 1.39$\pm$0.328 \\
A3639 & & & & & & & & & & \\
  --Centre & 2.10$\pm$0.504 & 0.535$\pm$0.490 & 7.95$\pm$0.556 & 11.0$\pm$0.550 & 6.10$\pm$0.519 & 3.50$\pm$0.556 & 1.38$\pm$0.119 & 1.21$\pm$0.128 & 0.264$\pm$0.0660 & 1.74$\pm$0.314 \\
  --Total & 24.5$\pm$4.66 & 0.535$\pm$0.00 & 41.7$\pm$4.80 & 41.6$\pm$4.57 & 15.1$\pm$4.67 & 16.2$\pm$4.80 & 0.996$\pm$0.159 & 0.749$\pm$0.182 & 0.588$\pm$0.131 & 0.930$\pm$0.399 \\
  --Extended & 22.4$\pm$4.69 & 0.00$\pm$0.490 & 33.8$\pm$4.83 & 30.6$\pm$4.60 & 8.95$\pm$4.70 & 12.7$\pm$4.64 & 0.905$\pm$0.188 & 0.641$\pm$0.216 & 0.664$\pm$0.168 & 0.705$\pm$0.451 \\
A3806 & & & & & & & & & & \\
  --Centre & 1.30$\pm$0.454 & 1.19$\pm$0.452 & 2.37$\pm$0.451 & 10.4$\pm$0.519 & 2.04$\pm$0.449 & 0.697$\pm$0.451 & 4.38$\pm$0.860 & 1.15$\pm$0.346 & 0.547$\pm$0.218 & 2.93$\pm$2.00 \\
  --Total & 3.69$\pm$2.38 & 3.60$\pm$2.38 & 15.0$\pm$2.39 & 65.8$\pm$2.63 & 7.13$\pm$2.39 & 2.14$\pm$2.39 & 4.40$\pm$0.725 & 0.620$\pm$0.247 & 0.247$\pm$0.164 & 3.32$\pm$3.88 \\
  --Extended & 2.40$\pm$2.42 & 2.42$\pm$2.42 & 12.6$\pm$2.44 & 55.4$\pm$2.68 & 5.09$\pm$2.43 & 1.45$\pm$2.19 & 4.40$\pm$0.878 & 0.519$\pm$0.279 & 0.190$\pm$0.196 & 3.52$\pm$5.58 \\
A383 & & & & & & & & & & \\
  --Centre & 2.22$\pm$0.389 & 0.527$\pm$0.384 & 6.72$\pm$0.403 & 9.51$\pm$0.380 & 3.43$\pm$0.412 & 2.15$\pm$0.403 & 1.41$\pm$0.102 & 0.830$\pm$0.0991 & 0.331$\pm$0.0612 & 1.59$\pm$0.355 \\
  --Total & 9.30$\pm$2.09 & 3.98$\pm$2.05 & 37.8$\pm$2.27 & 45.9$\pm$2.29 & 14.9$\pm$2.09 & 8.98$\pm$2.27 & 1.21$\pm$0.0947 & 0.632$\pm$0.0900 & 0.246$\pm$0.0572 & 1.66$\pm$0.480 \\
  --Extended & 7.07$\pm$2.13 & 3.45$\pm$2.08 & 31.1$\pm$2.30 & 36.4$\pm$2.32 & 11.5$\pm$2.13 & 6.83$\pm$2.10 & 1.17$\pm$0.114 & 0.590$\pm$0.106 & 0.227$\pm$0.0705 & 1.69$\pm$0.605 \\
A3880 & & & & & & & & & & \\
  --Centre & 3.42$\pm$1.08 & 1.99$\pm$1.07 & 11.6$\pm$1.16 & 26.6$\pm$1.06 & 10.3$\pm$1.13 & 6.03$\pm$1.16 & 2.29$\pm$0.247 & 1.40$\pm$0.198 & 0.295$\pm$0.0975 & 1.70$\pm$0.377 \\
  --Total & 30.7$\pm$8.29 & 11.2$\pm$8.32 & 105$\pm$8.43 & 214$\pm$8.55 & 56.7$\pm$8.51 & 43.4$\pm$8.43 & 2.03$\pm$0.181 & 0.950$\pm$0.137 & 0.291$\pm$0.0821 & 1.31$\pm$0.320 \\
  --Extended & 27.3$\pm$8.36 & 9.25$\pm$8.39 & 93.8$\pm$8.51 & 187$\pm$8.61 & 46.5$\pm$8.58 & 37.4$\pm$8.54 & 1.99$\pm$0.203 & 0.894$\pm$0.152 & 0.291$\pm$0.0930 & 1.24$\pm$0.365 \\
A3998 & & & & & & & & & & \\
  --Centre & 1.46$\pm$0.738 & 0.199$\pm$0.199 & 2.42$\pm$0.302 & 5.70$\pm$0.314 & 1.62$\pm$0.300 & 1.44$\pm$0.302 & 2.36$\pm$0.322 & 1.27$\pm$0.237 & 0.605$\pm$0.315 & 1.13$\pm$0.316 \\
  --Total & 1.46$\pm$0.00 & 1.62$\pm$1.62 & 32.1$\pm$1.93 & 41.5$\pm$2.07 & 9.55$\pm$1.91 & 9.62$\pm$1.93 & 1.29$\pm$0.101 & 0.597$\pm$0.0917 & 0.0455$\pm$0.00273 & 0.993$\pm$0.281 \\
  --Extended & 0.00$\pm$0.738 & 1.42$\pm$1.63 & 29.7$\pm$1.95 & 35.8$\pm$2.10 & 7.92$\pm$1.93 & 8.18$\pm$1.95 & 1.21$\pm$0.106 & 0.542$\pm$0.0990 & 0.00$\pm$0.00 & 0.969$\pm$0.330 \\
A4059 & & & & & & & & & & \\
  --Centre & 6.14$\pm$1.78 & 2.27$\pm$1.75 & 8.01$\pm$4.20 & 47.2$\pm$3.54 & 20.5$\pm$1.84 & 14.8$\pm$4.20 & 5.90$\pm$3.13 & 4.40$\pm$2.38 & 0.767$\pm$0.460 & 1.39$\pm$0.414 \\
  --Total & 18.9$\pm$7.38 & 3.56$\pm$3.56 & 42.5$\pm$15.5 & 212$\pm$22.3 & 53.6$\pm$7.50 & 43.3$\pm$15.5 & 4.99$\pm$1.90 & 2.28$\pm$0.926 & 0.445$\pm$0.238 & 1.24$\pm$0.475 \\
  --Extended & 12.8$\pm$7.59 & 1.29$\pm$3.97 & 34.5$\pm$16.1 & 165$\pm$22.6 & 33.1$\pm$7.73 & 28.6$\pm$7.58 & 4.78$\pm$2.32 & 1.79$\pm$0.890 & 0.371$\pm$0.280 & 1.16$\pm$0.409 \\
A478 & & & & & & & & & & \\
  --Centre & 3.09$\pm$0.650 & 0.641$\pm$0.641 & 13.0$\pm$0.650 & 13.9$\pm$0.695 & 6.17$\pm$0.679 & 4.66$\pm$0.650 & 1.07$\pm$0.0756 & 0.834$\pm$0.0835 & 0.238$\pm$0.0514 & 1.32$\pm$0.235 \\
  --Total & 27.7$\pm$5.83 & 6.58$\pm$5.75 & 122$\pm$6.10 & 121$\pm$6.06 & 46.4$\pm$6.03 & 30.6$\pm$6.10 & 0.993$\pm$0.0702 & 0.632$\pm$0.0771 & 0.228$\pm$0.0491 & 1.52$\pm$0.360 \\
  --Extended & 24.6$\pm$5.86 & 5.94$\pm$5.79 & 109$\pm$6.13 & 107$\pm$6.09 & 40.2$\pm$6.07 & 26.0$\pm$5.85 & 0.984$\pm$0.0787 & 0.608$\pm$0.0846 & 0.226$\pm$0.0553 & 1.55$\pm$0.421 \\
A496 & & & & & & & & & & \\
  --Centre & 4.96$\pm$1.84 & 0.742$\pm$0.742 & 19.5$\pm$1.95 & 46.2$\pm$1.85 & 19.1$\pm$1.91 & 14.2$\pm$1.95 & 2.37$\pm$0.255 & 1.71$\pm$0.221 & 0.254$\pm$0.0975 & 1.35$\pm$0.229 \\
  --Total & 30.4$\pm$11.0 & 5.19$\pm$5.19 & 121$\pm$10.9 & 275$\pm$11.0 & 95.7$\pm$11.5 & 61.5$\pm$10.9 & 2.27$\pm$0.224 & 1.30$\pm$0.175 & 0.251$\pm$0.0932 & 1.55$\pm$0.333 \\
  --Extended & 25.5$\pm$11.1 & 4.45$\pm$5.24 & 102$\pm$11.1 & 229$\pm$11.2 & 76.6$\pm$11.6 & 47.4$\pm$11.2 & 2.25$\pm$0.269 & 1.22$\pm$0.207 & 0.251$\pm$0.113 & 1.62$\pm$0.455 \\
A795 & & & & & & & & & & \\
  --Centre & 6.99$\pm$0.699 & 2.41$\pm$0.700 & 10.7$\pm$0.748 & 15.6$\pm$0.781 & 0.773$\pm$0.688 & 4.12$\pm$0.748 & 1.46$\pm$0.126 & 0.458$\pm$0.100 & 0.654$\pm$0.0799 & 0.188$\pm$0.170 \\
  --Total & 13.8$\pm$1.66 & 6.21$\pm$1.61 & 30.4$\pm$1.67 & 29.7$\pm$1.63 & 0.773$\pm$0.00 & 4.12$\pm$1.67 & 0.978$\pm$0.0761 & 0.161$\pm$0.0557 & 0.456$\pm$0.0602 & 0.188$\pm$0.0760 \\
  --Extended & 6.86$\pm$1.80 & 3.80$\pm$1.76 & 19.7$\pm$1.83 & 14.1$\pm$1.81 & 0.00$\pm$0.688 & 0.00$\pm$1.74 & 0.715$\pm$0.114 & 0.00$\pm$0.00 & 0.348$\pm$0.0972 & 0.00$\pm$0.00 \\
A85 & & & & & & & & & & \\
  --Centre & 0.289$\pm$0.0967 & 0.0634$\pm$0.0634 & 0.00$\pm$0.00 & 0.00$\pm$0.00 & 0.306$\pm$0.0963 & 0.629$\pm$0.00 & 0.00$\pm$0.00 & 0.00$\pm$0.00 & 0.00$\pm$0.00 & 0.486$\pm$0.153 \\
  --Total & 1.11$\pm$1.11 & 0.0634$\pm$0.00 & 14.3$\pm$1.71 & 43.3$\pm$1.73 & 7.47$\pm$1.72 & 6.63$\pm$1.71 & 3.03$\pm$0.383 & 0.987$\pm$0.207 & 0.0780$\pm$0.0786 & 1.13$\pm$0.390 \\
  --Extended & 0.826$\pm$1.12 & 0.00$\pm$0.0634 & 14.3$\pm$1.71 & 43.3$\pm$1.73 & 7.16$\pm$1.72 & 6.00$\pm$1.69 & 3.03$\pm$0.383 & 0.921$\pm$0.202 & 0.0578$\pm$0.0786 & 1.19$\pm$0.442 \\
HCG62 & & & & & & & & & & \\
  --Centre & 1.67$\pm$1.20 & 0.00$\pm$0.00 & 1.91$\pm$1.19 & 20.8$\pm$1.25 & 4.17$\pm$1.19 & 8.83$\pm$1.19 & 10.9$\pm$6.77 & 6.80$\pm$4.31 & 0.875$\pm$0.828 & 0.473$\pm$0.149 \\
  --Total & 5.26$\pm$3.82 & 0.00$\pm$0.00 & 13.2$\pm$3.88 & 57.7$\pm$3.75 & 7.88$\pm$3.86 & 25.7$\pm$3.88 & 4.39$\pm$1.32 & 2.55$\pm$0.861 & 0.400$\pm$0.313 & 0.306$\pm$0.157 \\
  --Extended & 3.59$\pm$4.00 & 0.00$\pm$0.00 & 11.2$\pm$4.06 & 36.9$\pm$3.95 & 3.71$\pm$4.04 & 16.9$\pm$4.05 & 3.28$\pm$1.24 & 1.83$\pm$0.834 & 0.319$\pm$0.374 & 0.219$\pm$0.245 \\
Hydra-a & & & & & & & & & & \\
  --Centre & 8.01$\pm$2.08 & 1.72$\pm$1.72 & 45.0$\pm$2.25 & 38.9$\pm$2.34 & 22.4$\pm$2.24 & 17.6$\pm$2.25 & 0.866$\pm$0.0676 & 0.891$\pm$0.0835 & 0.178$\pm$0.0472 & 1.27$\pm$0.206 \\
  --Total & 36.6$\pm$9.52 & 11.6$\pm$9.43 & 199$\pm$9.96 & 172$\pm$10.3 & 98.9$\pm$9.89 & 80.3$\pm$9.96 & 0.861$\pm$0.0673 & 0.899$\pm$0.0836 & 0.184$\pm$0.0487 & 1.23$\pm$0.196 \\
  --Extended & 28.6$\pm$9.75 & 9.85$\pm$9.59 & 154$\pm$10.2 & 133$\pm$10.6 & 76.5$\pm$10.1 & 62.6$\pm$9.86 & 0.860$\pm$0.0891 & 0.902$\pm$0.109 & 0.185$\pm$0.0644 & 1.22$\pm$0.251 \\
NGC4325 & & & & & & & & & & \\
  --Centre & 2.59$\pm$0.648 & 0.00552$\pm$0.00552 & 8.21$\pm$0.656 & 14.3$\pm$0.714 & 3.27$\pm$0.719 & 3.03$\pm$0.656 & 1.74$\pm$0.164 & 0.768$\pm$0.134 & 0.316$\pm$0.0829 & 1.08$\pm$0.333 \\
  --Total & 11.5$\pm$3.98 & 0.00552$\pm$0.00 & 61.3$\pm$4.29 & 79.7$\pm$3.98 & 6.36$\pm$4.13 & 11.5$\pm$4.29 & 1.30$\pm$0.112 & 0.292$\pm$0.0993 & 0.188$\pm$0.0662 & 0.551$\pm$0.413 \\
  --Extended & 8.95$\pm$4.03 & 0.00$\pm$0.00552 & 53.1$\pm$4.34 & 65.4$\pm$4.05 & 3.09$\pm$4.19 & 8.51$\pm$4.03 & 1.23$\pm$0.126 & 0.218$\pm$0.111 & 0.168$\pm$0.0771 & 0.363$\pm$0.522 \\
NGC5044 & & & & & & & & & & \\
  --Centre & 0.00$\pm$0.00 & 0.00$\pm$0.00 & 77.2$\pm$3.86 & 2.92$\pm$2.92 & 20.7$\pm$3.30 & 0.00$\pm$3.86 & 0.0379$\pm$0.0379 & 0.268$\pm$0.0672 & 0.00$\pm$0.00 & 0.00$\pm$0.00 \\
  --Total & 0.00$\pm$0.00 & 5.49$\pm$5.49 & 320$\pm$16.0 & 2.92$\pm$0.00 & 30.1$\pm$14.0 & 0.00$\pm$16.0 & 0.00913$\pm$0.000457 & 0.0939$\pm$0.0665 & 0.00$\pm$0.00 & 0.00$\pm$0.00 \\
  --Extended & 0.00$\pm$0.00 & 5.49$\pm$5.49 & 243$\pm$16.5 & 0.00$\pm$2.92 & 9.40$\pm$14.4 & 0.00$\pm$0.00 & 0.00$\pm$0.00 & 0.0387$\pm$0.0592 & 0.00$\pm$0.00 & 0.00$\pm$0.00 \\
\hline
\end{tabular}
%\label{tab:spec}
\end{center}
\end{sidewaystable}

\begin{sidewaystable}[p]
\begin{center}
\tiny
\centerline{\sc Table \ref{tab:sam}.}
\centerline{\sc The spectroscopic properties for each object in the sample}
\smallskip
\begin{tabular}{l c c c c c c c c c c c}
\hline
\smallskip
Cluster & [OI]$_{\lambda 6300}$ & [OI]$_{\lambda 6366}$ & H$\alpha$ & [NII]$_{\lambda 6583}$ & [SII]$_{\lambda 6716}$ & [SII]$_{\lambda 6731}$ & $\frac{[NII]_{\lambda 6583}}{H\alpha}$ & $\frac{[SII]_{\lambda 6716 + 6731}}{H\alpha}$ & $\frac{[OI]_{\lambda 6300}}{H\alpha}$ & $\frac{[SII]_{\lambda 6716}}{[SII]_{\lambda 6731}}$ \\
  --Region & \multicolumn{6}{c}{ 10$^{-16}$ erg s$^{-1}$ cm$^{-2}$} & & & & \\
\hline
NGC533 & & & & & & & & & & \\
  --Centre & 2.93$\pm$1.58 & 0.00$\pm$0.00 & 7.72$\pm$1.62 & 29.7$\pm$1.49 & 10.6$\pm$1.58 & 10.8$\pm$1.62 & 3.85$\pm$0.831 & 2.77$\pm$0.651 & 0.379$\pm$0.220 & 0.976$\pm$0.207 \\
  --Total & 8.32$\pm$5.83 & 2.97$\pm$2.97 & 20.6$\pm$5.86 & 94.7$\pm$5.68 & 31.8$\pm$5.88 & 22.5$\pm$5.86 & 4.60$\pm$1.34 & 2.64$\pm$0.854 & 0.405$\pm$0.306 & 1.41$\pm$0.452 \\
  --Extended & 5.40$\pm$6.04 & 2.97$\pm$2.97 & 12.8$\pm$6.08 & 64.9$\pm$5.87 & 21.3$\pm$6.09 & 11.7$\pm$6.18 & 5.06$\pm$2.44 & 2.57$\pm$1.39 & 0.421$\pm$0.511 & 1.82$\pm$1.09 \\
NGC5813 & & & & & & & & & & \\
  --Centre & 3.35$\pm$1.82 & 0.00$\pm$0.00 & 0.00$\pm$0.00 & 23.4$\pm$1.75 & 8.60$\pm$1.85 & 2.66$\pm$0.00 & 0.00$\pm$0.00 & 0.00$\pm$0.00 & 0.00$\pm$0.00 & 3.24$\pm$0.696 \\
  --Total & 7.67$\pm$3.83 & 6.68$\pm$3.84 & 36.5$\pm$4.02 & 71.3$\pm$4.28 & 32.6$\pm$3.91 & 15.8$\pm$4.02 & 1.95$\pm$0.245 & 1.33$\pm$0.212 & 0.210$\pm$0.107 & 2.06$\pm$0.581 \\
  --Extended & 4.32$\pm$4.25 & 6.68$\pm$3.84 & 36.5$\pm$4.02 & 48.0$\pm$4.63 & 24.0$\pm$4.33 & 13.1$\pm$4.27 & 1.31$\pm$0.192 & 1.02$\pm$0.201 & 0.118$\pm$0.117 & 1.83$\pm$0.679 \\
NGC5846 & & & & & & & & & & \\
  --Centre & 3.56$\pm$1.66 & 0.730$\pm$0.730 & 0.00$\pm$0.00 & 35.1$\pm$1.75 & 9.06$\pm$1.68 & 4.83$\pm$0.00 & 0.00$\pm$0.00 & 0.00$\pm$0.00 & 0.00$\pm$0.00 & 1.87$\pm$0.347 \\
  --Total & 5.88$\pm$5.88 & 0.730$\pm$0.00 & 41.2$\pm$8.87 & 212$\pm$9.54 & 55.1$\pm$9.09 & 43.6$\pm$8.87 & 5.14$\pm$1.13 & 2.39$\pm$0.600 & 0.143$\pm$0.146 & 1.26$\pm$0.330 \\
  --Extended & 2.31$\pm$6.11 & 0.00$\pm$0.730 & 41.2$\pm$8.87 & 177$\pm$9.70 & 46.0$\pm$9.24 & 38.8$\pm$9.10 & 4.29$\pm$0.952 & 2.06$\pm$0.543 & 0.0561$\pm$0.149 & 1.19$\pm$0.366 \\
RXCJ0120.9-1351 & & & & & & & & & & \\
  --Centre & 3.61$\pm$0.939 & 1.41$\pm$0.912 & 6.16$\pm$0.924 & 21.4$\pm$1.17 & 7.93$\pm$0.952 & 6.57$\pm$0.924 & 3.47$\pm$0.554 & 2.35$\pm$0.414 & 0.586$\pm$0.176 & 1.21$\pm$0.223 \\
  --Total & 12.3$\pm$2.28 & 1.41$\pm$1.16 & 12.6$\pm$2.33 & 52.2$\pm$4.43 & 15.6$\pm$2.27 & 15.1$\pm$2.33 & 4.15$\pm$0.845 & 2.45$\pm$0.521 & 0.981$\pm$0.257 & 1.04$\pm$0.219 \\
  --Extended & 8.71$\pm$2.47 & 0.00$\pm$1.47 & 6.41$\pm$2.50 & 30.8$\pm$4.59 & 7.71$\pm$2.46 & 8.53$\pm$2.44 & 4.80$\pm$2.01 & 2.53$\pm$1.13 & 1.36$\pm$0.655 & 0.904$\pm$0.388 \\
RXCJ0132.6-0804 & & & & & & & & & & \\
  --Centre & 7.62$\pm$1.37 & 2.93$\pm$1.37 & 20.1$\pm$1.40 & 36.6$\pm$1.46 & 13.3$\pm$1.46 & 11.7$\pm$1.40 & 1.82$\pm$0.147 & 1.24$\pm$0.133 & 0.380$\pm$0.0734 & 1.14$\pm$0.185 \\
  --Total & 16.8$\pm$4.04 & 5.55$\pm$3.94 & 71.4$\pm$4.28 & 101$\pm$4.04 & 30.8$\pm$4.00 & 22.2$\pm$4.28 & 1.41$\pm$0.102 & 0.742$\pm$0.0934 & 0.236$\pm$0.0584 & 1.39$\pm$0.323 \\
  --Extended & 9.23$\pm$4.27 & 2.62$\pm$4.17 & 51.3$\pm$4.51 & 64.3$\pm$4.29 & 17.5$\pm$4.26 & 10.5$\pm$4.23 & 1.25$\pm$0.138 & 0.546$\pm$0.126 & 0.180$\pm$0.0846 & 1.67$\pm$0.783 \\
RXCJ0331.1-2100 & & & & & & & & & & \\
  --Centre & 1.30$\pm$0.916 & 0.00$\pm$0.00 & 1.54$\pm$0.924 & 5.24$\pm$0.890 & 5.14$\pm$0.925 & 0.00$\pm$0.924 & 3.40$\pm$2.12 & 3.34$\pm$2.18 & 0.843$\pm$0.781 & 0.00$\pm$0.00 \\
  --Total & 11.9$\pm$2.13 & 0.00$\pm$0.00 & 34.7$\pm$2.08 & 33.6$\pm$2.01 & 19.8$\pm$2.18 & 8.79$\pm$2.08 & 0.967$\pm$0.0821 & 0.825$\pm$0.1000 & 0.342$\pm$0.0648 & 2.26$\pm$0.589 \\
  --Extended & 10.6$\pm$2.32 & 0.00$\pm$0.00 & 33.2$\pm$2.28 & 28.3$\pm$2.20 & 14.7$\pm$2.37 & 8.79$\pm$2.07 & 0.854$\pm$0.0886 & 0.708$\pm$0.107 & 0.318$\pm$0.0733 & 1.67$\pm$0.476 \\
RXCJ0543.4-4430 & & & & & & & & & & \\
  --Centre & 1.01$\pm$0.212 & 1.75$\pm$0.219 & 0.00$\pm$0.00 & 0.00$\pm$0.00 & 0.209$\pm$0.106 & 1.14$\pm$0.00 & 0.00$\pm$0.00 & 0.00$\pm$0.00 & 0.00$\pm$0.00 & 0.183$\pm$0.0924 \\
  --Total & 1.77$\pm$0.919 & 1.75$\pm$0.922 & 0.00$\pm$0.00 & 2.55$\pm$0.878 & 2.41$\pm$0.915 & 1.16$\pm$0.00 & 0.00$\pm$0.00 & 0.00$\pm$0.00 & 0.00$\pm$0.00 & 2.07$\pm$0.787 \\
  --Extended & 0.755$\pm$0.943 & 0.00$\pm$0.947 & 0.00$\pm$0.00 & 2.55$\pm$0.878 & 2.20$\pm$0.921 & 0.0192$\pm$0.943 & 0.00$\pm$0.00 & 0.00$\pm$0.00 & 0.00$\pm$0.00 & 115$\pm$5630 \\
RXCJ0944.6-2633 & & & & & & & & & & \\
  --Centre & 13.1$\pm$1.18 & 5.56$\pm$1.08 & 26.5$\pm$1.19 & 14.4$\pm$1.08 & 9.90$\pm$1.09 & 8.85$\pm$1.19 & 0.544$\pm$0.0476 & 0.706$\pm$0.0687 & 0.492$\pm$0.0495 & 1.12$\pm$0.195 \\
  --Total & 20.2$\pm$3.84 & 5.96$\pm$3.70 & 107$\pm$4.29 & 45.2$\pm$3.62 & 25.7$\pm$3.85 & 23.3$\pm$4.29 & 0.422$\pm$0.0377 & 0.457$\pm$0.0568 & 0.188$\pm$0.0365 & 1.10$\pm$0.262 \\
  --Extended & 7.12$\pm$4.01 & 0.402$\pm$3.85 & 80.8$\pm$4.46 & 30.8$\pm$3.78 & 15.8$\pm$4.01 & 14.5$\pm$3.89 & 0.381$\pm$0.0513 & 0.375$\pm$0.0722 & 0.0882$\pm$0.0499 & 1.09$\pm$0.403 \\
RXCJ1257.1-1339 & & & & & & & & & & \\
  --Centre & 7.34$\pm$1.69 & 1.49$\pm$1.49 & 22.8$\pm$1.82 & 32.0$\pm$1.60 & 20.6$\pm$1.75 & 15.7$\pm$1.82 & 1.40$\pm$0.132 & 1.59$\pm$0.169 & 0.322$\pm$0.0784 & 1.31$\pm$0.189 \\
  --Total & 55.8$\pm$17.3 & 21.7$\pm$17.2 & 237$\pm$19.0 & 303$\pm$18.2 & 187$\pm$18.7 & 134$\pm$19.0 & 1.28$\pm$0.128 & 1.36$\pm$0.156 & 0.235$\pm$0.0752 & 1.39$\pm$0.242 \\
  --Extended & 48.4$\pm$17.4 & 20.2$\pm$17.2 & 215$\pm$19.1 & 271$\pm$18.3 & 167$\pm$18.8 & 119$\pm$17.6 & 1.26$\pm$0.141 & 1.33$\pm$0.168 & 0.226$\pm$0.0834 & 1.41$\pm$0.262 \\
RXCJ1304.2-3030 & & & & & & & & & & \\
  --Centre & 17.1$\pm$3.76 & 2.61$\pm$2.61 & 41.1$\pm$3.91 & 73.8$\pm$3.69 & 45.2$\pm$3.84 & 30.9$\pm$3.91 & 1.80$\pm$0.193 & 1.85$\pm$0.221 & 0.415$\pm$0.0995 & 1.46$\pm$0.223 \\
  --Total & 144$\pm$27.4 & 25.5$\pm$23.5 & 365$\pm$29.2 & 662$\pm$29.8 & 371$\pm$27.8 & 277$\pm$29.2 & 1.81$\pm$0.166 & 1.77$\pm$0.180 & 0.395$\pm$0.0815 & 1.34$\pm$0.174 \\
  --Extended & 127$\pm$27.7 & 22.9$\pm$23.6 & 324$\pm$29.5 & 588$\pm$30.0 & 326$\pm$28.1 & 246$\pm$28.0 & 1.81$\pm$0.189 & 1.76$\pm$0.202 & 0.393$\pm$0.0926 & 1.33$\pm$0.189 \\
RXCJ1436.8-0900 & & & & & & & & & & \\
  --Centre & 1.67$\pm$0.818 & 0.00$\pm$0.00 & 16.7$\pm$0.835 & 18.5$\pm$0.923 & 4.69$\pm$0.844 & 3.06$\pm$0.835 & 1.11$\pm$0.0782 & 0.464$\pm$0.0748 & 0.100$\pm$0.0493 & 1.53$\pm$0.500 \\
  --Total & 9.45$\pm$4.96 & 0.00$\pm$0.00 & 87.1$\pm$5.23 & 122$\pm$4.89 & 24.0$\pm$5.03 & 15.0$\pm$5.23 & 1.40$\pm$0.101 & 0.447$\pm$0.0875 & 0.108$\pm$0.0573 & 1.59$\pm$0.648 \\
  --Extended & 7.78$\pm$5.03 & 0.00$\pm$0.00 & 70.4$\pm$5.29 & 104$\pm$4.98 & 19.3$\pm$5.10 & 12.0$\pm$5.03 & 1.47$\pm$0.131 & 0.443$\pm$0.107 & 0.110$\pm$0.0719 & 1.61$\pm$0.800 \\
RXCJ1511.5+0145 & & & & & & & & & & \\
  --Centre & 0.329$\pm$0.291 & 0.00$\pm$0.00 & 0.368$\pm$0.292 & 4.11$\pm$0.287 & 1.02$\pm$0.296 & 0.783$\pm$0.292 & 11.2$\pm$8.92 & 4.91$\pm$4.06 & 0.896$\pm$1.07 & 1.30$\pm$0.615 \\
  --Total & 0.329$\pm$0.00 & 0.368$\pm$0.368 & 2.77$\pm$0.733 & 10.8$\pm$0.756 & 2.07$\pm$0.734 & 3.08$\pm$0.733 & 3.91$\pm$1.07 & 1.86$\pm$0.620 & 0.119$\pm$0.0315 & 0.671$\pm$0.287 \\
  --Extended & 0.00$\pm$0.291 & 0.368$\pm$0.368 & 2.40$\pm$0.789 & 6.70$\pm$0.809 & 1.05$\pm$0.792 & 2.30$\pm$0.796 & 2.79$\pm$0.978 & 1.40$\pm$0.656 & 0.00$\pm$0.00 & 0.456$\pm$0.379 \\
RXCJ1524.2-3154 & & & & & & & & & & \\
  --Centre & 5.09$\pm$1.22 & 0.873$\pm$0.873 & 16.0$\pm$1.28 & 24.4$\pm$1.22 & 11.1$\pm$1.22 & 5.52$\pm$1.28 & 1.53$\pm$0.144 & 1.04$\pm$0.139 & 0.318$\pm$0.0805 & 2.01$\pm$0.516 \\
  --Total & 36.8$\pm$8.10 & 6.31$\pm$6.31 & 163$\pm$8.14 & 192$\pm$7.70 & 57.7$\pm$8.37 & 38.6$\pm$8.14 & 1.18$\pm$0.0757 & 0.591$\pm$0.0776 & 0.226$\pm$0.0510 & 1.50$\pm$0.383 \\
  --Extended & 31.7$\pm$8.19 & 5.44$\pm$6.37 & 147$\pm$8.24 & 168$\pm$7.80 & 46.6$\pm$8.46 & 33.1$\pm$8.20 & 1.14$\pm$0.0833 & 0.542$\pm$0.0858 & 0.216$\pm$0.0571 & 1.41$\pm$0.433 \\
RXCJ1539.5-8335 & & & & & & & & & & \\
  --Centre & 3.86$\pm$0.965 & 1.52$\pm$0.968 & 17.1$\pm$1.03 & 21.0$\pm$1.05 & 11.1$\pm$1.00 & 6.41$\pm$1.03 & 1.22$\pm$0.0956 & 1.02$\pm$0.104 & 0.225$\pm$0.0579 & 1.74$\pm$0.319 \\
  --Total & 36.5$\pm$9.68 & 10.0$\pm$9.45 & 196$\pm$9.78 & 205$\pm$10.3 & 86.1$\pm$9.91 & 80.5$\pm$9.78 & 1.05$\pm$0.0742 & 0.852$\pm$0.0829 & 0.187$\pm$0.0503 & 1.07$\pm$0.179 \\
  --Extended & 32.7$\pm$9.72 & 8.48$\pm$9.50 & 178$\pm$9.83 & 184$\pm$10.3 & 75.0$\pm$9.96 & 74.1$\pm$9.71 & 1.03$\pm$0.0811 & 0.836$\pm$0.0905 & 0.183$\pm$0.0554 & 1.01$\pm$0.189 \\
RXCJ1558.3-1410 & & & & & & & & & & \\
  --Centre & 6.54$\pm$1.18 & 2.00$\pm$1.14 & 13.9$\pm$1.25 & 29.1$\pm$1.16 & 13.5$\pm$1.22 & 11.5$\pm$1.25 & 2.09$\pm$0.206 & 1.80$\pm$0.205 & 0.470$\pm$0.0945 & 1.18$\pm$0.166 \\
  --Total & 17.9$\pm$4.29 & 7.67$\pm$4.22 & 84.5$\pm$4.23 & 88.8$\pm$4.44 & 33.9$\pm$4.41 & 28.9$\pm$4.23 & 1.05$\pm$0.0743 & 0.743$\pm$0.0812 & 0.211$\pm$0.0518 & 1.17$\pm$0.229 \\
  --Extended & 11.3$\pm$4.44 & 5.67$\pm$4.37 & 70.6$\pm$4.41 & 59.7$\pm$4.59 & 20.4$\pm$4.57 & 17.4$\pm$4.50 & 0.846$\pm$0.0838 & 0.535$\pm$0.0968 & 0.160$\pm$0.0638 & 1.17$\pm$0.401 \\
RXCJ2014.8-2430 & & & & & & & & & & \\
  --Centre & 6.72$\pm$1.14 & 2.99$\pm$1.14 & 32.3$\pm$1.29 & 5.34$\pm$1.07 & 15.2$\pm$1.22 & 10.5$\pm$1.29 & 0.165$\pm$0.0337 & 0.795$\pm$0.0635 & 0.208$\pm$0.0363 & 1.46$\pm$0.215 \\
  --Total & 33.3$\pm$6.00 & 11.2$\pm$6.03 & 176$\pm$7.03 & 33.8$\pm$5.75 & 72.2$\pm$6.50 & 34.4$\pm$7.03 & 0.193$\pm$0.0336 & 0.607$\pm$0.0596 & 0.190$\pm$0.0350 & 2.10$\pm$0.469 \\
  --Extended & 26.6$\pm$6.11 & 8.18$\pm$6.14 & 143$\pm$7.15 & 28.5$\pm$5.85 & 57.0$\pm$6.61 & 23.9$\pm$6.30 & 0.199$\pm$0.0420 & 0.564$\pm$0.0696 & 0.186$\pm$0.0436 & 2.38$\pm$0.684 \\
RXCJ2101.8-2802 & & & & & & & & & & \\
  --Centre & 0.755$\pm$0.159 & 0.00$\pm$0.00 & 0.00$\pm$0.00 & 0.00$\pm$0.00 & 0.404$\pm$0.158 & 0.481$\pm$0.00 & 0.00$\pm$0.00 & 0.00$\pm$0.00 & 0.00$\pm$0.00 & 0.840$\pm$0.328 \\
  --Total & 4.74$\pm$1.68 & 0.00$\pm$0.00 & 41.3$\pm$1.86 & 4.95$\pm$1.59 & 7.67$\pm$1.69 & 6.89$\pm$1.86 & 0.120$\pm$0.0388 & 0.353$\pm$0.0628 & 0.115$\pm$0.0411 & 1.11$\pm$0.387 \\
  --Extended & 3.99$\pm$1.69 & 0.00$\pm$0.00 & 41.3$\pm$1.86 & 4.95$\pm$1.59 & 7.26$\pm$1.69 & 6.41$\pm$1.70 & 0.120$\pm$0.0388 & 0.331$\pm$0.0599 & 0.0966$\pm$0.0412 & 1.13$\pm$0.400 \\
RXCJ2129.6+0005 & & & & & & & & & & \\
  --Centre & 0.00$\pm$0.00 & 0.342$\pm$0.164 & 0.364$\pm$0.165 & 0.152$\pm$0.152 & 0.00$\pm$0.00 & 0.00$\pm$0.165 & 0.417$\pm$0.458 & 0.00$\pm$0.00 & 0.00$\pm$0.00 & 0.00$\pm$0.00 \\
  --Total & 2.46$\pm$1.24 & 2.80$\pm$1.25 & 20.2$\pm$1.31 & 16.5$\pm$1.24 & 0.744$\pm$0.744 & 5.43$\pm$1.31 & 0.819$\pm$0.0813 & 0.307$\pm$0.0774 & 0.122$\pm$0.0620 & 0.137$\pm$0.141 \\
  --Extended & 2.46$\pm$1.24 & 2.46$\pm$1.26 & 19.8$\pm$1.32 & 16.4$\pm$1.25 & 0.744$\pm$0.744 & 5.43$\pm$1.25 & 0.826$\pm$0.0837 & 0.312$\pm$0.0764 & 0.124$\pm$0.0632 & 0.137$\pm$0.140 \\
RXCJ2213.0-2753 & & & & & & & & & & \\
  --Centre & 3.32$\pm$0.762 & 0.515$\pm$0.515 & 11.3$\pm$0.788 & 12.0$\pm$0.722 & 9.39$\pm$0.751 & 7.85$\pm$0.788 & 1.07$\pm$0.0985 & 1.53$\pm$0.144 & 0.294$\pm$0.0708 & 1.20$\pm$0.153 \\
  --Total & 3.32$\pm$1.34 & 7.21$\pm$1.37 & 21.0$\pm$1.47 & 16.2$\pm$1.29 & 9.39$\pm$1.36 & 7.85$\pm$1.47 & 0.771$\pm$0.0819 & 0.822$\pm$0.111 & 0.158$\pm$0.0650 & 1.20$\pm$0.282 \\
  --Extended & 0.00$\pm$1.54 & 6.70$\pm$1.46 & 9.71$\pm$1.67 & 4.14$\pm$1.48 & 0.00$\pm$1.55 & 0.00$\pm$1.58 & 0.426$\pm$0.169 & 0.00$\pm$0.00 & 0.00$\pm$0.00 & 0.00$\pm$0.00 \\
RXJ0000.1+0816 & & & & & & & & & & \\
  --Centre & 2.05$\pm$0.883 & 0.00$\pm$0.00 & 9.67$\pm$0.919 & 19.2$\pm$0.961 & 8.85$\pm$0.885 & 7.23$\pm$0.919 & 1.99$\pm$0.213 & 1.66$\pm$0.206 & 0.212$\pm$0.0935 & 1.23$\pm$0.198 \\
  --Total & 10.6$\pm$3.73 & 0.249$\pm$0.249 & 46.4$\pm$3.95 & 85.8$\pm$4.29 & 32.4$\pm$3.89 & 26.1$\pm$3.95 & 1.85$\pm$0.182 & 1.26$\pm$0.160 & 0.229$\pm$0.0826 & 1.24$\pm$0.240 \\
  --Extended & 8.59$\pm$3.83 & 0.249$\pm$0.249 & 36.8$\pm$4.05 & 66.6$\pm$4.40 & 23.6$\pm$3.99 & 18.8$\pm$4.01 & 1.81$\pm$0.233 & 1.15$\pm$0.200 & 0.234$\pm$0.107 & 1.25$\pm$0.340 \\
\hline
\end{tabular}
%\label{tab:spec}
\end{center}
\end{sidewaystable}

\begin{sidewaystable}[p]
\begin{center}
\tiny
\centerline{\sc Table \ref{tab:sam}.}
\centerline{\sc The spectroscopic properties for each object in the sample}
\smallskip
\begin{tabular}{l c c c c c c c c c c c}
\hline
\smallskip
Cluster & [OI]$_{\lambda 6300}$ & [OI]$_{\lambda 6366}$ & H$\alpha$ & [NII]$_{\lambda 6583}$ & [SII]$_{\lambda 6716}$ & [SII]$_{\lambda 6731}$ & $\frac{[NII]_{\lambda 6583}}{H\alpha}$ & $\frac{[SII]_{\lambda 6716 + 6731}}{H\alpha}$ & $\frac{[OI]_{\lambda 6300}}{H\alpha}$ & $\frac{[SII]_{\lambda 6716}}{[SII]_{\lambda 6731}}$ \\
  --Region & \multicolumn{6}{c}{ 10$^{-16}$ erg s$^{-1}$ cm$^{-2}$} & & & & \\
\hline
RXJ0338+09 & & & & & & & & & & \\
  --Centre & 9.41$\pm$2.07 & 4.00$\pm$2.00 & 30.8$\pm$2.16 & 43.3$\pm$2.16 & 24.7$\pm$2.10 & 16.9$\pm$2.16 & 1.40$\pm$0.121 & 1.35$\pm$0.136 & 0.306$\pm$0.0706 & 1.46$\pm$0.224 \\
  --Total & 71.6$\pm$16.5 & 27.8$\pm$16.4 & 318$\pm$19.1 & 348$\pm$17.4 & 140$\pm$16.8 & 100.$\pm$19.1 & 1.09$\pm$0.0854 & 0.754$\pm$0.0918 & 0.225$\pm$0.0534 & 1.40$\pm$0.315 \\
  --Extended & 62.2$\pm$16.6 & 23.8$\pm$16.5 & 288$\pm$19.2 & 305$\pm$17.5 & 115$\pm$16.9 & 83.2$\pm$17.1 & 1.06$\pm$0.0935 & 0.690$\pm$0.0956 & 0.216$\pm$0.0595 & 1.38$\pm$0.350 \\
RXJ0352.9+1941 & & & & & & & & & & \\
  --Centre & 8.90$\pm$1.33 & 2.84$\pm$1.29 & 23.5$\pm$1.41 & 22.4$\pm$1.34 & 17.7$\pm$1.42 & 10.9$\pm$1.41 & 0.952$\pm$0.0808 & 1.22$\pm$0.112 & 0.379$\pm$0.0612 & 1.63$\pm$0.249 \\
  --Total & 52.4$\pm$8.91 & 16.7$\pm$8.50 & 201$\pm$10.0 & 151$\pm$9.07 & 91.1$\pm$9.11 & 64.9$\pm$10.0 & 0.753$\pm$0.0588 & 0.777$\pm$0.0779 & 0.261$\pm$0.0463 & 1.40$\pm$0.259 \\
  --Extended & 43.5$\pm$9.01 & 13.8$\pm$8.60 & 177$\pm$10.1 & 129$\pm$9.17 & 73.4$\pm$9.22 & 54.0$\pm$8.54 & 0.727$\pm$0.0664 & 0.719$\pm$0.0820 & 0.246$\pm$0.0528 & 1.36$\pm$0.274 \\
RXJ0439.0+0520 & & & & & & & & & & \\
  --Centre & 0.00$\pm$0.00 & 0.874$\pm$0.407 & 5.53$\pm$0.443 & 10.2$\pm$0.407 & 4.23$\pm$0.423 & 5.00$\pm$0.443 & 1.84$\pm$0.164 & 1.67$\pm$0.173 & 0.00$\pm$0.00 & 0.846$\pm$0.113 \\
  --Total & 0.00$\pm$0.00 & 3.16$\pm$3.16 & 40.9$\pm$3.68 & 38.0$\pm$3.42 & 20.6$\pm$3.49 & 16.7$\pm$3.68 & 0.931$\pm$0.118 & 0.911$\pm$0.149 & 0.00$\pm$0.00 & 1.23$\pm$0.342 \\
  --Extended & 0.00$\pm$0.00 & 2.28$\pm$3.18 & 35.3$\pm$3.71 & 27.9$\pm$3.45 & 16.3$\pm$3.52 & 11.7$\pm$3.45 & 0.789$\pm$0.128 & 0.793$\pm$0.162 & 0.00$\pm$0.00 & 1.39$\pm$0.509 \\
RXJ0747-19 & & & & & & & & & & \\
  --Centre & 18.3$\pm$3.84 & 6.71$\pm$3.72 & 71.1$\pm$4.27 & 77.1$\pm$3.86 & 43.2$\pm$3.89 & 36.4$\pm$4.27 & 1.08$\pm$0.0847 & 1.12$\pm$0.105 & 0.257$\pm$0.0562 & 1.19$\pm$0.175 \\
  --Total & 70.6$\pm$15.5 & 24.6$\pm$15.5 & 278$\pm$16.7 & 325$\pm$16.2 & 168$\pm$16.8 & 119$\pm$16.7 & 1.17$\pm$0.0913 & 1.03$\pm$0.105 & 0.254$\pm$0.0579 & 1.40$\pm$0.241 \\
  --Extended & 52.3$\pm$16.0 & 17.9$\pm$15.9 & 207$\pm$17.2 & 248$\pm$16.7 & 124$\pm$17.2 & 82.9$\pm$16.0 & 1.20$\pm$0.128 & 1.00$\pm$0.141 & 0.253$\pm$0.0802 & 1.50$\pm$0.357 \\
RXJ0821+07 & & & & & & & & & & \\
  --Centre & 0.631$\pm$0.281 & 0.00$\pm$0.00 & 6.28$\pm$0.314 & 3.62$\pm$0.290 & 1.16$\pm$0.284 & 0.0551$\pm$0.314 & 0.577$\pm$0.0544 & 0.193$\pm$0.0681 & 0.100$\pm$0.0450 & 21.0$\pm$120 \\
  --Total & 12.0$\pm$5.41 & 1.29$\pm$1.29 & 124$\pm$6.19 & 101$\pm$5.55 & 28.6$\pm$5.44 & 0.440$\pm$6.19 & 0.816$\pm$0.0607 & 0.235$\pm$0.0676 & 0.0971$\pm$0.0440 & 65.1$\pm$914 \\
  --Extended & 11.4$\pm$5.42 & 1.29$\pm$1.29 & 117$\pm$6.19 & 97.4$\pm$5.56 & 27.5$\pm$5.45 & 0.385$\pm$0.444 & 0.829$\pm$0.0645 & 0.237$\pm$0.0482 & 0.0970$\pm$0.0464 & 71.4$\pm$83.4 \\
RXJ1651.1+0459 & & & & & & & & & & \\
  --Centre & 1.52$\pm$0.326 & 0.623$\pm$0.321 & 7.43$\pm$0.334 & 1.62$\pm$0.308 & 5.51$\pm$0.358 & 2.16$\pm$0.334 & 0.218$\pm$0.0426 & 1.03$\pm$0.0806 & 0.204$\pm$0.0449 & 2.55$\pm$0.427 \\
  --Total & 4.46$\pm$1.47 & 2.44$\pm$1.47 & 38.4$\pm$1.53 & 3.94$\pm$1.40 & 23.0$\pm$1.61 & 9.25$\pm$1.53 & 0.103$\pm$0.0367 & 0.841$\pm$0.0671 & 0.116$\pm$0.0387 & 2.49$\pm$0.449 \\
  --Extended & 2.94$\pm$1.51 & 1.82$\pm$1.50 & 30.9$\pm$1.57 & 2.32$\pm$1.43 & 17.5$\pm$1.65 & 7.08$\pm$1.51 & 0.0751$\pm$0.0465 & 0.796$\pm$0.0830 & 0.0951$\pm$0.0490 & 2.47$\pm$0.578 \\
S555 & & & & & & & & & & \\
  --Centre & 3.77$\pm$1.09 & 1.20$\pm$1.09 & 15.8$\pm$1.11 & 31.9$\pm$10.7 & 15.4$\pm$1.23 & 13.0$\pm$1.11 & 2.02$\pm$0.691 & 1.80$\pm$0.164 & 0.239$\pm$0.0713 & 1.18$\pm$0.137 \\
  --Total & 17.1$\pm$7.71 & 7.69$\pm$7.57 & 106$\pm$7.95 & 226$\pm$64.5 & 94.6$\pm$8.04 & 77.2$\pm$7.95 & 2.13$\pm$0.629 & 1.62$\pm$0.162 & 0.162$\pm$0.0737 & 1.23$\pm$0.164 \\
  --Extended & 13.4$\pm$7.79 & 6.49$\pm$7.65 & 90.2$\pm$8.03 & 194$\pm$65.4 & 79.3$\pm$8.14 & 64.2$\pm$8.19 & 2.15$\pm$0.749 & 1.59$\pm$0.191 & 0.148$\pm$0.0873 & 1.24$\pm$0.202 \\
S780 & & & & & & & & & & \\
  --Centre & 4.48$\pm$0.874 & 1.95$\pm$0.866 & 17.9$\pm$0.895 & 17.3$\pm$0.863 & 8.39$\pm$0.923 & 10.4$\pm$0.895 & 0.964$\pm$0.0681 & 1.05$\pm$0.0889 & 0.250$\pm$0.0504 & 0.806$\pm$0.113 \\
  --Total & 21.6$\pm$4.32 & 9.09$\pm$4.23 & 94.8$\pm$4.74 & 101$\pm$4.03 & 32.4$\pm$4.37 & 37.2$\pm$4.74 & 1.06$\pm$0.0680 & 0.734$\pm$0.0773 & 0.228$\pm$0.0470 & 0.870$\pm$0.162 \\
  --Extended & 17.1$\pm$4.40 & 7.15$\pm$4.32 & 76.9$\pm$4.82 & 83.4$\pm$4.12 & 24.0$\pm$4.46 & 26.8$\pm$4.56 & 1.09$\pm$0.0867 & 0.660$\pm$0.0928 & 0.222$\pm$0.0590 & 0.895$\pm$0.226 \\
S805 & & & & & & & & & & \\
  --Centre & 1.22$\pm$1.22 & 0.00$\pm$0.00 & 1.51$\pm$1.40 & 23.3$\pm$1.51 & 7.24$\pm$1.45 & 7.40$\pm$1.40 & 15.5$\pm$14.4 & 9.72$\pm$9.14 & 0.813$\pm$1.11 & 0.978$\pm$0.269 \\
  --Total & 4.85$\pm$4.85 & 0.00$\pm$0.00 & 16.0$\pm$6.94 & 96.9$\pm$6.79 & 24.3$\pm$7.05 & 24.6$\pm$6.94 & 6.08$\pm$2.68 & 3.06$\pm$1.47 & 0.304$\pm$0.331 & 0.990$\pm$0.401 \\
  --Extended & 3.62$\pm$5.00 & 0.00$\pm$0.00 & 14.5$\pm$7.08 & 73.6$\pm$6.95 & 17.1$\pm$7.20 & 17.2$\pm$7.15 & 5.10$\pm$2.54 & 2.37$\pm$1.36 & 0.251$\pm$0.367 & 0.995$\pm$0.589 \\
S851 & & & & & & & & & & \\
  --Centre & 12.2$\pm$4.81 & 0.0469$\pm$0.0469 & 29.0$\pm$4.94 & 129$\pm$5.14 & 41.4$\pm$4.97 & 24.9$\pm$4.94 & 4.42$\pm$0.773 & 2.28$\pm$0.457 & 0.419$\pm$0.180 & 1.66$\pm$0.386 \\
  --Total & 95.1$\pm$36.1 & 0.0469$\pm$0.00 & 132$\pm$36.3 & 905$\pm$36.2 & 294$\pm$38.2 & 196$\pm$36.3 & 6.86$\pm$1.91 & 3.71$\pm$1.10 & 0.721$\pm$0.338 & 1.50$\pm$0.339 \\
  --Extended & 82.9$\pm$36.5 & 0.00$\pm$0.0469 & 103$\pm$36.6 & 777$\pm$36.6 & 253$\pm$38.5 & 171$\pm$37.6 & 7.55$\pm$2.71 & 4.12$\pm$1.56 & 0.806$\pm$0.456 & 1.48$\pm$0.395 \\
Z3179 & & & & & & & & & & \\
  --Centre & 1.61$\pm$0.490 & 0.927$\pm$0.482 & 3.16$\pm$0.490 & 11.6$\pm$0.466 & 3.62$\pm$0.489 & 3.32$\pm$0.490 & 3.68$\pm$0.589 & 2.19$\pm$0.404 & 0.508$\pm$0.174 & 1.09$\pm$0.218 \\
  --Total & 2.76$\pm$1.06 & 0.927$\pm$0.00 & 6.44$\pm$1.10 & 24.6$\pm$1.11 & 7.33$\pm$1.06 & 6.42$\pm$1.10 & 3.82$\pm$0.672 & 2.13$\pm$0.433 & 0.429$\pm$0.180 & 1.14$\pm$0.256 \\
  --Extended & 1.16$\pm$1.17 & 0.00$\pm$0.482 & 3.28$\pm$1.20 & 12.9$\pm$1.20 & 3.71$\pm$1.17 & 3.10$\pm$1.20 & 3.95$\pm$1.49 & 2.08$\pm$0.917 & 0.353$\pm$0.380 & 1.20$\pm$0.598 \\
Z348 & & & & & & & & & & \\
  --Centre & 10.5$\pm$1.26 & 3.18$\pm$1.23 & 36.7$\pm$1.47 & 13.8$\pm$1.24 & 14.8$\pm$1.33 & 10.1$\pm$1.47 & 0.376$\pm$0.0370 & 0.677$\pm$0.0604 & 0.286$\pm$0.0362 & 1.46$\pm$0.250 \\
  --Total & 47.6$\pm$5.24 & 13.6$\pm$5.24 & 156$\pm$6.25 & 57.8$\pm$5.20 & 58.9$\pm$5.30 & 43.5$\pm$6.25 & 0.370$\pm$0.0364 & 0.655$\pm$0.0586 & 0.305$\pm$0.0356 & 1.35$\pm$0.230 \\
  --Extended & 37.1$\pm$5.39 & 10.4$\pm$5.38 & 120$\pm$6.42 & 44.0$\pm$5.35 & 44.2$\pm$5.47 & 33.4$\pm$5.36 & 0.368$\pm$0.0489 & 0.648$\pm$0.0729 & 0.310$\pm$0.0480 & 1.32$\pm$0.268 \\
\hline
\end{tabular}
%\label{tab:s}
\end{center}
\end{sidewaystable}

\end{appendix}
